# Supplementary material for: Fundamental limits on taming infectious disease epidemics
Source: arXiv:2509.11764 source file (2025-09-15)
Supplement: Supplementary file 1 [file supp.pdf]

# Supplementary information for Fundamental limits on taming infectious disease epidemics

Giovanni Pugliese Carratelli<sup>1</sup>, Xiaodong Cheng<sup>2</sup>, Kris V. Parag<sup>3</sup>,  
Ioannis Lestas<sup>1</sup>

<sup>1</sup>Department of Engineering, University of Cambridge, Trumpington  
street, Cambridge, CB1 PZ, United Kingdom.

<sup>2</sup>Biometris group, Wageningen University, Radix building 107,  
Droevendaalsesteeg 1, Wageningen, 6708 PB, The Netherlands.

<sup>3</sup>MRC Centre for Global Infectious Disease Analysis, Imperial College  
London, 90 Wood Lane, London, W12 0BZ, United Kingdom.

Contributing authors: [gp459@cam.ac.uk](mailto:gp459@cam.ac.uk); [xiaodong.cheng@wur.nl](mailto:xiaodong.cheng@wur.nl);  
[k.parag@imperial.ac.uk](mailto:k.parag@imperial.ac.uk); [icl20@cam.ac.uk](mailto:icl20@cam.ac.uk);

## 1 Introduction

Finding optimal policies to control an epidemic is a problem of major significance. Policies have to trade-off over an indefinite amount of time the socio-economic costs of the interventions and the well-being of society. Uncertainty surrounding the transmission mechanism and the impact of the interventions further complicate the analysis. The policies depend on the choice of the considered costs that also are difficult to quantify, and lead to different optimal policies.

Many studies focus on the ad-hoc selection of the optimal policies via approximate deterministic models [1–4], including the time sensitivity of their implementation [5–7] or cost-benefit analysis studies [8–10]. Stochastic models that incorporate the randomness of the spread are predominately used in simulation studies to evaluate intuition based policies [11–14].

Results on general features of optimal policies in stochastic epidemic models and ones that establish the dependence of optimal policies on cost functions are, however, limited despite their practical significance.

In this paper we explicitly address these challenges by modelling epidemics as controlled continuous time Markov Jump Processes (MJPs) where we identify fundamental features in corresponding optimal policies.

Our contribution is summarised below:

- We consider stochastic models for epidemics modelled as a continuous time MJP with a controlled transmission rate. Throughout the paper we show that even when arbitrary feedback policies are considered, surprisingly negative feedback with respect to the number of individuals infected is not effective in taming the epidemic for broad classes of cost functions. In particular, the result is shown for costs that depend linearly with the number of infected individuals but can otherwise depend nonlinearly with the mitigation measures.
- This result is shown first analytically for the Susceptible Infected (SI) model. We also develop computational tools for evaluating the optimal policies for general classes of stochastic epidemic models with arbitrary number of states/compartments. We explicitly compute optimal policies for the stochastic Susceptible Infected Removed (SIR) and Susceptible Exposed Infected Removed (SEIR) models and we observe an analogous behaviour also in these models. In particular, the optimal policies do not involve negative feedback with respect to the number of infected. Feedback with respect to the number of susceptible is observed in this case, which is associated with herd immunity effects that generally occur at slower timescales.
- We also further validate the above observations, by quantifying the optimal policies in corresponding deterministic models as well as more complex models with random infection outcomes where analogous properties are observed.

This document is organised as follows. We introduce in Section 2 the notation and the epidemic models that will be considered and in Section 3 we define the problems we seek to address. Our main results are stated in Section 4. In Section 5 we derive our results via a series of intermediate Lemmas. Appendix A includes the proofs of these Lemmas. Additional figures and discussion are provided in Appendix B.

## 2 Preliminaries

In Section 2.1 we introduce the notation and the symbols used in the manuscript. In Section 2.2 we present the epidemic models and the mathematical quantities that will be considered in the study. In particular, we introduce the stochastic Susceptible Infected Removed (SIR) epidemic in Section 2.3. We then consider the simplified Susceptible Infected (SI) epidemic and the more complex Susceptible Exposed Infected Removed (SEIR) epidemic in Section 2.4 and Section 2.5 respectively.

## 2.1 Notation

The following list introduces various symbols used in the manuscript

|                           |                                                                                                                                                                                                     |
|---------------------------|-----------------------------------------------------------------------------------------------------------------------------------------------------------------------------------------------------|
| $\mathbb{E}[\cdot]$       | Expectation operator                                                                                                                                                                                |
| $\Delta_i^1[f]$           | Forward one step operator applied to function $f : \cdot \times \mathbb{Z}_{\geq} \rightarrow \cdot$ i.e. for $i \in \mathbb{Z}_{\geq}$ , $\Delta_i^1[f(\cdot, i)] = f(\cdot, i+1) - f(\cdot, i)$ . |
| $\Delta_i^p[f]$           | Forward $p$ step operator such that if $p > 1$ , $p \in \mathbb{Z}_{>}$ , $\Delta_i^p[f(\cdot, i)] = \Delta_i^1[\Delta_i^{p-1}[f(\cdot, i)]]$                                                       |
| $\inf$                    | The infimum operator                                                                                                                                                                                |
| $\mathbb{E}_{\pi}[\cdot]$ | Expectation operator with respect to the distribution $\pi$                                                                                                                                         |
| $\mathbb{R}_{>}$          | Set of positive real numbers $\{x \in \mathbb{R} : x > 0\}$                                                                                                                                         |
| $\mathbb{R}_{\geq}$       | Set of non-negative real numbers $\{x \in \mathbb{R} : x \geq 0\}$                                                                                                                                  |
| $\mathbb{Z}_{>}$          | Set of positive integers $\{1, 2, 3, \dots\}$                                                                                                                                                       |
| $\mathbb{Z}_{\geq}$       | Set of non-negative integers $\{0, 1, 2, 3, \dots\}$                                                                                                                                                |
| $\mathcal{B}(p, n)$       | Binomial probability distribution, with parameters $0 < p \leq 1$ and $n \in \mathbb{Z}_{\geq}$                                                                                                     |
| $\mathcal{U}(a, b)$       | Uniform probability distribution on the support $a, b$ with $a < b$                                                                                                                                 |

## 2.2 Mathematical preliminaries

We consider Markov Jump Process (MJP) versions of the SIR, SEIR and SI transmission models for an epidemic. The state of the system is the number of individuals in the considered categories which evolves via infection, exposure and recovery events occurring at certain rates. These events take place at random times that depend upon the state of the system [15] and its parameters and are summarised in Table S1. In

| ID | Event          | Transition                                  | Rate                          |
|----|----------------|---------------------------------------------|-------------------------------|
| 1a | SEIR Exposure  | $(S, E, I, R) \rightarrow (S-1, E+1, I, R)$ | $\mu \frac{SI \cdot h(u)}{N}$ |
| 1b | SEIR Infection | $(S, E, I, R) \rightarrow (S, E-1, I+1, R)$ | $\epsilon E$                  |
| 1c | SEIR Recovery  | $(S, E, I, R) \rightarrow (S, E, I-1, R+1)$ | $\gamma I$                    |
| 2a | SIR Infection  | $(S, I, R) \rightarrow (S-1, I+1, R)$       | $\mu \frac{SI \cdot h(u)}{N}$ |
| 2b | SIR Recovery   | $(S, I, R) \rightarrow (S, I-1, R+1)$       | $\gamma I$                    |
| 3a | SI Infection   | $I \rightarrow I+1$                         | $\mu \beta_f(I, u)$           |
| 3b | SI Recovery    | $I \rightarrow I-1$                         | $\gamma I$                    |

**Table S1:** Events associated with the Susceptible Exposed Infected Removed (SEIR), Susceptible Infected Removed (SIR) and Susceptible Infected (SI) epidemics

particular, the systems we will be considering are birth-death like process that can be defined via a corresponding Master equation [16? , 17] (also known as the Kolmogorov Equation). This is a partial difference equation for the probability at time  $t$  that the number of individuals in each category takes prescribed values [15]. The

Master equation for the considered epidemics is stated in the following sections, but before that we introduce the variables describing the systems and their physical interpretation. More precisely, we consider a constant population of  $N \in \mathbb{Z}_{>}$  individuals and the integer valued random variables  $S(t), E(t), I(t)$  and  $R(t)$ , each defined on the support  $\mathbb{S} = \{0, 1, \dots, N\}$ .  $S(t), E(t), I(t)$  and  $R(t)$  denote respectively the number of Susceptible, Exposed, Infected and Recovered individuals at time  $t$ . We denote the infection and exposure prevalence with  $I(t)/N$  and  $E(t)/N$  respectively, and we denote the incidence of the disease with  $S(t)/N$ .

The rate at which infected individuals recover corresponds to events 1c, 2b, 3b in Table S1, in the SEIR, SIR and SI epidemics, respectively, and is given by  $\gamma I(t)$  where  $\gamma \in \mathbb{R}_{>}$ .

For each exposure event of the SEIR epidemic and each infection event of the SIR epidemic, corresponding respectively to events 1a and 2a in Table S1, a single individual transitions from the Susceptible to the Infected or Exposed category. These events occur at a rate of  $\mu S(t)I(t)/Nh(u)$  where  $\mu \in \mathbb{R}_{>}$  is the transmission parameter. The infection rate of the SEIR epidemic, corresponding to event 1b in Table S1 is  $\epsilon E$ , with  $\epsilon \in \mathbb{R}_{>}$ .

The infection events of the SI epidemic, corresponding to event 3a of Table S1, occur at a rate  $\beta_f(I, u)$  defined in (3) of Section 2.4. We highlight that due to the proportional nature of the infection rate with respect to  $I$  the systems have an absorbing state at  $I = 0$ .

The variable  $u \in \mathcal{U}$  denotes a transmission mitigation measure within the set  $\mathcal{U} = \{u_1, u_2, \dots, u_{N_u}\}$  of cardinality  $N_u \in \mathbb{Z}_{>}$  i.e. the set of measures that can be implemented to tame the disease transmission. For simplicity we assign each measure in the set  $\mathcal{U}$  to be within  $[0, 1]$  and we denote with the function  $h(u) : \mathcal{U} \rightarrow [0, 1]$  the transmission rate reduction for each mitigation measure  $u$ . High values of  $u$  are associated with restrictive interventions and low values of  $u$  are associated with moderately restrictive interventions. This mathematical formulation is common in the literature as measures  $u$  can have different effects on different epidemics but in the following sections we address optimal control problems where we optimise over all possible values of  $\mathcal{U}$  and our results are independent of the set  $\mathcal{U}$ , its cardinality and  $h(u)$ .

We consider for notational purposes and to simplify the interpretation of the results, the following assumption

**Assumption 1** *The function  $h(u) : \mathcal{U} \rightarrow [0, 1]$  is a non-increasing function.*

Assumption 1 formalises that increasing values of  $u$ , that are associated with increasingly restrictive mitigation measures, reduce  $h(u)$  and thus reduce the transmission of the disease. This assumption is without any loss of generality as will be discussed after the results are presented and with some examples in Section B.1.

We finally define the controlled reproduction number<sup>1</sup>

$$\mathcal{R} = \mathcal{R}_0 h(u), \mathcal{R}_0 = \mu/\gamma \quad (1)$$

where  $\mathcal{R}_0$  is the basic reproduction number, *i.e.* the expected number of new infections due to a single infection [19]. The controlled reproduction number  $\mathcal{R}$ , corresponds to  $\mathcal{R}_0$  when no interventions are used. Also, high values of  $u$  associated with restrictive interventions correspond to low values of  $\mathcal{R}$  and low values of  $u$ , associated with more moderate interventions, correspond to higher values of  $\mathcal{R}$ . It should be noted that  $\mathcal{R}$  is a convenient notion linking the parameters of the disease transmission to the possibility of major epidemics [20]. Values of  $\mathcal{R} > 1$  lead to a major epidemic characterised by exponential growth. Values of  $\mathcal{R} \leq 1$  are linked with a decrease of disease prevalence.

### 2.3 Stochastic Susceptible Infected Removed (SIR) model

The state of the SIR epidemic is the number of susceptible, infectious and removed individuals of a population. The state evolves via infection and recovery events occurring at the rates defined in rows 2a and 2b of Table S1. We consider a constant population of  $N \in \mathbb{Z}_>$  individuals and hence we have  $S(t) + I(t) + R(t) = N$ . Therefore  $R(t) = N - S(t) - I(t)$  and without any loss of generality we consider only the random variables  $S(t)$  and  $I(t)$ . For each  $s, i \in \mathbb{S} \times \mathbb{S}$  we denote by  $\mathbb{P}(s, i, t)$  the probability that at time  $t$  we have  $S(t) = s$  and  $I(t) = i$ . The considered MJP satisfies the following Kolmogorov Equation

$$\begin{aligned} \frac{\partial \mathbb{P}(s, i, t)}{\partial t} = & \gamma[(i+1)\mathbb{P}(s, i+1, t) - i\mathbb{P}(s, i, t)] \\ & + \frac{\mu h(u)}{N}[(s+1)(i-1)\mathbb{P}(s+1, i-1, t) - si\mathbb{P}(s, i, t)] \end{aligned} \quad (2)$$

### 2.4 Stochastic Susceptible Infected (SI) model

The SI model [21] is a simplified version of the SIR model, where it is assumed that there are few individuals in the recovered category. The state of the system is the number of susceptible and infectious individuals. The system evolves via the events 3a and 3b of Table S1 where  $\beta_f$  is defined below. This is a well suited model for diseases characterised by weak levels of immunity after a recovery or at the initial stages of an epidemic when the number of infected is small with respect to the size of the population, *i.e.* when few recoveries have taken place  $R(t) \ll N$ . In this model we also consider a constant population of  $N$  individuals and  $R(t) = 0$ . It follows that  $S(t) + I(t) = N, \forall t$  and hence  $S(t) = N - I(t)$ . We reformulate the system satisfying

---

<sup>1</sup> $\mathcal{R}$  is smaller than or equal to  $\mathcal{R}_0$  [18], irrespectively of the incidence of the disease  $S/N$ . This is accounted by the *effective reproduction number*  $\mathcal{R}_e = \mathcal{R}_0 h(u) \frac{S}{N}$ , *i.e.* a state and time dependant quantity. Note that for  $S < N$  it follows that  $\mathcal{R}_e \leq \mathcal{R}, \forall u \in \mathcal{U}$  and without any loss of generality we use  $\mathcal{R}$  over  $\mathcal{R}_e$  to simplify the interpretation of the results.

(2) as a function of  $I(t)$  with the following transmission rate

$$\beta_f(i, u) = \frac{i}{N}(N - i)h(u) \quad (3)$$

For each  $i \in \mathbb{S}$  we denote with  $\mathbb{P}(i, t)$  the probability that at time  $t$  we have  $I(t) = i$ . The Kolmogorov Equation for the considered system is

$$\begin{aligned} \frac{\partial \mathbb{P}(i, t)}{\partial t} = & \mu [\beta_f(i - 1, u)\mathbb{P}(i - 1, t) - \beta_f(i, u)\mathbb{P}(i, t)] \\ & + \gamma[(i + 1)\mathbb{P}(i + 1, t) - i\mathbb{P}(i, t)] \end{aligned} \quad (4)$$

## 2.5 Stochastic Susceptible Exposed Infected Removed (SEIR) model

The SEIR epidemic [22] is a more detailed model than the SIR transmission model and incorporates the Exposed category that quantifies the number of individuals that come into contact with infectious individuals. Individuals that have been exposed to the disease do not show symptoms and spend a random amount of time in this category that effectively corresponds to a random delay before becoming infectious.

The state of the system is the number of susceptible, exposed, infectious and removed individuals of a constant population of  $N$  individuals. The state evolves via exposure, infection and recovery events defined in row 1a, 1b, 1c of Table S1. It follows that  $S(t) + E(t) + I(t) + R(t) = N$  and hence  $R(t) = N - S(t) - E(t) - I(t)$ . Without any loss of generality we therefore consider only the random variables  $S(t)$ ,  $E(t)$  and  $I(t)$ .

For each  $s, e, i \in \mathbb{S} \times \mathbb{S} \times \mathbb{S}$  we denote by  $\mathbb{P}(s, e, i, t)$  the probability that at time  $t$  we have  $S(t) = s$ ,  $E(t) = e$  and  $I(t) = i$ . The Kolmogorov equation for the systems is

$$\begin{aligned} \frac{\partial \mathbb{P}(s, e, i, t)}{\partial t} = & \gamma[(i + 1)\mathbb{P}(s, e, i + 1, t) - i\mathbb{P}(s, e, i, t)] \\ & + \frac{\mu h(u)}{N}[(s + 1)(i - 1)\mathbb{P}(s + 1, e - 1, i, t) - si\mathbb{P}(s, e, i, t)] \\ & + \epsilon[(e + 1)\mathbb{P}(s, e + 1, i - 1, t) - e\mathbb{P}(s, e, i, t)] \end{aligned} \quad (5)$$

## 3 Problem formulation and considered costs

We consider the problem of finding an optimal feedback disease mitigation policy. We formulate a stochastic optimal control problem for the SIR epidemic in Section 3.1 and outline the considered costs in Section 3.2. We then introduce equivalent problems for the SI epidemic and the more complex SEIR epidemic in Section 3.3 and Section 3.4 respectively.

In the considered problem we seek to minimise social costs due to the presence of  $i$  infected and due to the adoption of the transmission mitigation measure  $u$ . In particular, we minimise the total expected costs in continuous time over an infinite

horizon, where the stage cost per unit of time is  $g_c(i, u) : \mathbb{S} \times \mathcal{U} \rightarrow \mathbb{R}_{\geq}$ . The function  $g_c$ , discussed in more detail in Section 3.2, is the cost of applying the mitigation measure  $u$  with  $i$  infected individuals.

We consider deterministic feedback policies that are a function of the current state of the process. This is without loss of generality due to the Markov nature of the system, *i.e.* state feedback policies would be optimal even if the feedback policy was allowed to depend on the history of the process [23],[24]. Later on we will discuss how our results relating to the properties of the optimal policies we derive hold also when imperfect state information is present. We consider without any loss of generality only time invariant feedback laws since it can be shown that the policies for an infinite horizon problem are independent of time [24, 25].

### 3.1 Problem formulation for the Susceptible Infected Removed (SIR) epidemic

A particular policy for the SIR epidemic satisfying (2) is denoted by  $u(s, i)$ ,  $u : \mathbb{S} \times \mathbb{S} \rightarrow \mathcal{U}$ . With  $\mathcal{F}$  we denote the set of time invariant state feedback policies, *i.e.* the set of functions  $u$  which for each value of the state give an element in  $\mathcal{U}$ .

**Problem 1** *Consider the system in (2) and the stage cost  $g_c(i, u) : \mathbb{S} \times \mathcal{U} \rightarrow \mathbb{R}_{\geq}$ . We consider the following problem*

$$J^c(s_0, i_0) = \min_{u \in \mathcal{F}} J_u^c(s_0, i_0) \quad (6)$$

where  $\mathcal{F}$  denotes the set of state feedback time invariant control policies  $u(s, i)$ ,  $u : \mathbb{S} \times \mathbb{S} \rightarrow \mathcal{U}$ .  $J_u^c(s_0, i_0)$ , defined in (7), is the cost associated with the evolution of the MJP in (2) from the initial condition  $\{s_0, i_0\}$  under the time invariant state feedback policy  $u$ .

$$J_u^c(s_0, i_0) = \lim_{T_{N_t} \rightarrow \infty} \mathbb{E} \left[ \int_0^{T_{N_t}} g_c(i(t), u) dt \middle| S(0) = s_0, I(0) = i_0 \right] \quad (7)$$

As previously discussed the considered continuous time process has an absorbing state and terminates in finite time. It can be shown that the considered continuous time optimal control problem can be transformed to that of an appropriately constructed discrete time Markov Decision Process (MDP). This equivalent formulation is presented in Section 5.1 and it is adopted for the derivation of the results.

The solution of Problem 1 corresponds to finding an optimal policy  $u^*(s, i)$  that minimises a socio-economic cost  $g_c(i, u)$  related to an epidemic. In particular, we associate for each infected individual a cost that society has to incur and a costs for interventions that reduce the transmission of the disease.

### 3.2 Considered costs

In this section we describe the class of costs functions that will be considered. In particular, we consider costs associated with targeted interventions, *i.e.* where a single individual may need medical treatment, isolation and quarantine, and the population wide costs of adopting transmission mitigation measures thus incurring in high socio/economic costs. The transmission mitigation interventions  $u$  encompass a broad

class of measures including social distancing, medical isolation and quarantine as well as business closure or stay at home policies which apply to the population as a whole. Specifically, we consider cost functions  $g_c$  of the form

$$g_c(i, u) = c_1 + c_2 iz(u) + c_3 i + c_4 Nu \quad (8)$$

where  $z(u) : \mathcal{U} \rightarrow \mathbb{R}_{\geq}$  is an arbitrary function with non-negative values and  $c_1, c_2, c_3, c_4$  are constants in  $\mathbb{R}_{>}$ .

We first consider cost functions  $g_c$  as in (8) without population wide costs *i.e.*  $c_4 = 0$

$$g_c(i, u) = c_1 + c_2 iz(u) + c_3 i \quad (9)$$

The stage cost in (9) is the sum of three terms relating to the state of the epidemic, the targeted mitigation measures and constant costs. The term  $c_1$  is a fixed cost to be accounted for regardless of the number of infected or the adopted mitigation measures. The proportionality between  $i$  and  $z(u)$  suggests that cost  $c_2 z(u)$  is incurred for each individual infected when mitigation measure  $u$  is used. The term  $c_3 i$  relates to the sole presence of infected individuals and is linked to fatalities and hospitalisations when the latter are below their capacity. The parameter  $c_3$  depends for example upon the infected to fatality ratio or the infected to hospitalisation ratio. Note that without loss of generality the cost in (9) can be rescaled with respect to the hospitalisation cost parameter  $c_3$ . We define the ratio

$$\zeta = c_2/c_3 \quad (10)$$

that is the ratio of marginal cost  $c_2$  of using mitigation measures, with respect to the marginal costs for hospitalisations, diagnosis and fatalities  $c_3$ . Costs of the form in (9) apply for example to influenza like epidemics [26] or more broadly to regimes where the efforts to control the epidemics through isolation of infected are applicable and exclude non-selective policies where the entire population is subject to restrictions such as lock down.

In our analysis we will also consider cost functions that are relevant when non selective policies are applied to the whole population, *i.e.*  $c_4 \neq 0$ , as defined below

$$g_c(i, u) = c_1 + c_2 iu + c_3 i + c_4 Nu \quad (11)$$

The terms  $c_1$ ,  $c_2 iu$  and  $c_3 i$  are analogous to those in (9) with  $z(u) = u$  and similarly to (9) the cost parameter  $c_3$  depends on the infected to fatality ratio and the infected to hospitalisation ratio. The cost function (11) has additionally the term  $c_4 Nu$  where  $c_4$  is the cost for each individual associated with interventions that affect the entire population and thus scale with the population size  $N$ . These interventions include the adoption of masks or area stay-at-home and business closures policies for the population. It should also be noted that costs of the form  $g_c(i, u) = c_1 + c_2 iu + c_3 i + c_4(N - i)u$ , that frequently appear in the literature [10, 27], can be reformulated as in (11).



### 3.3 Problem formulation for the Susceptible Infected (SI) epidemic

An optimal control problem analogous to that in Problem 1 for the continuous time SI model defined in (4) is given in Problem 2.

**Problem 2** Consider the system in (4) and the stage cost  $g_c(i, u) : \mathbb{S} \times \mathcal{U} \rightarrow \mathbb{R}_{\geq}$ . We consider the following problem

$$J^c(i_0) = \min_{u \in \mathcal{F}} J_u^c(i_0) \quad (12)$$

where  $\mathcal{F}$  denotes the set of state feedback time invariant control policies  $u(i)$ ,  $u : \mathbb{S} \rightarrow \mathcal{U}$ .  $J_u^c(i_0)$ , defined in (13), is the cost associated with the evolution of the MJP in (4) from the initial condition  $i_0$  under a time invariant state feedback policy  $u$ .

$$J_u^c(i_0) = \lim_{T_{N_t} \rightarrow \infty} \mathbb{E} \left[ \int_0^{T_{N_t}} g_c(i(t), u) dt \middle| I(0) = i_0 \right] \quad (13)$$

### 3.4 Problem formulation for the Susceptible Exposed Infected Removed (SEIR) epidemic

A corresponding optimal control problem for the SEIR epidemic defined in (5) is given below.

**Problem 3** Consider the system in (5) and the stage cost  $g_c(i, u) : \mathbb{S} \times \mathcal{U} \rightarrow \mathbb{R}_{\geq}$ . We consider the following problem

$$J^c(s_0, e_0, i_0) = \min_{u \in \mathcal{F}} J_u^c(s_0, e_0, i_0) \quad (14)$$

where  $\mathcal{F}$  denotes the set of state feedback time invariant control policies  $u(s, e, i)$ ,  $u : \mathbb{S} \times \mathbb{S} \times \mathbb{S} \rightarrow \mathcal{U}$ .  $J_u^c(s_0, e_0, i_0)$ , defined in (15), is the cost associated with the evolution of the MJP in (5) from the initial condition  $\{s_0, e_0, i_0\}$  under the time invariant state feedback policy  $u$ .

$$J_u^c(s_0, e_0, i_0) = \lim_{T_{N_t} \rightarrow \infty} \mathbb{E} \left[ \int_0^{T_{N_t}} g_c(i(t), u) dt \middle| S(0) = s_0, E(0) = e_0, I(0) = i_0 \right] \quad (15)$$

## 4 Results

We summarize first the results that will be presented in Section 4 for the Problems described in Section 3. The results are then presented in detail in the subsections that follow.

- In Section 4.1 we consider Problem 2 for the SI epidemic and we show that for costs as in (9) that are linear in the number of infected  $i$  and otherwise nonlinear with respect to the mitigation measures, there is no incentive to make use of increasingly restrictive interventions for increasing prevalence  $i/N$ . In Section 4.1.1 we then consider cost functions as in (11) that also allow mitigation measures applied to the whole population, and we quantify a cost parameter threshold below which infection sensitive feedback policies are not effective to tame the spread of the disease.

- In Section 4.2 we extend our results to Problem 1 for the SIR epidemic. We make use of the computational tools developed in Section 5 for finding optimal policies, which apply to arbitrary complex epidemics, and we find that also for this more complex epidemic prevalence sensitive feedback policies are not effective to tame the disease. In Section 4.2.3 we discuss when a prevalence sensitive negative feedback policy can be an effective strategy for the SIR epidemic.
- In Section 4.3 we consider the more complex SEIR epidemic and we show that remarkably the results of the previous sections hold also for this epidemic.
- In Section 4.4 we consider an equivalent deterministic optimal control problem for the SIR epidemic. We illustrate that optimal policies are not sensitive to infection prevalence also in this simplified setting.
- Finally, in Section 4.5 we show that prevalence sensitive feedback schemes are not effective even when a random number of infected individuals are infected for each infection event, an effect known as *bursts*.

#### 4.1 Limitations of prevalence sensitive policies for the Susceptible Infected (SI) epidemic

We consider in this Section Problem 2 for the SI model with costs of the type in (9).

In Proposition 1 below we give our first result. In particular, we show that for the considered costs, the optimal policy  $u^*(i)$  is non-increasing in the variable  $i$ , *i.e.* the controlled transmission rate is non-decreasing in  $i$  under an optimal policy. This implies that negative feedback policies with respect to prevalence, *i.e.* policies associating increasingly stricter interventions for increasing prevalence levels, are not effective in taming the effects of the epidemic for any value of the cost and system parameters considered.

Numerical computations of the optimal policies validating this result are presented in Section B.3. These show that the optimal policies are predominantly constant further highlighting that there is no incentive to vary interventions to tame the epidemic.

**Proposition 1** *Consider Problem 2 with stage cost  $g_c(i, u)$  selected as in (9). Then the optimal control policy  $u^*(i)$  satisfies*

$$u^*(i+1) \leq u^*(i), \quad \forall i \in \mathbb{S} \quad (16)$$

*Proof* See Section 5.3. □

Various remarks about the Proposition are provided below.

**Remark 1** *Proposition 1 establishes that the optimal policies  $u^*(i)$  are non-increasing with the number of infected  $i$  (or equivalently with prevalence  $i/N$ ). Hence the controlled transmission rate  $\beta_f(i, u^*(i))$  (see (3)) is non-decreasing with the number of infected. This implies the surprising result that the optimal policies do not implement a negative feedback scheme, since for increasing infection prevalence the mitigation measures are not increased (or equivalently the infection rate is not decreased).*

**Remark 2** It should be noted that the result in Proposition 1 holds for arbitrary system and cost parameters. In particular, it holds for arbitrary  $c_1 \in \mathbb{R}_{>}, c_2 \in \mathbb{R}_{>}, c_3 \in \mathbb{R}_{\geq}$  and for any function  $z(u) : \mathcal{U} \rightarrow \mathbb{R}_{\geq}$  in (9). It also holds for an arbitrary non-increasing function  $h(u) : \mathcal{U} \rightarrow [0, 1]$  and for arbitrary recovery rate  $\gamma \in \mathbb{R}_{>}$  and transmission parameter  $\mu \in \mathbb{R}_{>}$ . Furthermore, the set  $\mathcal{U}$  of control inputs and its cardinality  $N_u$  can also be chosen arbitrarily.

**Remark 3** Since we consider an arbitrary feedback policy and an arbitrary function  $z(u)$  in the cost, the result of Proposition 1 can be obtained irrespectively of Assumption 1. In particular, the conclusion that under an optimal policy the infection rate  $\mu\beta_f(i, u)$  is a non-decreasing function of the number of infected  $i$ , follows without requiring  $h(u)$  to be non-increasing in  $u$ . We discuss this in more detail and with some examples in Section B.1.

**Remark 4** Proposition 1 shows that negative feedback is ineffective even in the ideal setting where prevalence is directly observed. It should be noted that if the infection prevalence is not directly observed and needs to be inferred then there is still no incentive to use negative feedback as the corresponding control policy would be in this case even less effective in reducing the desired cost.

**Remark 5** Proposition 1 holds also when, depending upon  $h(u)$  and the set  $\mathcal{U}$ , in an optimal policy it may not be possible to achieve values of  $\mathcal{R}^* < 1$ . Frequent choices of  $h$  such as  $h(u) = (1 - q_{eff}u)$  or  $h(u) = (1 - q_{eff}u)^2$  may not yield  $\mathcal{R}^* < 1$  due to the low effectiveness of the interventions  $q_{eff} \ll 1$  even with the most restrictive measure available, i.e.  $u_{N_u} = 1$ . Small values of  $u_{N_u}$  may also not yield  $\mathcal{R}^* < 1$  irrespectively of effectiveness  $q_{eff}$ . The optimal policies in these settings are of practical relevance for example when a pharmaceutical intervention, e.g. vaccine, is in development or when a reduction of high infection peaks is desirable such as for common flu.

**Remark 6** Another benefit that follows from the monotone property of the optimal policy established in Proposition 1, is that one can considerably reduce the computation time when the optimal control policy is numerically computed. One such algorithm with reduced computation time is provided in the Appendix, in Section A.11.

**Remark 7** Prevalence measurements, have been the focus of various studies [28], and even though they can be non effective in controlling epidemics as quantified in Proposition 1, they are needed in order to estimate key transmission parameters, such as  $\mathcal{R}_0$  and  $h(u)$ , which are required to find the optimal policy.

#### 4.1.1 Effectiveness of prevalence sensitive feedback policies for the Susceptible Infected (SI) epidemic

In this section we consider Problem 2 for costs functions with that include individual and population wide intervention costs of the type in (11). We derive analytically a cost ratio threshold below which prevalence sensitive feedback policies can be effective and above which it is optimal to ignore prevalence and use constant disease mitigation

measures. Numerical computations of the optimal policies validating the results are given in Section B.3.

**Proposition 2** Consider Problem 2 with stage cost  $g_c(i, u)$  as in (11). Then the optimal control policy  $u^*(i)$  satisfies

$$u^*(i+1) \leq u^*(i) \quad \forall i \geq \bar{i} \quad (17)$$

where

$$\bar{i} = -\frac{\chi + 2N}{2\chi} + \sqrt{\frac{\chi^2 + 4\chi N^2 + 4N^2}{4\chi^2}} \quad (18)$$

with

$$\chi = c_2/c_4 \quad (19)$$

*Proof* See Section 5.3. □

Various remarks about the proposition are provided below.

**Remark 8** Proposition 2 establishes that the optimal policies  $u^*(i)$  are non-increasing with respect to infection levels after a threshold  $\bar{i}$  that depends upon the cost parameter ratio  $\chi$ . It follows that the controlled transmission rate is non-decreasing with respect to prevalence levels. It also should be noted that the result in Proposition 2 holds for arbitrary system parameters, for arbitrary  $c_3$ , for an arbitrary set  $\mathcal{U}$  and irrespectively of its cardinality  $N_u$ .

**Remark 9** It should be noted that the relative value of  $\bar{i}$  over  $N$  when  $N$  tends to infinity is

$$\lim_{N \rightarrow \infty} \frac{\bar{i}}{N} = \frac{\sqrt{\chi + 1} - 1}{\chi} \quad (20)$$

It follows that for increasing values of  $\chi$  there is less incentive to make use of a negative feedback scheme to tame the infections for an increasing percentage of the values of  $i$  within the population. In particular, for large values of  $\chi$ , i.e. when the marginal cost per individual  $c_2$  is high with respect to the cost per individual  $c_4$  of using measures for the entire population it follows that  $\frac{\bar{i}}{N} \rightarrow 0$ . Note that for population wide costs  $c_4$  that are comparable to the marginal costs per individual  $c_2$ , i.e.  $\chi \approx 1$ , a prevalence sensitive feedback scheme may be beneficial for  $\bar{i}/N \lesssim \sqrt{2} - 1 = 0.41$ .

## 4.2 Limitations of prevalence sensitive feedback policies for the Susceptible Infected Removed (SIR) epidemic

### 4.2.1 Ineffectiveness of negative feedback policies for the Susceptible Infected Removed (SIR) epidemic

In this section we make use of the computational tools for finding optimal policies developed in Section 5.1, which are applicable to epidemic models with arbitrary number of states, to investigate the form of the optimal policies in more advanced epidemic models. In particular, we start by investigating the optimal policies for the SIR model in Problem 1 with costs as in (9), i.e.  $g_c(i, u) = \zeta i u + i$ . A representative

figure is shown in the diagrams of Fig. S1 where  $\mathcal{R}^* = \mathcal{R}_0 h(u^*(s, i))$  is illustrated for four cases with  $\zeta = \{1, 10\}$  and  $\mathcal{R}_0 = \{1.6, 3.5\}$  respectively. Additional computations of optimal policies and related discussion are presented in Section B.2. The optimal policies for the more advanced SEIR transmission models are also discussed in the following section.

The methodology used to compute the optimal policies is described in Section 5.1. This exploits the absorbing boundary of the considered MJP and makes use of the *uniformisation* method, which yields a discrete time MDP. We then use the value iteration algorithm which allows to explicitly compute the optimal policies  $u^*(s, i)$  and  $\mathcal{R}^*$ .

We observe in Fig. S1 that the optimal  $\mathcal{R}^*$  is predominantly constant for low values of  $i/N$  and is non-decreasing for increasing prevalence levels. This is an analogous behaviour to that of the optimal policies of the SI model *i.e.* the interventions are non-increasing for increasing prevalence levels and thus the optimal policies do not incorporate negative feedback with respect to prevalence. In addition, the policies are constant with respect to prevalence and therefore there is no incentive to vary the optimally chosen interventions since this is not directly useful to minimise the total epidemic costs. It should be noted that prevalence levels measurements are nevertheless required in order to infer the parameters of the transmission mechanism, such as  $\mathcal{R}_0$  and  $h(u)$  and explicitly compute the optimal policies. In particular, as the optimal policies are constant there is no incentive to change interventions and hence efforts should be focused on quantifying key parameters and costs.

In an SIR epidemic model the transmission rate depends also upon the number of susceptible  $s$ . Specifically, low values of  $s$  reduce the transmission rate via a form of negative feedback known as *herd immunity*[29], that generally occurs at slow timescales. Negative feedback schemes on the faster timescales of the infection dynamics do not appear, however, in the optimal policies irrespectively of the levels of  $s$ . In particular, the optimal  $\mathcal{R}^*$  is predominantly constant before the *herd immunity threshold* [30, 31]  $H_i$  defined below is reached. Beyond this point expected levels of prevalence decrease due to a decrease in the number of susceptible  $s$ , [20, 32], and mitigation measures in optimal policies are also relaxed.

$$H_i = (1 - 1/\mathcal{R}_0) \quad (21)$$

In particular,  $H_i$  corresponds to the proportion of population that has to be removed from the susceptible pool due to recoveries or vaccinations so that, in the absence of transmission mitigation interventions expected prevalence levels decrease<sup>2</sup>.

Fig.S1 illustrates that high values of the intervention-to-hospitalization cost ratio  $\zeta$  defined in (10) lead to optimal  $\mathcal{R}^*$  where interventions are eased at low prevalence; *i.e.* it is optimal to rely upon herd immunity effects rather than implementing interventions to try to control the disease. Low values of  $\zeta$  correspond to policies for which interventions are implemented even for very high prevalence levels thus implementing interventions is beneficial even beyond  $H_i$  since these can reduce the mitigation of the

---

<sup>2</sup>Analogously the effective reproduction number  $\mathcal{R}_e = 1$ .

disease at low cost. Increasing values of the reproduction number  $\mathcal{R}_0$  yield policies for which interventions are implemented for increasingly higher values of prevalence.

It should be noted that similar features have been verified for a broad range of relevant linear and nonlinear functions  $h(u)$  and  $z(u)$ , as well as for a large range of intervention-to-hospitalization cost ratios  $\zeta$  and basic reproduction number  $\mathcal{R}_0$ . We investigate the effect of the optimal policies in these settings as well as others in Section B.2.

It should also be noted that if the infections levels are not directly accessible and have to be inferred then there is still no incentive to tame infection levels via a negative feedback scheme on the infection dynamics as the associated policy would be even less effective in reducing the total cost of the epidemic.

#### 4.2.2 Examples of epidemic trajectories

In Fig. S2 we provide a representative figure of the expected prevalence levels  $\mathbb{E}[I(t)/N]$  and the expected costs  $\mathbb{E}[g_c(i, u)]$  when implementing the non-increasing optimal policy associated with Problem 1 and when using the ad-hoc suboptimal negative feedback policy  $u_{fb}$  defined below, *i.e.* a feedback law implementing intervention  $u_{N_u}$  after the threshold  $i_{th}$ .

$$u_{fb}(i) = \begin{cases} 0 & \text{if } i \leq i_{th}, \\ u_{N_u}, & \text{otherwise} \end{cases} \quad (22)$$

Fig. S2 shows that the optimal policy (—) yields lower infections levels and total number of infections with respect to suboptimal negative feedback laws (---, ····). It should be noted that higher values of  $i_{th}$  yield higher prevalence peaks but shorter epidemics and may lead to a significant increase of fatalities for diseases with high infection to fatality ratios [43, 44]. Fig. S2(b) reflects this on the expected costs which are incurred for longer periods of time when the negative feedback interventions are taken for lower values of  $i_{th}$ . It should be noted that Fig. S2 is a representative diagram and we have found similar conclusions to hold for more complex suboptimal negative feedback policies, a large range of parameters and for several functions  $h(u)$  and  $z(u)$ .

Fig. S3 displays the ratio between the total costs  $J_{u_{fb}}^c(s, i)$  defined in (6) that are associated with the suboptimal negative feedback policies (22) over the optimal total costs  $J^c(s, i)$  for Problem 1 defined in (7). The diagrams show that irrespectively of  $\zeta$  and the initial condition, using a negative feedback scheme on the infection yields higher costs with respect to implementing the optimal constant mitigation measures. The diagrams also show that the costs of suboptimal negative feedback schemes that vary interventions at low values of  $i_{th}$  are close to the cost of optimal costs irrespectively of  $\zeta$ . This is because for low values of  $i_{th}$ , the suboptimal policies are close to the optimal policies and result in short periods of exponential growth of the infections before the interventions are used. We have found similar conclusions to those in Fig. S3 to hold for more complex suboptimal negative feedback policies, and a wide range of parameters and functions  $h(u)$  and  $z(u)$ .

### 4.2.3 Effectiveness of prevalence sensitive feedback policies for the Susceptible Infected Removed (SIR) epidemic

We make use of the computational methods developed in Section 5.1 and compute explicitly the optimal policies for the SIR model with costs of the form in (11) *i.e.*  $g_c(i, u) = c_2 i u + c_3 i + c_4 N u$  with  $v = c_4/c_3 = 50$ ,  $c_2 \approx 0$ .

Fig. S4 displays the optimal policies  $u^*(s, i)$  for  $\mathcal{R}_0 \in \{2.5, 3.5\}$ . The figure illustrates that prevalence sensitive feedback schemes can be optimal for high values of  $c_4$ , with respect to  $c_2$  and  $c_3$ , *i.e.* when the population wide costs are considerably higher than the costs for the targeted measures and when these cost considerably outweigh the cost associated with the infected. The considered regime occurs when isolations and social distancing measures are insufficient to tame the infection and stay-at-home interventions are costly. Stay-at-home strategies or business closure orders may be required, for example, for high value of  $\mathcal{R}_0$  when the adopted interventions are insufficient to lower  $\mathcal{R} < 1$ . In particular, Fig. S4 shows that for high values of  $\mathcal{R}_0$  and high values of  $v = c_4/c_3$  the optimal policies are sensitive to infection prevalence with increasingly restrictive interventions for increasing prevalence levels: a result in agreement with recent studies [27] where parametric uncertainty is also considered. For all the considered cases interventions are eased at prevalence levels that depend upon the ratio  $v = c_4/c_3$  of intervention over hospitalisation costs. Furthermore, population wide interventions are used in these cases also after the herd immunity threshold  $H_i$  defined in (21) is reached.

In Fig. S5 we display  $\mathbb{P}(i/N, t)$ , *i.e.* the probability that at time  $t$  the prevalence is  $i/N$  when using the optimal negative feedback law associated with costs as  $g_c(i, u) = c_3 i + c_4 N u$ . Fig. S5(a) corresponds to the epidemics with  $\mathcal{R}_0 = 2.5$ , which result in a high probability that the epidemics go extinct early and a peak of prevalence at approximately  $i/N \approx 35\%$ . Fig. S5(b) shows the prevalence probability for  $\mathcal{R}_0 = 3.5$  under the associated optimal policy. For this value of  $\mathcal{R}_0$  there is a lower probability that epidemics go extinct early when compared to Fig. S5(a) due to the increase of  $\mathcal{R}_0$  and prevalence has a peak approximately  $i/N \approx 45\%$ .

### 4.3 Limitations of prevalence sensitive feedback policies for the Susceptible Exposed Infected Removed (SEIR) epidemic

In this section we investigate the optimal policies for the more advanced SEIR transmission model in Problem 3 for costs  $g_c$  as in (9). The policies are computed using the computational tools developed in Section 5.1 that can be used for epidemic models with arbitrary complexity. Such computation is shown in Fig. S6 where the optimal policy  $u^*(s/N, e/N, i/N)$  is illustrated with respect to  $s/N$  and  $i/N$  for different fixed levels of practically relevant exposure prevalence  $e/N = \hat{e}/N$  with  $\hat{e}/N = 0.02, 0.03$ . We observe that the optimal policies for low values of  $\hat{e}$  are analogous to those obtained for the SIR epidemic, *i.e.* the policies are predominantly constant and are non increasing with respect to prevalence. Thus there is no incentive to vary the optimally chosen measures and the optimal policies do not implement a negative feedback scheme on the infections. It should be noted that the exposed category, where individuals spend a random amount of time, does not affect our results as it models the difficulty of

effectively measuring prevalence which has been found not to be a useful signal to mitigate the epidemic. It should be noted that Fig. S6 is only representative of our result and similar conclusions have been obtained for a wide range of cost and system parameters as well as choices of  $h(u)$  and  $z(u)$ .

#### 4.4 Deterministic Susceptible Infected Removed (SIR) epidemic and problem formulation

For completeness we compute the optimal policies also for a deterministic version of the SIR model and verify that these validate the results of the stochastic formulation presented in the previous sections. It should be noted that our results are based upon stochastic models that are more accurate than deterministic formulations which hold only in the limit of large  $N$ .

Let us consider a population of size  $N \in \mathbb{Z}_{>}$ . We denote with  $\mathbb{D}$  the values of  $z$  such that  $\mathbb{D} = \{z \in \mathbb{R}_{\geq} | 0 \leq z \leq N\}$  and we denote with the variables  $x_S, x_I$  and  $x_R$  the number of susceptible, infected and recovered individuals of the considered population taking values in  $\mathbb{D} \times \mathbb{D} \times \mathbb{D}$ . We consider a constant population of  $N$  individuals and hence  $x_S + x_I + x_R = N$ . It follows that  $x_R = N - x_S - x_I$  and therefore without any loss of generality in the remainder of the section we consider only the quantities  $x_S$  and  $x_I$ . In order to simplify the notation in the following derivations we consider the variable  $x_S$  and  $x_I$  stacked in vector  $x = \begin{bmatrix} x_S \\ x_I \end{bmatrix} \in \mathbb{D}^{2 \times 1}$ .

The system of Ordinary Differential Equations (ODEs) associated with the deterministic SIR epidemic model [47–49], is

$$\dot{x} = f(x(t), u(t)), \quad x(0) = [x_S(0), x_I(0)]^T \quad (23)$$

where  $\dot{x} = \left[ \frac{dx_S}{dt}, \frac{dx_I}{dt} \right]^T$  and the function  $f(x(t), u) : \mathbb{D}^{2 \times 1} \rightarrow \mathbb{D}^{2 \times 1}$  is defined as

$$f(x, u) = \left[ -\mu \frac{x_S x_I}{N} h(u), \mu \frac{x_S x_I}{N} h(u) - \gamma y \right]^T \quad (24)$$

The quantities  $\gamma$ ,  $\mu$  and  $h(u)$  appearing in (24) are the deterministic versions of the quantities defined for the MJP in Section 2.3.

We now consider Problem 4, defined below, *i.e.* a deterministic continuous valued version of Problem 1 and we consider the cost function  $g_{x_I}(x_I(t), u(t)) : \mathbb{D} \times \mathcal{U} \rightarrow \mathbb{R}_{\geq}$ , *i.e.* the cost per unit of time for the deterministic formulation.

We consider without any loss of generality only time independent policies as it can be shown that the optimal policies for infinite horizon problems are independent of time. A particular policy for the system in (23) is denoted by  $u : \mathbb{D} \times \mathbb{D} \rightarrow \mathcal{U}$ . With  $\mathcal{F}$  we denote the set of time invariant state feedback policies, *i.e.* the set of functions  $u$  which for each value of the state  $x_S, x_I$  give an element in  $\mathcal{U}$ . We consider without any loss of generality only time invariant feedback laws since it can be shown that the policies for an infinite horizon problem are independent of time [24, 25].



**Problem 4** Consider the system in (23). We consider the following problem

$$V^c(x(0), t_0) = \min_{u \in \mathcal{F}} [V_u^c(x(0), t_0)] \quad (25)$$

where  $\mathcal{F}$  denotes the set of state feedback time invariant control policies  $u : \mathbb{D}^{2 \times 1} \rightarrow \mathcal{U}$ .  $V_u^c(x(0), t_0)$ , defined in (26), is the cost associated with the evolution of the system in (23) from the initial condition  $x(0)$  under the time invariant state feedback policy  $u$ .

$$V_u^c(x(0), t_0) = \lim_{T \rightarrow \infty} \int_{t_0}^T g_{x_I}(x_I(t), u(t)) dt \quad (26)$$

The function  $V(x, t)$  is the value function for Problem 4.

In order to compute the optimal policies for Problem 4 we make use of Dynamic Programming (DP) [50]. This formulation casts the minimisation problem into the Hamilton-Jacobi-Bellman Equation (HJBE) a particular Partial Differential Equation (PDE) that the optimal policies have to satisfy. Differently from the Pontryagin's Maximum Principle (PMP) [51], this formulation allows to obtain optimal feedback policies that are a function of the state variable  $x(t)$  by solving a PDE.

Associated with Problem 4 we introduce the function  $H : \mathbb{D}^{2 \times 1} \times \mathcal{U} \times \mathbb{D}^{2 \times 1} \rightarrow \mathbb{R}$  particularised for system (23)

$$H(x(t), u(t), \lambda(t)) = g_{x_I}(x_I(t), u(t)) + \lambda(t)^T f(x(t), u(t)) \quad (27)$$

The function  $H$  in (27) is the Hamiltonian [52], and is a convenient notion, that stems from classical mechanics, that allows to solve optimal control problems such as Problem 4. The quantity  $\lambda(t) \in \mathbb{D}^{2 \times 1}$  is the co-state and is a time varying quantity analogous to the Lagrange multipliers found in the literature for static optimisation problems [53].

We now state the following Proposition, a well known result in control theory, giving a necessary and sufficient condition<sup>3</sup> for the optimality of the control policy.

**Proposition 3** Consider Problem 4 and the associated Hamiltonian function in (27). Then a necessary and sufficient condition for an optimal policy  $u^*(x)$  is to satisfy the following Hamilton-Jacobi-Bellman Equation (HJBE)

$$-V_t(x) = \inf_{u \in \mathcal{U}} H(x(t), u(t), -V_x(x)) \quad (28)$$

where  $V_t = \frac{\partial V(x, t)}{\partial t}$ ,  $V_x = \frac{\partial V(x, t)}{\partial x}$  and  $V(x, T) = g_{x_I}(x_I(T), u(T))$ .

*Proof* See [52]. □

Due the constraint on the control value  $u$  in (28) an analytical expression for the feedback policy in this deterministic setting cannot be derived and is computed numerically. Via numerical computations in Fig. S7 we solve Problem 2 and Problem

---

<sup>3</sup>It should be noted that Proposition 3 is stated for time dependant policies. By considering the limit as the time horizon goes to infinity the optimal policies are required to satisfy  $\inf_{u \in \mathcal{U}} H(x(t), u(t), -V_x(x)) = 0$  for arbitrary boundary conditions.

4, *i.e.* the optimal control problems for the stochastic and deterministic SIR epidemic. We observe that the optimal policies are constant and non-increasing with respect to the number of infected in both formulations and hence also for the deterministic SIR model negative feedback is ineffective in mitigating the disease. The computations have been performed using the computational tools derived in Section 5.1 for the stochastic SIR optimal control Problem, and using the HJBE in (28) for the deterministic Problem. The HJBE has been solved via the software in [54] for  $h(u) = 1 - u$  but similar results have been obtained for different choices of  $h$  and also when the costs are of the form  $g_{x_I}(y, u) = c_1 + c_2 x_I u + c_3 x_I + c_4 u N$ .

## 4.5 Epidemics with random infection outcomes

In this Section we extend the result of the previous Sections to epidemics with heterogeneous infection events. We consider a more complex version of the SI and SIR models where a random number of individuals are infected for each infection event. In the rest of the manuscript we refer to this effect as *bursts*.

We first extend the MJP of the SIR transmission model and introduce the required mathematical quantities. We then formulate a MJP version of the SI transmission model where bursts are considered and define an equivalent minimisation problem to Problem 2 for this setting. We make use of this formulation and we present an extended version of Proposition 1 when bursts are considered. The results are derived in Section 5.4.

We consider the stochastic SIR model defined in Section 2.3 and consider that for a single infection event a random number of people  $Q$  transition from the Susceptible to the Infected category. This can for example model the presence of super nodes, *i.e.* individuals that spread the infection to a large number of individuals, or it can serve as first approximation of spatial and demographic effects.

We consider the variables  $S(t), I(t), R(t), u$ , the parameters  $\mu, \gamma$  and the function  $h(u)$  defined in Section 2.3. The random variable  $Q$  is assumed to be independent from the random variables  $S(t)$  and  $I(t)$ . We also assume that  $Q$  has a known Probability Mass Function (p.m.f.)  $\pi_Q$  defined on the support  $\mathbb{Q} = \{1, \dots, N_q\}$  with  $N_q \in \mathbb{Z}_{>}$ . We denote with  $\mathbb{P}_Q(q)$  the probability that the random variable  $Q = q$ .

The events we consider, and the associated rates for this model, are summarised in Table S2.

| Event     | Transition                                | Rate                           |
|-----------|-------------------------------------------|--------------------------------|
| Infection | $(S, I, R) \rightarrow (S - Q, I + Q, R)$ | $\frac{\mu S I \cdot h(u)}{N}$ |
| Removal   | $(S, I, R) \rightarrow (S, I - 1, R + 1)$ | $\gamma I$                     |

**Table S2:** Table of transition rates for the SIR model with random infection outcomes

The system in Table S2 is defined by the following Master equation

$$\begin{aligned} \frac{\partial \mathbb{P}(s, i, t)}{\partial t} = & \left[ \sum_{q=1}^{N_q} \mathbb{P}_Q(q) \mu(s+q)(i-q)/Nh(u) \mathbb{P}(s+q, i-q, t) \right] \\ & - \mu si/Nh(u) \mathbb{P}(s, i, t) + \gamma[(i+1) \mathbb{P}(s, i+1, t) - i \mathbb{P}(s, i, t)] \end{aligned} \quad (29)$$

We consider the following optimal control problem for the SIR epidemic with random infection outcomes with events in Table S2 satisfying (29). We show and discuss optimal policies for this problem in Section B.2.2.

**Problem 5** Consider the system in (29). We consider the following problem:

$$J^{Q,c}(s_0, i_0) = \min_{u \in \mathcal{F}} J_u^{Q,c}(s_0, i_0) \quad (30)$$

where  $\mathcal{F}$  denotes the set of state feedback time invariant control policies  $u(i)$ ,  $u : \mathbb{S} \rightarrow \mathcal{U}$ .  $J_u^{Q,c}(s_0, i_0)$ , defined in (31), is the cost associated with the evolution of the MJP in (32) from the initial condition  $\{s_0, i_0\}$  under a time invariant state feedback policy  $u$ .

$$J_u^{Q,c}(s_0, i_0) = \lim_{T_{N_t} \rightarrow \infty} \mathbb{E} \left[ \int_0^{T_{N_t}} g_c(i(t), u) dt \middle| S(0) = s_0, I(0) = i_0 \right] \quad (31)$$

Analogously to the SIR epidemic transmission model we derive the SI model where bursts are considered satisfying the following Kolmogorov Equation

$$\begin{aligned} \frac{\partial \mathbb{P}(i, t)}{\partial t} = & -\mu \beta_f(i, u) \mathbb{P}(i, t) \\ & + \left[ \sum_{q=1}^{N_q} \mathbb{P}_Q(q) \mu \beta_f(i-q, u) \mathbb{P}(i-q, t) \right] \\ & + \gamma[(i+1) \mathbb{P}(i+1, t) - i \mathbb{P}(i, t)] \end{aligned} \quad (32)$$

where  $\beta_f(i, u)$ , similarly as the case with no bursts, is defined as in (3)

We now consider the following Problem for the stochastic SI model where bursts are taken into consideration for the infection events.

**Problem 6** Consider the system in (32). We consider the following problem:

$$J^c(i) = \min_{u \in \mathcal{F}} J_u^c(i_0) \quad (33)$$

where  $\mathcal{F}$  denotes the set of state feedback time invariant control policies  $u(i)$ ,  $u : \mathbb{S} \rightarrow \mathcal{U}$ .  $J_u^c(i_0)$ , defined in (34), is the cost associated with the evolution of the MJP in (32) from the initial condition  $i_0$  under a time invariant state feedback policy  $u$ .

$$J_u^c(i_0) = \lim_{T_{N_t} \rightarrow \infty} \mathbb{E} \left[ \int_0^{T_{N_t}} g_c(i(t), u) dt \middle| I(0) = i_0 \right] \quad (34)$$

We now give our result showing that the optimal policies  $u^*(i)$  are non-increasing in the variable  $i$  also when bursts are considered and irrespectively of the distribution  $\pi_Q$  of the bursts.

**Proposition 4** *Consider Problem 6, i.e. an equivalent formulation of Problem 2 where bursts are considered and consider  $g_c(i, u)$  to be selected as in (9). Then the optimal policy  $u^*(i)$  satisfies*

$$u^*(i+1) \leq u^*(i), \quad \forall i \in \mathbb{S} \quad (35)$$

*Proof* See Section 5.4. □

**Remark 10** *Note that Proposition 4 is identical to Proposition 1, i.e. for the SI model satisfying (4) where bursts are not considered. The result shows that there is no incentive to make use of negative feedback policies to tame the transmission of the disease also when infection events have random outcomes. The optimal policies however have different forms depending upon the distribution  $\pi_Q$  as shown in Fig. S8.*

In Fig. S8 we make use of the computational tools developed in Section 5 to explicitly compute the optimal policies for Problem 6 for various values of  $c_2$  and for different  $p, q : \pi_Q \sim \mathcal{B}(p, n)$ . The diagrams in Fig. S8 show the optimal policies  $u^*(i)$  for different values of the expected value  $\mathbb{E}_{\pi_Q}[Q]$ . Increasing  $\mathbb{E}_{\pi_Q}[Q]$  leads to policies that decrease at higher values of  $i$ .

By means of numerical computations of the optimal policies we have also verified that similar conclusions to the ones found in Fig. S8 apply also to the more complex SIR and SEIR models.

## 5 Derivation of the results

We start in Section 5.1 by developing tools that allow to explicitly compute the optimal policies for general stochastic epidemic models (which include also the ones described in the previous Sections). The methodology developed is based on the conversion of the considered continuous time Problem to that of an equivalent discrete time one for which the optimal policies can then be computed via the Bellman equation and the *value iteration* algorithm.

We make also use of this equivalent discrete time formulation throughout the derivation of Proposition 1. In particular, we define an equivalent discrete time problem for Problem 2 in Section 5.1 (defined as Problem 8), and in Section 5.2 we give some preliminary results associated with the characterisation of its solution and convergence properties. We then derive various Lemmas (Section 5.3) associated with the positivity and the one step finite differences of the *value function*. These then allow to deduce generic properties of the optimal policies via induction arguments. These intermediate Lemmas enable us then to prove our main results stated in Sections 4.1-4.4.

We then provide in in Section 5.4 the proof of Proposition 4, the extended version of Proposition 1 for the SI epidemic introduced in Section 4.5, where there is randomness in the number of individuals infected for each event.

The proofs of the Lemmas and Propositions in Section 5 are given in in Appendix A.

## 5.1 Formulation as equivalent discrete time Markov Decision Processes (MDPs)

In order to characterise the optimal policies we derive equivalent discrete time optimal control problems to those of the previous Sections via the method of *uniformisation* [25]. This methodology applies to epidemics with an arbitrary number of compartments and is used also to characterise the optimal policies for Problem 6 (Section 5.4) where random infection outcomes are considered.

Consider Problem 1 and the SIR model in (2). The infection and recovery events of the considered SIR system in Problem 1 take place at random moments in time indicated by  $T_k$ . The holding time of the process in a specific state, *i.e.* the time between two consecutive transitions, is exponentially distributed with a parameter denoted by  $\xi(s, i, u) : \mathbb{S} \times \mathbb{S} \times N_u \rightarrow \mathbb{R}_>$ . In particular,  $\xi(s, i, u)$  denotes the holding time parameter of the process in state  $s, i$ , under control  $u$  and it can be shown that it is the sum of the rates associated with the considered state and control, *i.e.*  $\xi(s, i, u) = \frac{\mu}{N} si \cdot h(u) + \gamma i$  [24].

In order to define an equivalent discrete time process, referred to as the *uniformised* process, consider  $\nu \in \mathbb{R}_>$  such that

$$\begin{aligned} \nu &\geq \max_{s, i, u} \xi(s, i, u) \\ &= \max_{s, i, u} \left[ \frac{\mu}{N} si h(u) + \gamma i \right] \end{aligned} \quad (36)$$

The uniformised process is defined as follows. Consider a discrete time Markov Chain  $\{S_k, I_k\}$  taking values in  $\mathbb{S} \times \mathbb{S}$  where  $k$  is the time step. The transition probabilities of the Markov chain are denoted by  $p_{[s, i] \rightarrow [t, w]}^u = \mathbb{P}(S_{k+1} = t, I_{k+1} = w | S_k = s, I_k = i)$ , *i.e.* this is the probability that the process transitions from state  $s$  and  $i$  at time  $k$  to state  $t$  and  $w$  at time  $k + 1$ . These transition probabilities are defined as follows

$$p_{[s, i] \rightarrow [t, w]}^u = \begin{cases} \frac{1}{\nu} \frac{\mu}{N} si \cdot h(u) & \text{if } t = s - 1, w = i + 1 \\ \frac{1}{\nu} \gamma i & \text{if } w = i - 1 \\ 1 - \frac{\frac{\mu}{N} si \cdot h(u) + \gamma i}{\nu} & t = s, w = i \end{cases} \quad (37)$$

where  $s, i, t, w \in \mathbb{S}$  and  $\nu$  is defined in (36). Note that the probabilities for all other values of  $t$  and  $w$  are zero since the probabilities in (37) sum up to 1.

Associated with the discrete time MJP specified by (37) consider the following cost function  $g : \mathbb{S} \times \mathcal{U} \rightarrow \mathbb{R}_\geq$ . The function  $g$  is the cost for each discrete step and it

is assumed non negative. We now specify the following discrete time optimal control problem associated with the uniformised process in (37).

**Problem 7** Consider the discrete time Markov Chain specified by the transition probabilities in (37). We seek to solve the following problem

$$J(s_0, i_0) = \min_{u \in \mathcal{F}} J_u(s_0, i_0) \quad (38)$$

where  $\mathcal{F}$  is the set of time invariant state feedback policies  $u(s, i)$ ,  $u : \mathbb{S} \times \mathbb{S} \rightarrow \mathcal{U}$ . The function  $J_u(s_0, i_0)$ , defined below, is the cost associated with the evolution of the discrete time Markov Chain with transition probabilities defined in (37) from the initial condition  $\{s_0, i_0\}$  under a time invariant state feedback policy  $u$ .

$$J_u(s_0, i_0) = \lim_{N_d \rightarrow +\infty} \sum_{k=0}^{N_d-1} \mathbb{E}[g(I_k, u) | S_0 = s_0, I_0 = i_0] \quad (39)$$

The control input  $u(s, i)$  associated with Problem 1 only changes at times  $T_k$ , which are the times the state changes. In order to solve Problem 1 it is thus sufficient to consider the values of the policies when state transitions take place. This allows to reduce Problem 1 to Problem 7, which is based on a discrete time formulation, as stated in Proposition 5 below.

**Proposition 5** Consider Problem 1 and consider  $\nu \in \mathbb{R}_{>}$  as in (36) then the optimal policy for Problem 7 with cost

$$g(i, u) = \frac{1}{\nu} g_c(i, u) \quad (40)$$

is also the optimal policy for Problem 1 where the cost is  $g_c(i, u)$ .

*Proof* See Section A.6. □

In Proposition 5 we refer to a policy that is optimal for Problem 7 to be optimal for Problem 1 in the sense that the feedback law  $u$  is the same function of the states for both Problems.

**Remark 11** An analogous version of Proposition 5 also holds for Problem 2 as discussed below, and more broadly for other MJP epidemic models [55], whereby these can be converted to an equivalent discrete time optimal control problem.

**Remark 12** The transformation to a discrete time MDP with finite state and input values and an absorbing state allows to make use of appropriate iterations, such as the value iteration or policy iteration, to compute the optimal policy with arbitrarily high precision [25]. The former was used for the computation of the optimal policies presented in Section 4.2. Problem 7 can also be associated with a convex linear program, or its dual, for which many solution techniques exist [56].

A discrete time Problem for the MJP corresponding to the SI model in (4) can also be derived. Analogously to Problem 7 the parameter  $\nu$  associated with the SI model has to satisfy<sup>4</sup> (36). More precisely, consider a discrete time Markov Chain  $I_k$  that takes values in  $\mathbb{S}$  and where  $k$  is the time step. The transition probabilities  $p_{ij}^u = \mathbb{P}(I_{k+1} = j | I_k = i)$  are given by (41)

$$p_{ij}^u = \mathbb{P}(I_{k+1} = j | I_k = i) = \begin{cases} \frac{1}{\nu} \beta_f(i, u) & \text{if } j = i + 1 \\ \frac{1}{\nu} \gamma i & \text{if } j = i - 1 \\ 1 - \frac{\beta_f(i, u) + \gamma i}{\nu} & i = j \end{cases} \quad (41)$$

where  $i, j \in \mathbb{S}$  and the transmission rate  $\beta_f(i, u)$ , is defined in (3).

**Problem 8** Consider the discrete time Markov Chain specified by the transition probabilities in (41). We seek to solve the following problem

$$J(i_0) = \min_{u \in \mathcal{F}} J_u(i_0) \quad (42)$$

where  $\mathcal{F}$  is the set of time invariant state feedback policies  $u(i)$ ,  $u : \mathbb{S} \rightarrow \mathcal{U}$ .  $J_u(i_0)$ , defined in (43), is the cost associated with the evolution of the discrete time Markov Chain with transition probabilities as in (41) from the initial condition  $i_0$  under the time invariant state feedback policy  $u$ .

$$J_u(i_0) = \lim_{N_d \rightarrow +\infty} \sum_{k=0}^{N_d-1} \mathbb{E}[g(I_k, u) | I_0 = i_0] \quad (43)$$

We now make use of Remark 11 and formulate an equivalent discrete time Problem to Problem 3 for the SEIR epidemic in (5). We make use of a parallel argument used for (36), for which the uniformisation constant  $\nu$  has to be larger than the sum of all the rates, and we derive the uniformisation factor  $\nu$  for the SEIR model as

$$\begin{aligned} \nu &\geq \max_{s, e, i, u} \xi(s, e, i, u) \\ &= \max_{s, e, i, u} [\mu \text{sinh}(u) + \gamma i + \epsilon e] \end{aligned} \quad (44)$$

where we have denote with  $\xi(s, e, i, u)$  the holding time parameter of the system in the state  $s, e, i$ .

Consider a discrete Markov Chain  $S_k, E_k, I_k$  taking values on  $\mathbb{S} \times \mathbb{S} \times \mathbb{S}$ . We denote with  $p_{[s, e, i] \rightarrow [a, d, f]}^u$  the probability at time step  $k$  the Markov chain transitions from state  $s, e, i$  to state  $a, d, f$  at time  $k + 1$ . More precisely, we define the transition

---

<sup>4</sup>Note that the uniformisation constant  $\nu$  has to be larger than the sum of all the rates. In this case it turns out that the upper bound for the SIR model in (36) is sufficient also for the SI model.

probability  $\mathbb{P}(S_{k+1} = a, E_{k+1} = d, I_{k+1} = f | S_k = s, E_k = e, I_k = i)$  as

$$p_{[s,e,i] \rightarrow [a,d,f]}^u = \begin{cases} \frac{1}{\nu} \frac{\mu}{N} si \cdot h(u) & \text{if } a = s - 1, d = e + 1 \\ \frac{1}{\nu} \epsilon e & \text{if } d = e - 1, f = i + 1 \\ \frac{1}{\nu} \gamma i & \text{if } f = i - 1 \\ 1 - \frac{\frac{\mu}{N} si \cdot h(u) + \gamma i + \epsilon e}{\nu} & a = s, d = e, f = i \end{cases} \quad (45)$$

where  $s, e, i, a, d, f \in \mathbb{S}$ . The optimal control problem associated with the uniformised SEIR epidemic specified by (45) is defined below.

**Problem 9** Consider the discrete time Markov Chain specified by the transition probabilities in (45). We seek to solve the following problem

$$J(s_0, e_0, i_0) = \min_{u \in \mathcal{F}} J_u(s_0, e_0, i_0) \quad (46)$$

where  $\mathcal{F}$  is the set of time invariant state feedback policies  $u(s, e, i)$ ,  $u : \mathbb{S} \rightarrow \mathcal{U}$ .  $J_u(s_0, e_0, i_0)$ , defined in (47), is the cost associated with the evolution of the discrete time Markov Chain with transition probabilities defined in (45) from the initial condition  $s_0, e_0, i_0$  under a time invariant state feedback policy  $u$ .

$$J_u(s_0, e_0, i_0) = \lim_{N_d \rightarrow +\infty} \sum_{k=0}^{N_d-1} \mathbb{E}[g(I_k, u) | S_0 = s_0, E_0 = e_0, I_0 = i_0] \quad (47)$$

## 5.2 Preliminaries associated with Problem 8

In order to derive Proposition 1 we make use of the Bellman equation for optimality and the value iteration algorithm, which is an iteration that is guaranteed to converge to the minimum cost, as we state below in this section [25, 57]. The value iteration algorithm for Problem 8 is

$$J_{k+1}(i) = \frac{1}{\nu} \min_{u \in \mathcal{U}} [g_c(i, u) + \mu \beta_f(i, u) L_k(i) - \gamma i L_k(i - 1) + \nu J_k(i)] \quad (48)$$

where we have introduced the quantity  $L_k(i)$  defined<sup>5</sup> as

$$L_k(i) = J_k(i + 1) - J_k(i) \quad (49)$$

and for simplicity in the notation we remove the subscript from  $i_0$  in the rest of the manuscript.

In the remainder of the manuscript we denote with  $\mathcal{J}_k(i, u)$  the function to be minimised with respect to  $u$  at each time step in the right hand side of (48), i.e.

$$\mathcal{J}_k(i, u) = g_c(i, u) + \mu \beta_f(i, u) L_k(i) - \gamma i L_k(i - 1) + \nu J_k(i) \quad (50)$$

---

<sup>5</sup>We set  $\gamma i L_k(i - 1) = 0$  for  $i = 0$  and  $\beta_f(i, u) L_k(i) = 0$  for  $i = N$ .



and with  $u_k^*(i)$  we denote the optimal policy for state  $i$  at step  $k$  of the value iteration algorithm.

It should be noted that Problem 8 is an infinite horizon optimal control problem with an absorbing state, positive costs, and with finite cardinality  $N_u$  of the mitigation measures  $\mathcal{U}$ . As stated in the following Lemma [25] (48) is known to converge to the minimum cost  $J(i)$ , which is the solution of the Bellman equation (51).

**Lemma 1** *Consider Problem 8. Then for any initial condition  $J_0(i)$  the value iteration algorithm in (48) converges to the optimal cost  $J(i)$  which is the unique solution to the Bellman equation*

$$J(i) = \frac{1}{\nu} \min_{u \in \mathcal{U}} [g_c(i, u) + \mu \beta_f(i, u) L(i) - \gamma i L(i-1) + \nu J(i)] \quad (51)$$

where  $L(i)$  denotes the quantity.

$$L(i) = J(i+1) - J(i) \quad (52)$$

Furthermore, a policy  $u^*(i)$  is optimal if and only if it solves (51).

*Proof* See [25, Vol.II] □

As stated in Lemma 1 the value iteration algorithm converges for any initial condition. For the derivations that follow we select without loss of generality as initial condition

$$J_0(i) = 0, \forall i \in \mathbb{S} \quad (53)$$

### 5.3 Derivation of Proposition 1

We now give various Lemmas that establish a set of sufficient conditions for  $J_k(i)$  to be positive, increasing and concave in the variable  $i \forall k \in \mathbb{Z}_{\geq}$ . We then show that these Lemmas lead to the result in Proposition 1, via an extended version stated as Proposition 7.

We begin by establishing the positivity of the functions  $J_k(i)$ , i.e.  $J_k(i) \geq 0, \forall k \in \mathbb{Z}_{\geq}$  in Lemma 2 via induction. In Lemma 3 we make use of an induction argument to show that the functions  $J_k(i)$  are increasing in  $i$  for all  $k \in \mathbb{Z}_{\geq}$ , i.e.  $L_k(i) \geq 0$ . The results of Lemma 2 and 3 are used for Lemma 4 where we establish the concavity in the variable  $i$  of the function  $J_k(i)$ , i.e.  $L_k(i-1) - L_k(i) \geq 0, \forall k \in \mathbb{Z}_{\geq}, \forall i$ .

We then derive Proposition 6 and Proposition 7 that are more general technical results that follow from the previous Lemmas. Our main result in Proposition 1 then follows directly from Proposition 7.

We begin by establishing the positivity for all  $i$  of the functions  $J_k(i)$  via the following Lemma.

**Lemma 2** *Consider Problem 8, the value iteration algorithm (48), and select  $J_0(i)$  as in (53). If  $g_c(i, u)$  satisfies*

$$g_c(i, u) \geq 0, \quad \forall i \in \mathbb{S}, \forall u \in \mathcal{U} \quad (54)$$

*Then*

$$J_k(i) \geq 0, \quad \forall k \in \mathbb{Z}_{\geq}, \forall i \in \mathbb{S} \quad (55)$$

*Proof* See Section A.1.  $\square$

The following Lemma shows that the functions  $L_k(i)$  defined in (49) satisfy  $L_k(i) \geq 0, \forall k \in \mathbb{Z}_{\geq}$ .

**Lemma 3** Consider Problem 8, the function  $L_k(i)$  in (49) the value iteration algorithm (48). If the conditions of Lemma 2 are satisfied and if  $g_c(i, u)$  satisfies

$$\Delta_i^1[g_c(i, u)] \geq 0, \quad \forall i \in \mathbb{S}, \forall u \in \mathcal{U} \quad (56)$$

then

$$L_k(i) \geq 0, \quad \forall k \in \mathbb{Z}_{\geq}, \forall i \in \{0, 1, 2, \dots, N-1\} \quad (57)$$

*Proof* See Section A.2.  $\square$

The following Lemma provides conditions for which the function  $J_k(i)$  is a concave function in the variable  $i$ .

**Lemma 4** Consider Problem 8 and the associated value iteration algorithm (48). Assume the conditions of Lemma 3 and Lemma 2 are satisfied.

If  $\beta_f$  satisfies

$$\Delta_i^2[\beta_f(i, u)] \leq 0, \quad \forall i \in \mathbb{S}, \forall u \in \mathcal{U} \quad (58)$$

and  $g_c(i, u)$  satisfies

$$\Delta_i^2[g_c(i, u)] \leq 0, \quad \forall i \in \mathbb{S}, \forall u \in \mathcal{U} \quad (59)$$

then

$$L_k(i-1) - L_k(i) \geq 0, \quad \forall k \in \mathbb{Z}_{\geq}, \forall i \in \{1, 2, \dots, N-1\} \quad (60)$$

*Proof* See Section A.3.  $\square$

The following Proposition is a more technical result that is then used to prove Proposition 1 and Proposition 2.

**Proposition 6** Consider Problem 8. Assume the conditions in Lemma 3 and Lemma 4 are satisfied. If there exists a function  $t(i)$

$$t(i) : \mathbb{S} \rightarrow \mathbb{R}_{>} \quad (61)$$

such that  $\forall u^+, u^- \in \mathcal{U}$  with  $u^+ \geq u^-$ .

$$\frac{t(i+1)}{t(i)} \leq \frac{\beta_f(i, u^-) - \beta_f(i, u^+)}{\beta_f(i+1, u^-) - \beta_f(i+1, u^+)} \quad (62)$$

and

$$\frac{t(i+1)}{t(i)} \geq \frac{g_c(i, u^+) - g_c(i, u^-)}{g_c(i+1, u^+) - g_c(i+1, u^-)} \quad (63)$$

then the optimal feedback policy  $u^*(i)$  satisfies

$$u^*(i+1) \leq u^*(i), \quad \forall i \in \mathbb{S} \quad (64)$$

*Proof* See Section A.4 □

We now particularise Proposition 6 to the case where  $\beta_f$  has the form in (3) and the costs have the form

$$g_c(i, u) = c_1 + c_2 p(i) z(u) + c_3 i \quad (65)$$

where  $p(i)$  is a concave function.

**Proposition 7** Consider Problem 2. Assume the conditions of Lemma 3, Lemma 4 and Proposition 6 are satisfied.

Let  $g_c(i, u)$  satisfy

$$g_c(i, u) = c_1 + c_2 p(i) z(u) + c_3 i \quad (66)$$

where  $z(u) : \mathcal{U} \rightarrow \mathbb{R}_{\geq}$  and  $p(i) : \mathbb{S} \rightarrow \mathbb{R}_{\geq}$ .  $p(i)$  is assumed as per Lemma 4, to be a concave function in the variable  $i$ , i.e.  $\Delta_i^2[p(i)] \leq 0$ .

Then if  $\exists t(i) : \mathbb{S} \rightarrow \mathbb{R}_{>}$  such that

$$\frac{p(i)}{p(i+1)} \leq \frac{t(i+1)}{t(i)} \leq \frac{i(N-i)}{(i+1)(N-i-1)} \quad (67)$$

it follows that

$$u^*(i+1) \leq u^*(i) \quad (68)$$

*Proof* We make use of Proposition 6 leading to the condition in (67). □

Our main result in Proposition 1 is a direct Corollary of Proposition 7.

*Proof of Proposition 1* We consider the equivalent Problem 8 as discussed in Section 5.1. We then make use of Proposition 7 with  $t(i) = \frac{1}{i}$  and  $p(i) = i$  and Proposition 1 follows directly. □

Proposition 2 follows by making use of Proposition 6 when  $g_c(i, u)$  is selected as in (11). The proof is given in the Appendix, Section A.5.

## 5.4 Derivation of Proposition 4

In this Section we derive Proposition 4, given in Section 4.5. The Proposition establishes that the optimal policies are non-increasing also when a random number of infected individuals transition from the susceptible to infected category for an infection event. As in Section 4.5 we refer to this effect as *bursts*.

We now define some quantities that will be used in the following derivations. By adapting the results of Proposition 5 to Problem 6 where the process satisfying (32) is taken into consideration, we construct an equivalent discrete time optimal control Problem that is used for the derivations.

Consider a discrete time Markov Chain  $I_k^q$ . The process  $I_k^q$  is defined on the set  $\mathbb{S}$ , introduced in Section 2.3, where  $k$  is the time step. The transition probabilities of the Markov Chain  $p_{i,j}^{uq} = \mathbb{P}(I_{k+1}^q = j | I_k^q = i)$  are defined in (69). Consider  $i, j \in \mathbb{S}$  and

$$p_{i,j}^{uq} = \mathbb{P}(I_{k+1}^q = j | I_k^q = i) = \begin{cases} \frac{1}{\nu} \mathbb{P}_Q(q) \mu \beta_f(i, u) & \text{if } j = i + q \\ \frac{1}{\nu} \gamma i & \text{if } j = i - 1 \\ 1 - \frac{\mu \beta_f(i, u) + \gamma i}{\nu} & i = j \end{cases} \quad (69)$$

where  $\nu$  is selected<sup>6</sup> as in (36).

We now consider Problem 10 which is a discrete time formulation of Problem 6 for the SI model where bursts are considered.

**Problem 10** *We seek to solve the following problem*

$$J(i_0) = \min_{u \in \mathcal{F}} J_u(i_0) \quad (70)$$

where  $\mathcal{F}$  is the set of time invariant state feedback policies  $u(i)$ ,  $u : \mathbb{S} \rightarrow \mathcal{U}$ .  $J_u(i_0)$ , defined in (71), is the cost associated with the evolution of the uniformised Markov Chain  $I_k^q$  with transition probabilities defined in (69) from the initial condition  $i_0$  under a time invariant state feedback policy  $u$ .

$$J_u(i_0) = \lim_{N_d \rightarrow +\infty} \sum_{k=0}^{N_d-1} \mathbb{E} [g(I_k^q, u) | I_0 = i_0] \quad (71)$$

In order to derive Proposition 4 we consider the functions  $J_k^Q(i)$  and  $\mathcal{J}^Q(i, u)$  where for simplicity in the notation we remove the subscript from  $i_0$ . These are equivalent quantities to  $J_k(i)$  and  $\mathcal{J}_k(i, u)$  defined in Section 5.3.

We now make use of the Bellman equation for optimality and the value iteration algorithm [25, 57]. The value iteration algorithm associated with Problem 10 is

$$\begin{aligned} J_{k+1}^Q(i) &= \min_{u \in \mathcal{U}} [\mathcal{J}_k^Q(i, u)] \\ &= \frac{1}{\nu} \min_{u \in \mathcal{U}} [g_c(i, u) + \mu \beta_f(i, u) (\mathbb{E}_{\pi_Q} [J_k^Q(i + q)] - J_k^Q(i)) \\ &\quad - \gamma i L_k^Q(i - 1) + \nu J_k^Q(i)] \end{aligned} \quad (72)$$

In the last line of (72) we have defined<sup>7</sup> the quantity

$$L_k^Q(i) = J_k^Q(i + 1) - J_k^Q(i) \quad (73)$$

<sup>6</sup>It should be noted that the uniformisation factor computed for the case with bursts corresponds to the one for the SI model with no bursts. This follows by means of an analogous reasoning for the SI case with no bursts.

<sup>7</sup>We set  $\gamma i L_k^Q(i - 1) = 0$  for  $i = 0$  and  $\beta_f(i, u) (\mathbb{E}_{\pi_Q} [J_k^Q(i + q)] - J_k^Q(i)) = 0$  for  $i \leq N$ .

and the term  $\mathbb{E}_{\pi_Q} [J_k^Q(i+q)] = \sum_q [\mathbb{P}_Q(q) J_k^Q(i+q)]$  is the expectation with respect to the burst distribution  $\pi_Q$  introduced in Section 4.5.

It should be noted that Problem 10 is an infinite horizon optimal control problem with an absorbing state, positive costs, and with finite cardinality  $N_u$  of the mitigation measures  $\mathcal{U}$ . Therefore the results of Lemma 1 hold also for the case under consideration and for any initial condition  $J_0^Q$  the value iteration algorithm in (72) converges to optimal cost  $J^Q(i)$  that is the unique solution to the following Bellman Equation

$$\begin{aligned} J^Q(i) &= \min_{u \in \mathcal{U}} [\mathcal{J}^Q(i, u)] \\ &= \frac{1}{\nu} \min_{u \in \mathcal{U}} [g_c(i, u) + \mu \beta_f(i, u) (\mathbb{E}_{\pi_Q} [J^Q(i+q)] - J^Q(i)) \\ &\quad - \gamma i L^Q(i-1) + \nu J^Q(i)] \end{aligned} \quad (74)$$

where  $L^Q(i)$  denotes the quantity

$$L^Q(i) = J^Q(i+1) - J^Q(i) \quad (75)$$

Furthermore, the optimal policy  $u^*(i)$  is optimal if and only if it solves (74).

We now give various equivalent Lemmas to the ones of the previous sections for  $J_k^Q(i)$  to be positive, increasing and concave in the variable  $i \forall k \in \mathbb{Z}_{\geq}$ . We then show that these Lemmas lead to the result in Proposition 8, via an extended version stated as Proposition 6.

We begin by establishing in Lemma 5, analogously to Lemma 2, the positivity of the functions  $J_k^Q(i)$  via induction. In Lemma 6, an extension of Lemma 3 accounting for bursts, we make use of an induction argument and show that the functions  $\mathbb{E}_{\pi_Q} [J_k^Q(i+q) - J_k^Q(i)] \geq 0 \quad \forall k \in \mathbb{Z}_{\geq}$ . The results of Lemma 5 and 6 are used for Lemma 7, a version of Lemma 4 where bursts are considered, for which we show that  $(\mathbb{E}_{\pi_Q} [J_k^Q(i-1+q)] - J_k^Q(i)) - (\mathbb{E}_{\pi_Q} [J_k^Q(i-1+q)] - J_k^Q(i)) \geq 0, \forall k \in \mathbb{Z}_{\geq}$ .

We then show by using the results in the previous Lemmas that Proposition 8, an extended version of Proposition 6 when bursts are considered, follows from the previous Lemmas.

We begin by establishing the positivity for all  $i$  of  $J^Q(i)$  which is stated in the following Lemma.

**Lemma 5** *Consider Problem 10, the value iteration algorithm (72) and select  $J_0^Q(i)$  as in (53). If  $g_c(i, u)$  satisfies*

$$g_c(i, u) \geq 0, \quad \forall i \in \mathbb{S}, \forall u \in \mathcal{U} \quad (76)$$

*Then*

$$J_k^Q(i) \geq 0, \quad \forall k \in \mathbb{Z}_{\geq}, \forall i \in \mathbb{S} \quad (77)$$

*Proof* See Section A.7. □

The following Lemma shows that the functions  $\mathbb{E}_{\pi_Q} [J_k^Q(i+q)] - J_k^Q(i) \geq 0 \forall k \in \mathbb{Z}_{\geq}$ .

**Lemma 6** Consider Problem 10 and the value iteration algorithm (72). If the conditions of Lemma 2 are satisfied and if  $g_c(i, u)$  satisfies

$$\Delta_i^1[g_c(i, u)] \geq 0, \quad \forall i \in \mathbb{S}, \forall u \in \mathcal{U} \quad (78)$$

then

$$\mathbb{E}_{\pi_Q} [J_k^Q(i+q)] - J_k^Q(i) \geq 0, \quad \forall k \in \mathbb{Z}_{\geq}, \quad \forall i \in \{1, \dots, N - N_q - 1\} \quad (79)$$

*Proof* See Section A.8.  $\square$

The following lemma provides conditions for which  $\mathbb{E}_{\pi_Q} [J_k^Q(i-1+q)] - J_k^Q(i-1) - (\mathbb{E}_{\pi_Q} [J_k^Q(i+q)] - J_k^Q(i)) \geq 0, \quad \forall k \in \mathbb{Z}_{\geq}$

**Lemma 7** Consider Problem 10 and the value iteration algorithm (72). Assume the conditions of Lemma 6 and Lemma 5 satisfied.

If  $\beta_f$  satisfies

$$\Delta_i^2[\beta_f(i, u)] \leq 0, \quad \forall i \in \mathbb{S}, \forall u \in \mathcal{U} \quad (80)$$

and  $g_c(i, u)$  satisfies

$$\Delta_i^2[g_c(i, u)] \leq 0, \quad \forall i \in \mathbb{S}, \forall u \in \mathcal{U} \quad (81)$$

then

$$\begin{aligned} & \mathbb{E}_{\pi_Q} [J_k^Q(i-1+q)] - J_k^Q(i-1) \\ & - (\mathbb{E}_{\pi_Q} [J_k^Q(i+q)] - J_k^Q(i)) \geq 0, \quad \forall k \in \mathbb{Z}_{\geq} \\ & \forall i \in \{1, \dots, N - N_q - 1\} \end{aligned} \quad (82)$$

*Proof* See Section A.9.  $\square$

We now state our result showing that if the conditions of the previous Lemmas are satisfied then the optimal policy is non-increasing also if there are bursts in the number of infected.

**Proposition 8** Consider Problem 10. Assume the conditions in Lemma 6 and Lemma 7 satisfied.

If there exists a function  $t(i)$  where

$$t(i) : \mathbb{S} \rightarrow \mathbb{R}_{>} \quad (83)$$

such that  $\forall u^+, u^- \in \mathcal{U}$ , with  $u^+ \geq u^-$ .

$$\frac{t(i+1)}{t(i)} \leq \frac{\beta_f(i, u^-) - \beta_f(i, u^+)}{\beta_f(i+1, u^-) - \beta_f(i+1, u^+)} \quad (84)$$

and

$$\frac{t(i+1)}{t(i)} \geq \frac{g_c(i, u^+) - g_c(i, u^-)}{g_c(i+1, u^+) - g_c(i+1, u^-)} \quad (85)$$

then the optimal feedback policy  $u^*(i)$  satisfies

$$u^*(i+1) \leq u^*(i), \quad \forall i \in \mathbb{S} \quad (86)$$

*Proof* See Section A.10 □

Our result in Proposition 4 is a direct Corollary of Proposition 8.

*Proof of Proposition 4* We make use of the equivalent Problem 10. We then make use of Proposition 8 with  $t(i) = \frac{1}{i}$  and  $g_c(i, u)$  selected as in (9). Proposition 4 then follows directly. □

## Appendix A Proofs

### A.1 Proof of Lemma 2

*Proof* The proof is carried out by induction. In particular, we assume that at step  $k$ ,  $J_k(i) \geq 0$  and we seek to show that  $J_{k+1}(i)$  is non negative by expressing it as the sum of terms that are assumed non negative at step  $k$ . Let  $u_k^*(i)$  be the minimiser of  $\mathcal{J}_k(i, u)$  in (50) at step  $k$ . Let us rewrite (48) as follows

$$J_{k+1}(i) = g_c(i, u_k^*) + \gamma i J_k(i-1) + \mu \beta_f(i, u_k^*) J_k(i+1) + (\nu - \gamma i - \mu \beta_f(i, u_k^*)) J_k(i) \quad (\text{A1})$$

where we have made use of  $L_k(i) = J_k(i+1) - J_k(i)$  from (49).

We now show that the right hand side of (A1) is the sum of terms that are assumed non negative at step  $k$ . From the induction hypothesis we have that at step  $k$ ,  $J_k(i) \geq 0$ . The term  $g_c(i, u) \geq 0$  as per (54). By making use of (36) the term  $(\nu - \gamma i - \mu \beta_f(i, u))$  is non negative due to Proposition 5, i.e.  $\nu \geq \max_{i,u} [\mu \beta_f(i, u) + \gamma i]$ . The term  $\beta_f(i, u)$  is non negative as it is a transition probability. The terms  $\gamma$  and  $\mu$  are the parameters of the system and are assumed positive.

It follows that  $J_{k+1}(i)$  is non negative as it is equal to the sum of terms that are assumed non negative at step  $k$ . Therefore  $J_k(i) \geq 0, \forall k \in \mathbb{Z}_{\geq}$  as the initial condition is selected as (53), i.e.  $J_0(i) \geq 0$ .  $\square$

### A.2 Proof of Lemma 3

*Proof* We use an induction argument and show that the terms  $L_{k+1}(i)$  are greater than or equal the sum of terms assumed non negative at step  $k$ . Specifically, consider (49) and assume that at step  $k$ ,  $L_k(i) = J_k(i+1) - J_k(i) \geq 0$ . As specified in Lemma 2 we choose  $J_0(i)$  as in (53) and hence have  $L_0(i) = 0, \forall i$ .

Consider (48) then the following relation holds for  $J_{k+1}(i+1)$

$$J_{k+1}(i+1) = \frac{1}{\nu} [g_c(i+1, u_k^*(i+1)) + \mu \beta_f(i+1, u_k^*(i+1)) L_k(i+1) - \gamma(i+1) L_k(i) + \nu J_k(i+1)] \quad (\text{A2})$$

i.e. that  $\mathcal{J}_k(i+1, u)$  is minimised by selecting  $u_k^*(i+1)$ .

For  $J_{k+1}(i)$  we have

$$J_{k+1}(i) \leq \frac{1}{\nu} [g_c(i, u_k^*(i+1)) + \mu \beta_f(i, u_k^*(i+1)) L_k(i) - \gamma i L_k(i-1) + \nu J_k(i)] \quad (\text{A3})$$

where the left hand side of (A3), i.e.  $J_{k+1}(i)$  is the minimum cost of state  $i$  at step  $k+1$ . The right hand side of (A3) is the function  $\mathcal{J}_k(i, u)$  appearing in (48) and (50), evaluated in state  $i$  using as control input  $u_k^*(i+1)$  which is not the optimal value of  $u$  for state  $i$  at time step  $k$  and is therefore a quantity that is greater than or equal to  $J_{k+1}(i)$ .

We now take the difference of (A2), evaluated at state  $i+1$  using  $u_k^*(i+1)$  as control input, and (A3) yielding

$$\begin{aligned} L_{k+1}(i) &= J_{k+1}(i+1) - J_{k+1}(i) \\ &\geq \frac{1}{\nu} [g_c(i+1, u_k^*(i+1)) \\ &\quad + \mu \beta_f(i+1, u_k^*(i+1)) L_k(i+1) \\ &\quad - \gamma(i+1) L_k(i) + \nu J_k(i+1)] \\ &\quad - \frac{1}{\nu} [g_c(i, u_k^*(i+1)) + \mu \beta_f(i, u_k^*(i+1)) L_k(i) \\ &\quad - \gamma i L_k(i-1) + \nu J_k(i)] \end{aligned} \quad (\text{A4})$$



After rearranging the previous expression it follows that

$$\begin{aligned}
L_{k+1}(i) \geq & \frac{1}{\nu} [g_c(i+1, u_k^*(i+1)) - g_c(i, u_k^*(i+1)) \\
& + \mu\beta_f(i+1, u_k^*(i+1))L_k(i+1) \\
& + (\nu - \gamma(i+1))L_k(i) \\
& - \mu\beta_f(i, u_k^*(i+1))L_k(i) + \gamma i L_k(i-1)]
\end{aligned} \tag{A5}$$

By regrouping the terms in (A5) we obtain

$$\begin{aligned}
L_{k+1}(i) \geq & \frac{1}{\nu} [g_c(i+1, u_k^*(i+1)) - g_c(i, u_k^*(i+1)) \\
& + \mu\beta_f(i+1, u_k^*(i+1))L_k(i+1) \\
& + (\nu - \gamma(i+1) - \mu\beta_f(i, u_k^*(i+1)))L_k(i) \\
& + \gamma i L_k(i-1)]
\end{aligned} \tag{A6}$$

We now show that the left hand side of (A6) is greater than or equal to a sum of terms that are assumed non negative at step  $k$  and is therefore non negative. The terms  $L_k(i)$  are assumed non negative from the induction argument. By using (56) the summation of the terms involving the costs  $g_c$  are non negative  $\forall u \in \mathcal{U}$ . By using (36) the terms related to  $L_k(i+1)$  namely  $(\nu - \gamma(i+1) - \mu\beta_f(i, u_k^*(i+1)))$  are non negative. The term  $\mu\beta_f(i+1, u_k^*(i+1)) \geq 0, \forall i, \forall u \in \mathcal{U}$  as it is a transition probability.  $L_{k+1}$  is greater than or equal to a sum of terms that are non negative and therefore the function  $L_k(i) \geq 0, \forall k \in \mathbb{Z}_{\geq}$  by induction.  $\square$

### A.3 Proof of Lemma 4

*Proof* The proof is carried out by induction. Consider (49) at step  $k+1$ . We show that  $L_{k+1}(i-1) - L_{k+1}(i) \geq 0$ , if this property holds at step  $k$ , by showing that this quantity is greater than or equal to a sum of terms that are assumed non negative at step  $k$ .

Let us assume that at step  $k$ ,  $L_k(i-1) - L_k(i) \geq 0$ . We assume the conditions of Lemma 3 are satisfied and hence the terms  $L_k(i) \geq 0, \forall i$ . We denote with  $u_k^*(i)$  the value of  $u$  such that (48) is minimised at step  $k$  and state  $i$ .

We make use of (49) yielding  $L_{k+1}(i-1) = J_{k+1}(i) - J_{k+1}(i-1)$ . By using (48) we obtain the following inequality

$$\begin{aligned}
L_{k+1}(i-1) \geq & \frac{1}{\nu} [g_c(i, u_k^*(i)) + \mu\beta_f(i, u_k^*(i))L_k(i) \\
& - \gamma i L_k(i-1) + \nu J_k(i)] \\
& - \frac{1}{\nu} [g_c(i-1, u_k^*(i)) \\
& + \mu\beta_f(i-1, u_k^*(i))L_k(i-1) \\
& - \gamma(i-1)L_k(i-2) + \nu J_k(i-1)]
\end{aligned} \tag{A7}$$

By rearranging (A7) we obtain

$$\begin{aligned}
L_{k+1}(i-1) \geq & \frac{1}{\nu} [g_c(i, u_k^*(i)) - g_c(i-1, u_k^*(i)) \\
& + \mu\beta_f(i, u_k^*(i))L_k(i) \\
& + (\nu - \gamma i - \mu\beta_f(i-1, u_k^*(i)))L_k(i-1) \\
& + \gamma(i-1)L_k(i-2)]
\end{aligned} \tag{A8}$$

Specifically, the right hand side of (A8) is the difference of the minimised quantity  $J_{k+1}(i)$  and a quantity that is larger than  $J_{k+1}(i-1)$ . This quantity is  $\mathcal{J}_k(i-1, u_k^*(i))$  appearing in (48) and (50) which is not the minimised as it is evaluated at  $u_k^*(i)$ .

We now derive an inequality for  $L_{k+1}(i)$ . By means of an analogous reasoning to the one adopted for the derivation of (A8) it follows that  $J_k(i+1) \leq \frac{1}{\nu}[g_c(i+1, u_k^*(i)) + \mu\beta_f(i+1, u_k^*(i))L_k(i+1) - \gamma(i+1)L_k(i) + \nu J_k(i+1)]$ . By making use of this inequality, (48) and the definition of  $L_{k+1}(i) = J_{k+1}(i+1) - J_{k+1}(i)$  yields

$$\begin{aligned} L_{k+1}(i) &\leq \frac{1}{\nu}[g_c(i+1, u_k^*(i)) \\ &\quad + \mu\beta_f(i+1, u_k^*(i))L_k(i+1) \\ &\quad - \gamma(i+1)L_k(i) + \nu J_k(i+1)] \\ &\quad - \frac{1}{\nu}[g_c(i, u_k^*(i)) + \mu\beta_f(i, u_k^*(i))L_k(i) \\ &\quad - \gamma i L_k(i-1) + \nu J(i)] \end{aligned} \quad (\text{A9})$$

By rearranging the previous equation we have

$$\begin{aligned} L_{k+1}(i) &\leq \frac{1}{\nu}[g_c(i+1, u_k^*(i)) - g_c(i, u_k^*(i)) \\ &\quad + \mu\beta_f(i+1, u_k^*(i))L_k(i+1) \\ &\quad + (\nu - \gamma(i+1) - \mu\beta_f(i, u_k^*(i)))L_k(i) \\ &\quad + \gamma i L_k(i-1)] \end{aligned} \quad (\text{A10})$$

By making use of the inequalities for  $L_{k+1}(i-1)$  and for  $L_{k+1}(i)$ , namely (A8) and (A10) we obtain the following inequality

$$\begin{aligned} L_{k+1}(i-1) - L_{k+1}(i) &\geq \\ &\quad \frac{1}{\nu}[g_c(i, u_k^*(i)) - g_c(i-1, u_k^*(i)) \\ &\quad + \mu\beta_f(i, u_k^*(i))L_k(i) \\ &\quad + (\nu - \gamma i - \mu\beta_f(i-1, u_k^*(i)))L_k(i-1) \\ &\quad + \gamma(i-1)L_k(i-2)] \\ &\quad - \frac{1}{\nu}[g_c(i+1, u_k^*(i)) - g_c(i, u_k^*(i)) \\ &\quad + \mu\beta_f(i+1, u_k^*(i))L_k(i+1) \\ &\quad + (\nu - \gamma(i+1) - \mu\beta_f(i, u_k^*(i)))L_k(i) \\ &\quad + \gamma i L_k(i-1)] \end{aligned} \quad (\text{A11})$$

After rearranging the previous expression it follows that

$$\begin{aligned} L_{k+1}(i-1) - L_{k+1}(i) &\geq \\ &\quad \frac{1}{\nu}[2g_c(i, u_k^*(i)) - g_c(i+1, u_k^*(i)) - g_c(i-1, u_k^*(i)) \\ &\quad + \nu(L_k(i-1) - L_k(i)) \\ &\quad + \gamma(i-1)L_k(i-2) \\ &\quad - (\mu\beta_f(i-1, u_k^*(i)) + 2\gamma i)L_k(i-1) \\ &\quad + (2\mu\beta_f(i, u_k^*(i)) + \gamma(i+1))L_k(i) \\ &\quad - \mu\beta_f(i+1, u_k^*(i))L_k(i+1)] \end{aligned} \quad (\text{A12})$$

We now make use of the induction hypothesis, *i.e.*  $L_k(i-2) \geq L_k(i-1)$ , leading to

$$\begin{aligned}
& L_{k+1}(i-1) - L_{k+1}(i) \geq \\
& \frac{1}{\nu} [2g_c(i, u_k^*(i)) - g_c(i+1, u_k^*(i)) - g_c(i-1, u_k^*(i))] \\
& + \nu(L_k(i-1) - L_k(i)) \\
& + (\gamma(i-1) - 2\gamma i)L_k(i-1) + \gamma(i+1)L_k(i) \\
& - \mu\beta_f(i-1, u_k^*(i))L_k(i-1) \\
& + 2\mu\beta_f(i, u_k^*(i))L_k(i) \\
& - \mu\beta_f(i+1, u_k^*(i))L_k(i+1)]
\end{aligned} \tag{A13}$$

By making use of the induction hypothesis again we have

$$\begin{aligned}
& L_{k+1}(i-1) - L_{k+1}(i) \geq \\
& \frac{1}{\nu} [2g_c(i, u_k^*(i)) - g_c(i+1, u_k^*(i)) - g_c(i-1, u_k^*(i))] \\
& + \nu(L_k(i-1) - L_k(i)) \\
& + (\gamma(i-1) - 2\gamma i - \mu\beta_f(i-1, u_k^*(i)))L_k(i-1) \\
& - (\mu\beta_f(i+1, u_k^*(i)) - 2\mu\beta_f(i, u_k^*(i)) - \gamma(i+1))L_k(i)
\end{aligned} \tag{A14}$$

After rearranging the terms we obtain

$$\begin{aligned}
& L_{k+1}(i-1) - L_{k+1}(i) \geq \\
& \frac{1}{\nu} [2g_c(i, u_k^*(i)) - g_c(i+1, u_k^*(i)) - g_c(i-1, u_k^*(i))] \\
& + (\nu - \gamma(i+1) - \mu\beta_f(i-1, u_k^*(i)))L_k(i-1) \\
& - (\nu - 2\mu\beta_f(i, u_k^*(i)) - \gamma(i+1) + \\
& \quad + \mu\beta_f(i+1, u_k^*(i)))L_k(i)]
\end{aligned} \tag{A15}$$

In order for the previous expression to be non negative its sufficient for two conditions to be satisfied.

The first condition is related to the costs  $g_c(i, u)$ . The summation of the term involving the cost function are non negative since  $g_c(i, u)$  satisfies

$$2g_c(i, u) - g_c(i+1, u) - g_c(i-1, u) \geq 0, \forall u \in \mathcal{U} \tag{A16}$$

which after some manipulation can be equivalently expressed as (59), *i.e.*

$$\Delta_i^2[g_c(i, u)] \leq 0, \forall u \in \mathcal{U} \tag{A17}$$

The second condition is related to the terms involving  $L_k(i-1)$  and  $L_k(i)$ . Specifically, it is sufficient for the following equation to be satisfied

$$\begin{aligned}
& + (\nu - \gamma(i+1) - \mu\beta_f(i-1, u_k^*(i)))L_k(i-1) \\
& - (\nu - 2\mu\beta_f(i, u_k^*(i)) - \gamma(i+1) + \mu\beta_f(i+1, u_k^*(i)))L_k(i) \geq 0
\end{aligned} \tag{A18}$$

Note that the conditions in Lemma 3 are assumed satisfied, therefore (57) holds and hence the terms  $L_k(i-1) \geq 0$  and  $L_k(i) \geq 0, \forall k \in \mathbb{Z}_{\geq}$ . To show that (A18) is satisfied it suffices to show that (A19) is satisfied since due to (36) we have that  $(\nu - \gamma(i+1) - \mu\beta_f(i-1, u_k^*(i))) \geq 0$  and  $(\nu - 2\mu\beta_f(i, u_k^*(i)) - \gamma(i+1) + \mu\beta_f(i+1, u_k^*(i))) \geq 0$  yielding

$$\begin{aligned}
& - \gamma(i+1) - \mu\beta_f(i-1, u_k^*(i)) \geq \\
& - 2\mu\beta_f(i, u_k^*(i)) - \gamma(i+1) + \mu\beta_f(i+1, u_k^*(i))
\end{aligned} \tag{A19}$$

By simplifying the terms related to  $\gamma$  it follows that the previous equation may be expressed as

$$2\mu\beta_f(i, u_k^*(i)) - \mu\beta_f(i+1, u_k^*(i)) - \mu\beta_f(i-1, u_k^*(i)) \geq 0 \quad (\text{A20})$$

which after rearranging can be expressed as

$$\Delta_i^2[\beta_f(i, u)] \leq 0, \forall u \in \mathcal{U} \quad (\text{A21})$$

that is (58). It follows by induction that  $L_k(i-1) - L_k(i) \geq 0 \quad \forall k \in \mathbb{Z}_{\geq}$ .  $\square$

#### A.4 Proof of Proposition 6

*Proof* We prove this Proposition by contradiction. We negate (64) and consider a  $t(i) : \mathbb{S} \rightarrow \mathbb{R}_{\geq}$  such that (63) holds. We then show that (62) does not hold leading to a contradiction.

For the proof we make use of the Bellman equation (51) that is satisfied by any optimal policy. Let us denote with  $\mathcal{J}(i, u)$  the function to be minimised on the right hand side of (51), i.e.

$$\mathcal{J}(i, u) := g_c(i, u) + \mu\beta_f(i, u)L(i) - \gamma iL(i-1) + \nu J(i) \quad (\text{A22})$$

Let us denote for some  $i$   $u^*(i+1)$  and  $u^*(i)$  as  $u^+$  and  $u^-$  respectively. By negating (64) we have

$$\exists i : u^*(i+1) > u^*(i) \quad (\text{A23})$$

or equivalently  $u^+ > u^-$ .

By making use of (51), the definition of  $\mathcal{J}(i, u)$  in (A22) and the definition of  $u^+, u^-$  the following two equations hold

$$\begin{aligned} J(i) &= \mathcal{J}(i, u^-) \leq \mathcal{J}(i, u^+) \\ J(i+1) &= \mathcal{J}(i+1, u^+) \leq \mathcal{J}(i+1, u^-) \end{aligned} \quad (\text{A24})$$

which by using the definition of  $\mathcal{J}(i, u)$  in (A22) yields

$$g_c(i, u^+) - g_c(i, u^-) \geq L(i)[\mu\beta_f(i, u^-) - \mu\beta_f(i, u^+)] \quad (\text{A25})$$

and

$$g_c(i+1, u^+) - g_c(i+1, u^-) \leq L(i+1)[\mu\beta_f(i+1, u^-) - \mu\beta_f(i+1, u^+)] \quad (\text{A26})$$

Consider  $t(i) > 0$  as in (61) and since we are assuming  $u^+ > u^-$ , by using (63) we have

$$[g_c(i+1, u^+) - g_c(i+1, u^-)]t(i+1) \geq [g_c(i, u^+) - g_c(i, u^-)]t(i) \quad (\text{A27})$$

We multiply (A25) by  $t(i)$  and (A26) by  $t(i+1)$  yielding

$$[g_c(i, u^+) - g_c(i, u^-)]t(i) \geq L(i)[\mu\beta_f(i, u^-) - \mu\beta_f(i, u^+)]t(i) \quad (\text{A28})$$

and

$$t(i+1)[g_c(i+1, u^+) - g_c(i+1, u^-)] \leq L(i+1)[\mu\beta_f(i+1, u^-) - \mu\beta_f(i+1, u^+)]t(i+1) \quad (\text{A29})$$

By making use of the previous two equations and (A27) we obtain after rearranging

$$L(i)[\mu\beta_f(i, u^+) - \mu\beta_f(i, u^-)]t(i) - L(i+1)[\mu\beta_f(i+1, u^+) - \mu\beta_f(i+1, u^-)]t(i+1) \geq 0 \quad (\text{A30})$$

Note that the properties stated in Lemmas 2, 3 and 4 for  $J_k(i)$  and  $L_k(i)$  are satisfied also by  $J(i)$  and  $L(i)$ , respectively, since  $J_k(i) \rightarrow J(i)$ , as stated in Lemma 1. Therefore we have  $L(i) - L(i+1) \geq 0$  and  $L(i) \geq 0, \forall i$  and hence we obtain that for the previous equation to be satisfied

$$[\beta_f(i, u^-) - \beta_f(i, u^+)]t(i) \leq [\beta_f(i+1, u^-) - \beta_f(i+1, u^+)]t(i+1) \quad (\text{A31})$$

which contradicts (62).  $\square$

## A.5 Proof of Proposition 2

*Proof* Consider (62) and (63) from Proposition 6. Let us make use of (62) when  $\beta_f(i, u) = \frac{i}{N}(N - i)$ . We obtain that  $t(i)$  has to satisfy

$$\frac{t(i+1)}{t(i)} \leq \frac{i(N-i)}{(i+1)(N-i-1)} \quad (\text{A32})$$

Considering (63) particularised to the case where  $g_c(i, u)$  is selected as (11) we obtain the  $t(i)$  has to also satisfy

$$\frac{t(i+1)}{t(i)} \geq \frac{c_2 i + c_4 N}{c_2(i+1) + c_4 N} \quad (\text{A33})$$

We make use of conditions in (A33) and (A32) in order to establish if there exists a function  $t(i)$  such that (61) is satisfied and therefore Proposition 6 holds. This leads to

$$\frac{c_2 i + c_4 N}{c_2(i+1) + c_4 N} \leq \frac{i(N-i)}{(i+1)(N-i-1)} \quad (\text{A34})$$

By manipulating (A34) we obtain

$$\frac{c_2 i + c_4 N}{i(N-i)} \leq \frac{c_2(i+1) + c_4 N}{i(N-i) + N - 2i - 1} \quad (\text{A35})$$

We proceed to simplify (A34) as follows

$$\begin{aligned} \frac{c_2 i + c_4 N}{c_2(i+1) + c_4 N} &\leq \frac{i(N-i)}{(i+1)(N-i-1)} \\ (c_2 i + c_4 N)(i+1)(N-i-1) &\leq (c_2(i+1) + c_4 N)i(N-i) \\ c_2 i(N-i) &\geq (c_2 i + c_4 N)(N-2i-1) \\ c_2 i(N-i) - (c_2 i + c_4 N)(N-2i-1) &\geq 0 \\ -c_2 i^2 + 2c_2 i^2 + c_2 i - c_4 N(N-2i-1) &\geq 0 \\ c_2 i^2 + i(c_2 + 2c_4 N) - c_4 N(N-1) &\geq 0 \\ i &\geq -\frac{c_2 + 2c_4 N}{2c_2} + \sqrt{\left(\frac{c_2 + 2c_4 N}{2c_2}\right)^2 + \frac{c_4 N}{c_2}(N-1)} \\ i &\geq -\frac{c_2 + 2c_4 N}{2c_2} + \sqrt{\frac{c_2^2 + 4(c_4 N)^2 + 4c_2 c_4 N^2}{4c_2^2}} \end{aligned} \quad (\text{A36})$$

Let us define

$$\bar{i} = -\frac{c_2 + 2c_4 N}{2c_2} + \sqrt{\frac{c_2^2 + 4c_4^2 N^2 + 4c_2 c_4 N^2}{4c_2^2}} \quad (\text{A37})$$

By selecting  $\chi = c_2/c_4$  it follows that (A37) can be rewritten as

$$\bar{i} = -\frac{\chi + 2N}{2\chi} + \sqrt{\frac{\chi^2 + 4\chi N^2 + 4N^2}{4\chi^2}} \quad (\text{A38})$$

By making use of (A38) and (A36) it follows that (61) is satisfied  $\forall i \geq \bar{i}$ . We now make use of Proposition 6 leading to the following inequality

$$u^*(i+i) \leq u^*(i) \quad \forall i \geq \bar{i} \quad (\text{A39})$$

□

## A.6 Proof of Proposition 5

*Proof* The Proposition follows from a procedure known as *uniformization* which is described in e.g. [25] and [58]. In particular, the parameter  $\nu$  used in the definition of the discrete time process described in Problem 8 needs to satisfy [25] and [58]

$$\nu \geq \max_{s,i,u} \left[ \frac{\mu}{N} si \cdot h(u) + \gamma i \right] \quad (\text{A40})$$

subject to the constraint  $s + i = N$ . □

## A.7 Sketch Proof of Lemma 5

*Proof* We follow an analogous argument to the one adopted for the proof of Lemma 2 in Section A.1.

Let us rewrite  $\mathcal{J}_k^Q(i, u)$  in (72) as

$$\mathcal{J}_k^Q(i, u) = g_c(i, u) + \gamma i J_k^Q(i-1) + \mu \beta_f(i, u) \mathbb{E}_{\pi_Q} \left[ J_k^Q(i+q) \right] + (\nu - \gamma i - \mu \beta_f(i, u)) J_k^Q(i) \quad (\text{A41})$$

using (72) yields

$$\begin{aligned} J_{k+1}^Q(i) &= \min_{u \in \mathcal{U}} [g(i, u) \\ &\quad + \gamma i J_k^Q(i-1) + \mu \beta_f(i, u) \mathbb{E}_{\pi_Q} \left[ J_k^Q(i+q) \right] \\ &\quad + (\nu - \gamma i - \mu \beta_f(i, u)) J_k^Q(i)] \end{aligned} \quad (\text{A42})$$

By means of a similar induction argument as the one adopted in Section A.1, particularising the results of Proposition 5 to the case under consideration, and supposing that  $J_k^Q(i) \geq 0, \mathbb{E}_{\pi_Q} \left[ J_k^Q(i+q) \right] \geq 0$  it is straight forward to show using (A42) that  $J_k^Q(i)$  is non-negative if the initial condition  $J_0^Q(i)$  is selected as in (53). □

## A.8 Sketch Proof of Lemma 6

*Proof* We make use of induction following a similar argument to the one adopted in Section A.8 for the proof of Lemma 6. We seek to show by induction that  $\mathbb{E}_{\pi_Q} \left[ J_{k+1}^Q(i+q) \right] - J_{k+1}^Q(i) \geq 0$  and we suppose that the same expression holds at step  $k$ . As specified in Lemma 5 we choose  $J_0^Q(i)$  as in (53).

We rearrange  $\mathbb{E}_{\pi_Q} \left[ J_{k+1}^Q(i+q) \right] - J_{k+1}^Q(i) \geq 0$  as follows

$$\begin{aligned} \sum_{q=1}^{N_q} \mathbb{P}_Q(q) J_{k+1}^Q(i+q) - \sum_{q=1}^{N_q} \mathbb{P}_Q(q) J_{k+1}^Q(i) &\geq 0 \\ \sum_{q=1}^{N_q} \mathbb{P}_Q(q) [J_{k+1}^Q(i+q) - J_{k+1}^Q(i)] &\geq 0 \end{aligned} \quad (\text{A43})$$

Note that by expanding the summation in the last line the equation is satisfied if  $J_{k+1}^Q(i+1) - J_{k+1}^Q(i) \geq 0, \forall i \in \mathbb{S}$  and by making use of the property of p.m.f.s that  $\mathbb{P}_Q(q) \geq 0, \forall q \in \mathbb{Q}$ .

In order to show (79) it is thus sufficient to show that  $L_{k+1}^Q(i) = J_{k+1}^Q(i+1) - J_{k+1}^Q(i) \geq 0$ . By making use of a similar induction argument to the one used in Section A.8 it is possible to show that (79) is satisfied. □

## A.9 Sketch Proof of Lemma 7

*Proof* We make use of an induction argument similar to the one adopted in Section A.3 for Lemma 4.

In order to show that (82) is satisfied we make use of induction and we seek to show that  $\mathbb{E}_{\pi_Q} [J_{k+1}^Q(i-1+q)] - J_{k+1}^Q(i-1) - (\mathbb{E}_{\pi_Q} [J_{k+1}^Q(i+q)] - J_{k+1}^Q(i)) \geq 0$  if the same equality holds at step  $k$ . By rearranging the previous expression we obtain

$$\mathbb{E}_{\pi_Q} [J_{k+1}^Q(i-1+q) - J_{k+1}^Q(i+q)] - (J_{k+1}^Q(i-1) - J_{k+1}^Q(i)) \geq 0 \quad (\text{A44})$$

The previous expression leads to

$$\mathbb{E}_{\pi_Q} [L_{k+1}^Q(i-1) - L_{k+1}^Q(i-1+q)] \geq 0 \quad (\text{A45})$$

or equivalently

$$\sum_{q=1}^{N_q} \mathbb{P}_Q(q) [L_{k+1}^Q(i-1) - L_{k+1}^Q(i-1+q)] \geq 0 \quad (\text{A46})$$

Note that (A46) is verified as long as  $L_{k+1}^Q(i-1) - L_{k+1}^Q(i) \geq 0 \forall i$  is verified and by using the property of p.m.f.s, *i.e.*  $\mathbb{P}_Q(q) \geq 0, \forall q \in \mathbb{Q}$ .

By making use of an induction argument similar to the one adopted in Section A.3 it is possible to show that  $L_k^Q(i-1) - L_k^Q(i) \geq 0 \forall k \in \mathbb{Z}_{\geq}$ . Thus we obtain that  $\mathbb{E}_{\pi_Q} [J_k^Q(i-1+q)] - J_k^Q(i-1) - (\mathbb{E}_{\pi_Q} [J_k^Q(i+q)] - J_k^Q(i)) \geq 0, \forall k \in \mathbb{Z}_{\geq}$ .  $\square$

## A.10 Sketch Proof of Proposition 8

*Proof* We prove this Proposition by contradiction using a similar method as the one adopted for Proposition 6. In particular as the conditions of Lemma 6 and Lemma 7 are supposed verified we make use of the method adopted in Section A.4 particularised to the value iteration algorithm equation accounting for bursts, *i.e.* (72). Specifically, we negate (86) and we consider a  $t(i)$  such that for some  $i$  the condition in (85) holds. After some manipulation this leads to contradict (84).  $\square$

## A.11 Value Iteration algorithm for non-increasing policies

If a MDP is known to have policies that are non-increasing with respect to its state, one may use the Algorithm 1 from [24], reported here to facilitate readability.

Consider a MDP where the state is defined on  $\mathbb{S} = \{0, \dots, N\}$  and the set of control actions is  $\mathcal{U} = \{u_1, \dots, u_{N_u}\}$  where  $u_i < u_j, \forall j > i$ . Let us denote with  $\mathcal{J}_k(i, u)$  the function to be minimised at step  $k$  of the DP algorithm and let us denote with  $J_k(i)$  the value function at step  $k$  of the DP algorithm. If such a MDP is known to have non-increasing policies with respect to the state then the following algorithm can be used to find an optimal policy. The algorithm reduces considerably the computational effort with respect to the value iteration algorithm. This is accomplished by reducing the set of possible minimisers for increasing values of the state in line 11.

## Appendix B Additional figures and discussion

In this section we provide additional figures and discussion relating to various sections of the manuscript.

---

**Algorithm 1** Monotone algorithm

---

```
1: Set  $\epsilon \ll 1$ 
2: while  $|J_{k+1}(i) - J_k(i)| > \epsilon$  do
3:   Set  $\mathcal{U} = \{u_1, \dots, u_{N_u}\}$ 
4:   for  $i = 0 : N$  do
5:     Calculate  $J_{k+1} = \min_{\mathcal{U}} \mathcal{J}_k(i, u)$ 
6:     Calculate  $u^*(i) = \operatorname{argmin}_{\mathcal{U}} \mathcal{J}_k(i, u)$ 
7:     Set  $u_\ell = u^*(i)$   $\triangleright \ell \in \{1, \dots, N_u\}$ 
8:     if  $i = N$  then
9:       return
10:    else
11:       $\mathcal{U} = \{u_1, \dots, u_\ell\}$ 
12:    end if
13:  end for
14: end while
```

---

### B.1 Examples and discussion for the control to transmission rate function $h(u)$ and the cost function $z(u)$

In this section we provide some relevant examples of the functions  $h(u)$  and  $z(u)$  used in the formulation of the epidemic models in Section 2. We also provide examples illustrating how these relate to optimal policies, and examples that demonstrate that our results hold irrespectively of Assumption 1.

We would like to note that functions  $h(u)$  and  $z(u)$ , and in particular their relative form, affect the optimal policies.

The intervention to transmission rate function  $h(u)$  is a frequently used modelling formulation to relate a known set of interventions  $\mathcal{U}$  to reductions of the transmission rate of the epidemic and is also a convenient formalism when such relation has to be inferred. Especially for novel pathogens  $h(u)$  is difficult to assess [11] and is subject to high uncertainty [59]. Settings frequently considered in the literature include  $h(u) = (1 - q_{eff}u)$  [45] and quadratic functions  $h(u) = (1 - q_{eff}u)^2$  [27], where  $q_{eff} \in [0, 1]$  captures the effectiveness of contact tracing and of the interventions [60].

It should also be noted, as discussed in Remark 5, that a particular  $h$  can lead to the impossibility of reaching values of  $\mathcal{R}^* < 1$  for which infection levels are expected to decrease [20]. This can occur for low values  $q_{eff}$ , or if  $q_{eff} = 1$  but the available interventions  $\mathcal{U}$  are not sufficient to yield  $\mathcal{R} \leq 1$ .

In Fig. B1 we show two examples of  $h(u)$  and intervention cost functions  $z(u)$  as well as their effects on the optimal policies for costs as in (9). Fig B1(a) shows two examples of  $h$ :  $h(u) = (1 - u)$  (—) and  $h(u) = (1 - u)^2$  (—) and in Fig. B1(b) we display  $z(u) = u$  (—) for the mitigation measures  $u \in \mathcal{U}$  with  $\mathcal{U} = \{0, 0.04, \dots, 1\}$ . In these cases for increasingly restrictive interventions, the transmission rate is non-increasing and costs are non-decreasing. In Fig. B1(e) we show the optimal policies for the SI epidemic in Problem 2 computed for  $h(u) = (1 - u)$  (—) and  $h(u) = (1 - u)^2$  (—). It should be noted that linear functions  $h(u) = (1 - u)$  yield rapid variations of the optimal policies. Quadratic  $h$  of the form  $h(u) = (1 - u)^2$ , that model rapid reductions



of the transmission rate for moderate interventions, yield more gradual changes of the policies.

In Fig. B1(c) and Fig. B1(d) we illustrate the functions  $h(u^*(i))$  and  $z(u^*(i))$  as a function of the infection levels  $i$  when the optimal policies displayed in Fig. B1(e) are considered<sup>8</sup>. The diagrams show, as discussed in Remark 1, that in an optimal policy the transmission rate is non-decreasing with infection levels and that if  $h$  is nonlinear this increase can be gradual

In Fig. B2 we illustrate via a representative example that the form of the optimal policies depends upon the relation between  $z(u)$  and  $h(u)$ . In particular, the effects of an arbitrary  $h(u)$  can be quantified equivalently by considering an appropriate transformation of the intervention cost  $\tilde{z}(u) = z(h^{-1}(u))$  and  $\tilde{h}(u) = u$ . It follows as discussed in Remark 3 that our results hold irrespectively of Assumption 1. In particular via this transformation functions  $h$  that do not satisfy Assumption 1 can be incorporated in function  $z(\cdot)$  in the costs, for which the only restriction is non negativity. Fig. B2(a) shows  $h(u) = 1 - u$  satisfying Assumption 1 and Fig. B2(b) displays a linear cost function  $z(u) = u$ . An equivalent formulation can be obtained by considering  $\tilde{h}(u) = u$ , shown in Fig. B2(c), and  $\tilde{z}(u) = 1 - u$ , shown Fig. B2(d). This formulation leaves the results unaffected as the relationship between the two functions is unchanged. In particular, note that  $\tilde{h}(u)$  does not satisfy Assumption 1, but  $\tilde{z}(u)$  satisfies the assumptions of an analogous version of Proposition 7. It follows that similar conclusions to those of Proposition 7 can be derived where the optimal policies  $\tilde{u}^*(i)$  are however non-decreasing. We show the optimal policies  $u^*(i)$  and  $\tilde{u}^*(i)$  associated with the two formulations in Fig. B2(g). The formulation with  $h(u) = 1 - u$  shows non-increasing optimal policies while if the non-decreasing  $\tilde{h}(u) = u$  is considered, the optimal policy is non-decreasing due to the effect of the increasing  $\tilde{h}(u)$  upon the transmission of the disease. Fig. B2(e) and Fig. B2(f) show that under an optimal policy the controlled transmission rate of the disease is in both settings non-decreasing with respect to the prevalence levels.

We have verified that analogous conclusions hold also for more complex epidemics and for nonlinear  $h(u)$ .

## B.2 Additional figures and optimal policies for the SIR epidemic

### B.2.1 Additional optimal policies for the SIR model

In Fig. B3 we display optimal policies for the SIR epidemic of Problem 1 with costs  $g_c(u)$  as in (9) when interventions cannot reduce the controlled  $\mathcal{R}$  to values lower than 1. This is a relevant case when pharmaceutical interventions and vaccines are in development and the transmission mitigation interventions are required in order to try to suppress in an efficient way the spread of the disease. Differently from the representative optimal policies shown in Fig. S1 we select  $h(u)$  to be  $h = (1 - q_{eff}u)^2$ , a set of interventions  $\mathcal{U} = \{0, 0.05, \dots 0.4\}$  and  $q_{eff} = 0.5$ . This setting captures what occurs for common flu: the interventions can partially reduce the transmission of the disease, the effect on the transmission rate is nonlinear, and the effectiveness of the

---

<sup>8</sup>Note that  $\mathcal{R}^*$  defined in (1) corresponds to  $h(u^*(i))$  scaled by  $\mathcal{R}_0$

measures is low. This does not lead to values of  $\mathcal{R} < 1$  for which the expected levels decline and as discussed in Remark 5 can be considered in our formulation.

The reproduction numbers  $\mathcal{R}^*$  in Fig. B3 are analogous to the ones in Fig. S1 where the effects of the interventions are linear  $h(u) = 1 - u$ . The optimal policies in this case are non-increasing and are predominantly constant for low values of prevalence yielding increasing values of  $\mathcal{R}^*$ . A negative feedback scheme on the infections is therefore not optimal as for increasing levels of infection in an optimal policy there is no incentive to make use of stricter interventions.

In Fig. B4 and Fig. B5 we display the optimal policies for the SIR epidemic for  $\mathcal{R}_0 = \{1.6, 3.5\}$  for three values of  $\zeta$  and for three choices of cost functions  $z(u)$  when  $h(u) = 1 - u$ . The figures show that for all the selected cases feedback policies are not sensitive to changes of infection prevalence as  $\mathcal{R}^*$  is constant and increases to  $\mathcal{R}_0$  for increasing prevalence. In the optimal policies increasingly restrictive mitigation measures are not associated with increasing levels of infection. It should be noted that similarly to the SI epidemic model discussed in the previous section if the relationship between  $z$  and  $h$  is non linear the interventions are relaxed more gradually when compared to linear settings.

### B.2.2 Optimal policies for the SIR model with stochastic infection outcomes

In Fig. B6 we compute the optimal policies associated with Problem 5 with costs  $g_c(i, u) = \zeta i u + i$  and distribution  $\pi_Q \sim \mathcal{U}$  for two different supports. The results show that in an optimal policy there is no incentive to make use of negative feedback schemes to tame the epidemic irrespectively of the presence of stochastic infection outcomes. The diagrams show that increasing expected values of  $\pi_Q$  lead to more conservative policies. The optimal policies are also in line with Proposition 4 for the SI model (Section 4.5).

### B.2.3 Additional time simulations for the SIR models

In Fig. B7(a) and B7(b) we select  $h(u) = 1 - q_{eff}$  and the effectiveness  $q_{eff}$  of the interventions close to the mid range found for the COVID-19 pandemic in the United States of America [41] *i.e.*  $q_{eff} = 0.5$ . The parameter  $q_{eff}$  is such that  $\mathcal{R}$  cannot be lower than 1, *i.e.* the value of  $\mathcal{R}$  for which the expected infection levels decrease, as discussed in Remark 5. In Fig. B7(a) the suboptimal negative feedback laws (---, ·····) show a significant peak of infection even after the interventions are used. This is due to the inability of the interventions to reduce  $\mathcal{R}$  to values lower than one and thus halt the initial exponential growth. Nonetheless, similarly to Fig. S2(a), enacting the interventions after some time reduces the levels of peak infection prevalence. The infection peak appears also for the optimal feedback law (—) but it is not as significant as for the suboptimal negative feedback case.

## B.3 Optimal policies for SI model

In this Section we compute the optimal policies for the SI model of Problem 2. In Fig. B8 we numerically compute the optimal policies for Problem 1 with costs  $g_c(i, u) =$

$\zeta i u + i$ . The optimal policy  $u^*(i)$  is shown with respect to the prevalence  $i/N$  and takes a value of 0 when no measures are selected and is positive for transmission mitigation measures. The optimal policy is in line with the result in Proposition 1, *i.e.* it is non-increasing with prevalence, which verifies the fact that optimal policies are not sensitive to prevalence as the controlled infection rate is increased for increasing  $i/N$ . The optimal policies in Diagram B8(a) and B8(b) are also constant for low values of  $i/N$  and decrease rapidly for larger values of  $i/N$ . The policies shown in Diagram B8(b) decrease more gradually with respect to the ones appearing in Diagram B8(a) due to the different selection of  $h(u)$ . It should be noted that nonlinear relations between costs and transmission rates lead to gradual increases and decreases of the policies. Linear relations as show in Fig.B10, lead to abrupt variation of the policies with respect to infection prevalence.

In Fig. B9 we compute the ratio of the suboptimal costs  $J_u^c(i)$  defined in (13), associated with the suboptimal negative feedback policy (22) and the optimal total expected cost  $J^c(i)$  defined in (12). The diagrams are consistent with the results of Proposition 1, *i.e.* the use of negative feedback strategies are suboptimal for costs of the form in (9) and yield higher total costs. In particular, in diagram B9(a) for increasing values of the threshold  $i_{th}$  the total expected costs often increase in particular for low values of  $i$ . In diagram B9(b) the cost configuration  $\zeta = 6$  is such that the optimal strategy is not to make use of mitigation measures. For this cost configuration, using negative feedback yields higher costs especially for  $i_{th} \geq 3$  and for  $i \geq 10$ . As shown in diagrams B9(c) and B9(d) for different values of  $c_2$  and  $c_3$ , negative feedback strategies yield costs that are several times higher than the constant policies. Analogous results have also been observed for other choices of parameters, costs and transmission functions.

In Fig. B10 we consider the case where linear variations in the disease transmission have a corresponding linear variation in costs, *i.e.* when  $g_c(i, u) = \zeta i u + i$  and  $h(u) = 1 - u$ . In this setting the optimal policies  $u^*(i)$  are also non-increasing and validate Proposition 1. In particular, we observe that the optimal policies abruptly decrease to 0 from a constant value after a threshold  $\hat{i}$ . The value of  $\hat{i}$  depends upon the values of the parameters  $\zeta$  as shown in Fig. B10.

In Fig. B11 we provide numerical computations of optimal policies corresponding to Proposition 2 *i.e.* for  $g_c$  as in (11). We compute numerically the optimal policies for increasing  $c_4$  values and in particular we select  $c_2 \approx 0$ , a setting of practical relevance as discussed in Section 4.1.1, and we select  $h(u) = (1 - u)^2$ . Fig. B11 shows that similarly to case where the cost function is an in (9) the optimal policy is non-increasing for low values of  $\chi = c_2/c_4$ . For increasing values of  $c_4$  varying interventions for increasing levels of prevalence can be beneficial, as shown in the top part of the figure where the optimal policies gradually increase to more strict interventions.

## References

- [1] Bin, M., Cheung, P.Y.K., Crisostomi, E., Ferraro, P., Lhachemi, H., Murray-Smith, R., Myant, C., Parisini, T., Shorten, R., Stein, S., Stone, L.: Post-lockdown abatement of COVID-19 by fast periodic switching. PLOS Computational

Biology **17**(1), 1008604 (2021) <https://doi.org/10.1371/journal.pcbi.1008604>

- [2] Kasis, A., Timotheou, S., Monshizadeh, N., Polycarpou, M.: Optimal intervention strategies to mitigate the COVID-19 pandemic effects. arXiv (2021). <https://doi.org/10.48550/ARXIV.2101.06282>
- [3] Borri, A., Palumbo, P., Papa, F., Possieri, C.: Optimal design of lock-down and reopening policies for early-stage epidemics through SIR-d models. *Annual Reviews in Control* **51**, 511–524 (2021) <https://doi.org/10.1016/j.arcontrol.2020.12.002>
- [4] Tsay, C., Lejarza, F., Stadtherr, M.A., Baldea, M.: Modeling, state estimation, and optimal control for the US COVID-19 outbreak. *Scientific Reports* **10**(1) (2020) <https://doi.org/10.1038/s41598-020-67459-8>
- [5] Morris, D.H., Rossine, F.W., Plotkin, J.B., Levin, S.A.: Optimal, near-optimal, and robust epidemic control. *Communications Physics* **4**(1) (2021) <https://doi.org/10.1038/s42005-021-00570-y>
- [6] Di Lauro, F., Kiss, I.Z., Miller, J.C.: Optimal timing of one-shot interventions for epidemic control. *PLOS Computational Biology* **17**(3), 1008763 (2021) <https://doi.org/10.1371/journal.pcbi.1008763>
- [7] Pates, R., Ferragut, A., Pivo, E., You, P., Paganini, F., Mallada, E.: Respect the unstable: Delays and saturation in contact tracing for disease control. *SIAM Journal on Control and Optimization* **60**(2), 196–220 (2022) <https://doi.org/10.1137/20m1377825>
- [8] Rowthorn, R., Maciejowski, J.: A cost–benefit analysis of the COVID-19 disease. *Oxford Review of Economic Policy* **36**(Supplement\_1), 38–55 (2020) <https://doi.org/10.1093/oxrep/graa030>
- [9] Maciejowski, J., Rowthorn, R., Sheffield, S., Vines, D., Williamson, A.: Mitigation policy for the covid-19 pandemic: Intertemporal optimisation using an seir model. *SSRN Electronic Journal* (2022) <https://doi.org/10.2139/ssrn.4003885>
- [10] Rowthorn, R., Toxvaerd, F.M.O.: The optimal control of infectious diseases via prevention and treatment (2020) <https://doi.org/10.17863/CAM.52481>
- [11] Ferguson, N., Laydon, D., Nedjati Gilani, G., Imai, N., Ainslie, K., Baguelin, M., Bhatia, S., Boonyasiri, A., Cucunuba Perez, Z., Cuomo-Dannenburg, G., Dighe, A., Dorigatti, I., Fu, H., Gaythorpe, K., Green, W., Hamlet, A., Hinsley, W., Okell, L., Van Elsland, S., Thompson, H., Verity, R., Volz, E., Wang, H., Wang, Y., Walker, P., Winskill, P., Whittaker, C., Donnelly, C., Riley, S., Ghani, A.: Report 9: Impact of non-pharmaceutical interventions (npis) to reduce covid19 mortality and healthcare demand (2020) <https://doi.org/10.25561/77482>

- [12] Ferguson, N.M., Cummings, D.A.T., Cauchemez, S., Fraser, C., Riley, S., Meeyai, A., Iamsirithaworn, S., Burke, D.S.: Strategies for containing an emerging influenza pandemic in southeast asia. *Nature* **437**(7056), 209–214 (2005) <https://doi.org/10.1038/nature04017>
- [13] Longini, I.M., Nizam, A., Xu, S., Ungchusak, K., Hanshaoworakul, W., Cummings, D.A.T., Halloran, M.E.: Containing pandemic influenza at the source. *Science* **309**(5737), 1083–1087 (2005) <https://doi.org/10.1126/science.1115717>
- [14] Ferguson, N.M., Cummings, D.A.T., Fraser, C., Cajka, J.C., Cooley, P.C., Burke, D.S.: Strategies for mitigating an influenza pandemic. *Nature* **442**(7101), 448–452 (2006) <https://doi.org/10.1038/nature04795>
- [15] Allen, L.: *An Introduction to Stochastic Processes with Applications to Biology*. Chapman & Hall/CRC, Boca Raton, FL (2011)
- [16] Gardiner, C.W.: *Handbook of Stochastic Methods*, 3. ed. edn. Springer complexity. Springer, Berlin (2004)
- [17] Munsky, B., Khammash, M.: The finite state projection algorithm for the solution of the chemical master equation. *The Journal of Chemical Physics* **124**(4) (2006) <https://doi.org/10.1063/1.2145882>
- [18] Wallinga, J.: Different epidemic curves for severe acute respiratory syndrome reveal similar impacts of control measures. *American Journal of Epidemiology* **160**(6), 509–516 (2004) <https://doi.org/10.1093/aje/kwh255>
- [19] Dietz, K.: The estimation of the basic reproduction number for infectious diseases. *Statistical Methods in Medical Research* **2**(1), 23–41 (1993) <https://doi.org/10.1177/096228029300200103>
- [20] Diekmann, O., Heesterbeek, J.A.P., Metz, J.A.J.: On the definition and the computation of the basic reproduction ratio  $r_0$  in models for infectious diseases in heterogeneous populations. *Journal of Mathematical Biology* **28**(4) (1990) <https://doi.org/10.1007/bf00178324>
- [21] West, R.W., Thompson, J.R.: Models for the simple epidemic. *Mathematical Biosciences* **141**(1), 29–39 (1997) [https://doi.org/10.1016/s0025-5564\(96\)00169-1](https://doi.org/10.1016/s0025-5564(96)00169-1)
- [22] Kermack, W.O., McKendrick, A.G.: A contribution to the mathematical theory of epidemics. *Proceedings of the Royal Society of London. Series A, Containing Papers of a Mathematical and Physical Character* **115**(772), 700–721 (1927) <https://doi.org/10.1098/rspa.1927.0118>
- [23] Blackwell, D.: Memoryless strategies in finite-stage dynamic programming. *The Annals of Mathematical Statistics* **35**(2), 863–865 (1964) <https://doi.org/10.1093/annals/35.2.863>

- [24] Puterman, M.L. (ed.): Markov Decision Processes. John Wiley & Sons, Inc., ??? (1994). <https://doi.org/10.1002/9780470316887>
- [25] Bertsekas, D.: Dynamic Programming and Optimal Control. Athena Scientific, Belmont, Mass (2005)
- [26] Ludkovski, M., Niemi, J.: Optimal dynamic policies for influenza management. *Statistical Communications in Infectious Diseases* **2**(1) (2010) <https://doi.org/10.2202/1948-4690.1020>
- [27] Barnett, M., Buchak, G., Yannelis, C.: Epidemic responses under uncertainty. *Proceedings of the National Academy of Sciences* **120**(2) (2023) <https://doi.org/10.1073/pnas.2208111120>
- [28] UK Health Security Agency: REACT-1 study of coronavirus transmission: February 2022 final results. <https://www.gov.uk/government/publications/react-1-study-of-coronavirus-transmission-february-2022-final-results>
- [29] Metcalf, C.J.E., Morris, D.H., Park, S.W.: Mathematical models to guide pandemic response. *Science* **369**(6502), 368–369 (2020) <https://doi.org/10.1126/science.abd1668>
- [30] Fine, P., Eames, K., Heymann, D.L.: "herd immunity": A rough guide. *Clinical Infectious Diseases* **52**(7), 911–916 (2011) <https://doi.org/10.1093/cid/cir007>
- [31] Fontanet, A., Cauchemez, S.: Covid-19 herd immunity: where are we? *Nature Reviews Immunology* **20**(10), 583–584 (2020) <https://doi.org/10.1038/s41577-020-00451-5>
- [32] Delamater, P.L., Street, E.J., Leslie, T.F., Yang, Y.T., Jacobsen, K.H.: Complexity of the basic reproduction number ( $R_0$ ). *Emerging Infectious Diseases* **25**(1), 1–4 (2019) <https://doi.org/10.3201/eid2501.171901>
- [33] Lin, Q., Zhao, S., Gao, D., Lou, Y., Yang, S., Musa, S.S., Wang, M.H., Cai, Y., Wang, W., Yang, L., He, D.: A conceptual model for the coronavirus disease 2019 (COVID-19) outbreak in wuhan, china with individual reaction and governmental action. *International Journal of Infectious Diseases* **93**, 211–216 (2020) <https://doi.org/10.1016/j.ijid.2020.02.058>
- [34] Flaxman, S., Mishra, S., Gandy, A., Unwin, H., Coupland, H., Mellan, T., Zhu, H., Berah, T., Eaton, J., Perez Guzman, P., Schmit, N., Cilloni, L., Ainslie, K., Baguelin, M., Blake, I., Boonyasiri, A., Boyd, O., Cattarino, L., Ciavarella, C., Cooper, L., Cucunuba Perez, Z., Cuomo-Dannenburg, G., Dighe, A., Djaafara, A., Dorigatti, I., Van Elsland, S., Fitzjohn, R., Fu, H., Gaythorpe, K., Geidelberg,

- L., Grassly, N., Green, W., Hallett, T., Hamlet, A., Hinsley, W., Jeffrey, B., Jorgensen, D., Knock, E., Laydon, D., Nedjati Gilani, G., Nouvellet, P., Parag, K., Siveroni, I., Thompson, H., Verity, R., Volz, E., Walters, C., Wang, H., Wang, Y., Watson, O., Winskill, P., Xi, X., Whittaker, C., Walker, P., Ghani, A., Donnelly, C., Riley, S., Okell, L., Vollmer, M., Ferguson, N., Bhatt, S.: Report 13: Estimating the number of infections and the impact of non-pharmaceutical interventions on covid-19 in 11 european countries (2020) <https://doi.org/10.25561/77731>
- [35] Liu, Y., Gayle, A.A., Wilder-Smith, A., Rocklöv, J.: The reproductive number of COVID-19 is higher compared to SARS coronavirus. *Journal of Travel Medicine* **27**(2) (2020) <https://doi.org/10.1093/jtm/taaa021>
- [36] Korolev, I.: Identification and estimation of the SEIRD epidemic model for COVID-19. *Journal of Econometrics* **220**(1), 63–85 (2021) <https://doi.org/10.1016/j.jeconom.2020.07.038>
- [37] Arroyo-Marioli, F., Bullano, F., Kucinskas, S., Rondón-Moreno, C.: Tracking  $r$  of COVID-19: A new real-time estimation using the kalman filter. *PLOS ONE* **16**(1), 0244474 (2021) <https://doi.org/10.1371/journal.pone.0244474>
- [38] Driessche, P.: Reproduction numbers of infectious disease models. *Infectious Disease Modelling* **2**(3), 288–303 (2017) <https://doi.org/10.1016/j.idm.2017.06.002>
- [39] Biggerstaff, M., Cauchemez, S., Reed, C., Gambhir, M., Finelli, L.: Estimates of the reproduction number for seasonal, pandemic, and zoonotic influenza: a systematic review of the literature. *BMC Infectious Diseases* **14**(1) (2014) <https://doi.org/10.1186/1471-2334-14-480>
- [40] Petersen, E., Koopmans, M., Go, U., Hamer, D.H., Petrosillo, N., Castelli, F., Storgaard, M., Khalili, S.A., Simonsen, L.: Comparing SARS-CoV-2 with SARS-CoV and influenza pandemics. *The Lancet Infectious Diseases* **20**(9), 238–244 (2020) [https://doi.org/10.1016/s1473-3099\(20\)30484-9](https://doi.org/10.1016/s1473-3099(20)30484-9)
- [41] Yamamoto, N., Jiang, B., Wang, H.: Quantifying compliance with COVID-19 mitigation policies in the US: A mathematical modeling study. *Infectious Disease Modelling* **6**, 503–513 (2021) <https://doi.org/10.1016/j.idm.2021.02.004>
- [42] Gillespie, D.T.: Stochastic simulation of chemical kinetics. *Annual Review of Physical Chemistry* **58**(1), 35–55 (2007) <https://doi.org/10.1146/annurev.physchem.58.032806.104637>
- [43] Wu, J.T., Leung, K., Bushman, M., Kishore, N., Niehus, R., Salazar, P.M., Cowling, B.J., Lipsitch, M., Leung, G.M.: Estimating clinical severity of COVID-19 from the transmission dynamics in wuhan, china. *Nature Medicine* **26**(4), 506–510 (2020) <https://doi.org/10.1038/s41591-020-0822-7>

- [44] Jason Oke, C.H.: Global Covid-19 Case Fatality Rates. <https://www.cebm.net/covid-19/global-covid-19-case-fatality-rates/>
- [45] Alvarez, F., Argente, D., Lippi, F.: A simple planning problem for COVID-19 lock-down, testing, and tracing. *American Economic Review: Insights* **3**(3), 367–382 (2021) <https://doi.org/10.1257/aeri.20200201>
- [46] Lauer, S.A., Grantz, K.H., Bi, Q., Jones, F.K., Zheng, Q., Meredith, H.R., Azman, A.S., Reich, N.G., Lessler, J.: The incubation period of coronavirus disease 2019 (COVID-19) from publicly reported confirmed cases: Estimation and application. *Annals of Internal Medicine* **172**(9), 577–582 (2020) <https://doi.org/10.7326/m20-0504>
- [47] Allen, L.J.S.: A primer on stochastic epidemic models: Formulation, numerical simulation, and analysis. *Infectious Disease Modelling* **2**(2), 128–142 (2017) <https://doi.org/10.1016/j.idm.2017.03.001>
- [48] Van Kampen, N.G.: *Stochastic Processes in Physics and Chemistry*. Elsevier LTD, Oxford, ??? (2007)
- [49] Sethi, S.P., Staats, P.W.: Optimal control of some simple deterministic epidemic models. *The Journal of the Operational Research Society* **29**(2), 129 (1978) <https://doi.org/10.2307/3009792>
- [50] Bellman, R.: Dynamic Programming and a new formalism in the calculus of variations. *Proceedings of the National Academy of Sciences* **40**(4), 231–235 (1954) <https://doi.org/10.1073/pnas.40.4.231>
- [51] Gamkrelidze, R.V.: Discovery of the maximum principle. *Journal of Dynamical and Control Systems* **5**(4), 437–451 (1999) <https://doi.org/10.1023/a:1021783020548>
- [52] Liberzon, D.: *Calculus of Variations and Optimal Control Theory a Concise Introduction*, p. 235. Princeton Univ Press, ??? (2012)
- [53] Dixit, A.K.: *Optimization in Economic Theory*, p. 206. Oxford University Press, USA, ??? (1990)
- [54] Team Commands, I.S.: *BOCOP: an open source toolbox for optimal control* (2017)
- [55] Keeling, M.J., Rohani, P.: *Modeling Infectious Diseases in Humans and Animals*, 1st edn. Princeton University Press, Princeton, N.J. (2007)
- [56] Boyd, S., Vandenberghe, L.: *Convex Optimization*, p. 730. Cambridge University Press, ??? (2004)
- [57] Bellman, R.: On the theory of dynamic programming. *Proceedings of the National*



- Academy of Sciences **38**(8), 716–719 (1952) <https://doi.org/10.1073/pnas.38.8.716>
- [58] Christos G. Cassandras, S.L.: Introduction to Discrete Event Systems. Springer, ??? (2007)
- [59] Ferguson, N.: Capturing human behaviour. Nature **446**(7137), 733–733 (2007) <https://doi.org/10.1038/446733a>
- [60] Eames, K.T.D., Keeling, M.J.: Contact tracing and disease control. Proceedings of the Royal Society of London. Series B: Biological Sciences **270**(1533), 2565–2571 (2003) <https://doi.org/10.1098/rspb.2003.2554>

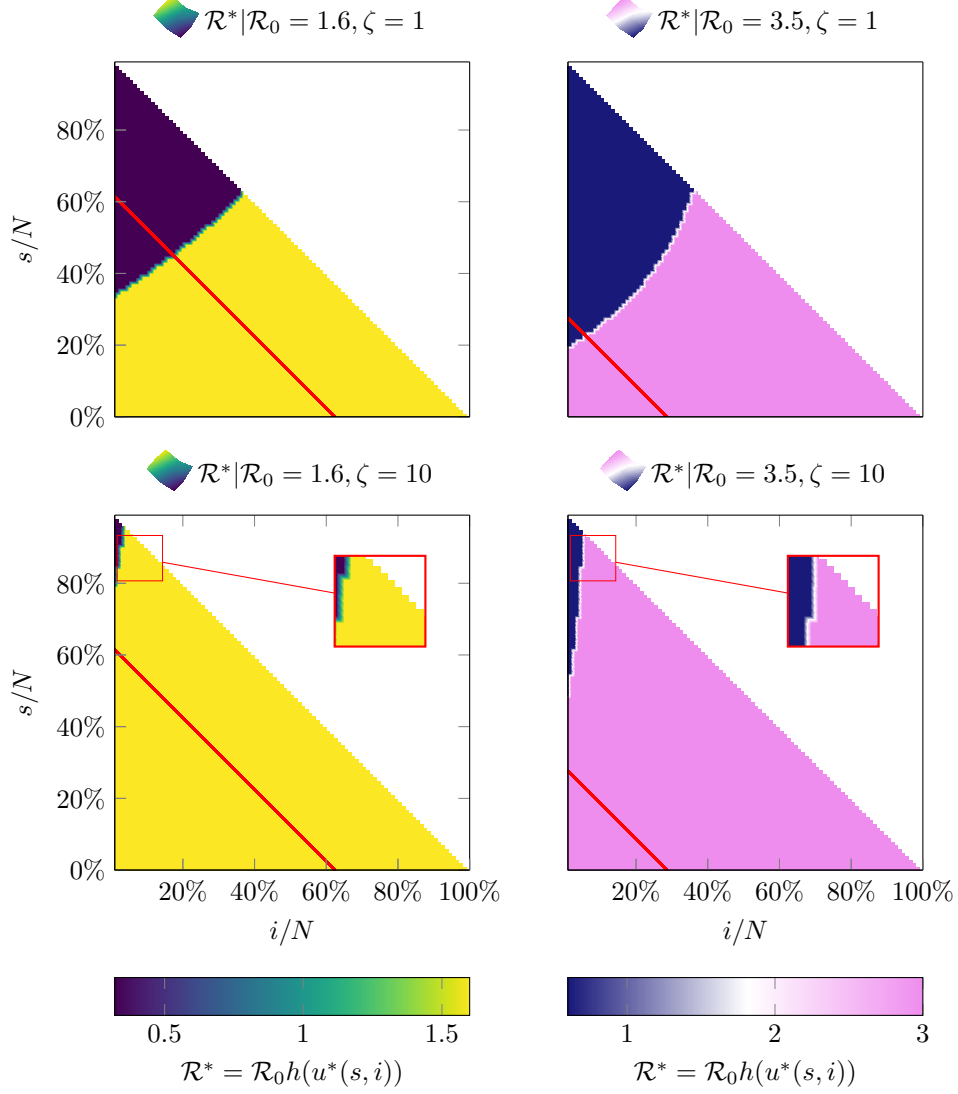

**Fig. S1:** The Figure shows the optimal  $\mathcal{R}^* = \mathcal{R}_0 h(u^*(s/N, i/N))$  in four settings for Problem 1 with  $g_c(i, u) = \zeta i u + i$  corresponding to  $\zeta = \{1, 10\}$  and  $\mathcal{R}_0 = \{1.6, 3.5\}$ . The effective reproduction number  $\mathcal{R}^*$  is constant for low prevalence levels and is non-decreasing for increasing prevalence, *i.e.* the optimal policies are predominantly constant and are non-increasing for increasing prevalence levels. Negative feedback scheme using infection prevalence are therefore not effective for taming the epidemic and there is no incentive to vary interventions. The diagrams display the values of  $\mathcal{R}^*$  in the lower left triangle, *i.e.* the sub diagonals of the graph, and correspond to regimes where recoveries have taken place. That is the values of  $s/N$  and  $i/N$  such that  $s/N + i/N < 1$  and  $r/N > 0$ . The top-left to bottom-right main diagonal of the diagrams corresponds to regimes where  $s/N + i/N = 1$ , *i.e.* regimes where there are no recovered individuals and the SIR and SI model have an exact correspondence. Note that  $H_i$  (—) is a threshold on the recovered levels such that  $s/N + i/N = 1 - H_i$  and is thus shown as a diagonal. For  $\zeta = 1$ , and for prevalence up to approximately 50%, it is optimal to implement interventions also after  $H_i$ . For  $\zeta = 10$  it is optimal to rely upon herd immunity since  $\mathcal{R}^*$  increases to  $\mathcal{R}_0$  before  $H_i$ . The parameters are representative of COVID-19 and flu and are selected using various studies including data from the European Centre of Disease Prevention and Control. In particular, the value of  $\gamma$  is held at  $\gamma = 0.32$  [33]. The values of  $\mathcal{R}_0 = 3.5$  is in line with the values found for COVID-19 in [34–36] and [37] and  $\mathcal{R}_0 = 1.6$  can be associated with Ebola [38] or the 2009 H1N1 flu pandemic [39, 40]. The cost function is selected as  $z(u) = u$ , the intervention to transmission rate function is selected as  $h(u) = 1 - u$ , and the set of implementable interventions is  $\mathcal{U} = \{0, 0.1, \dots, 0.8\}$  for which the effective  $\mathcal{R}$  can be reduced to values below 1.

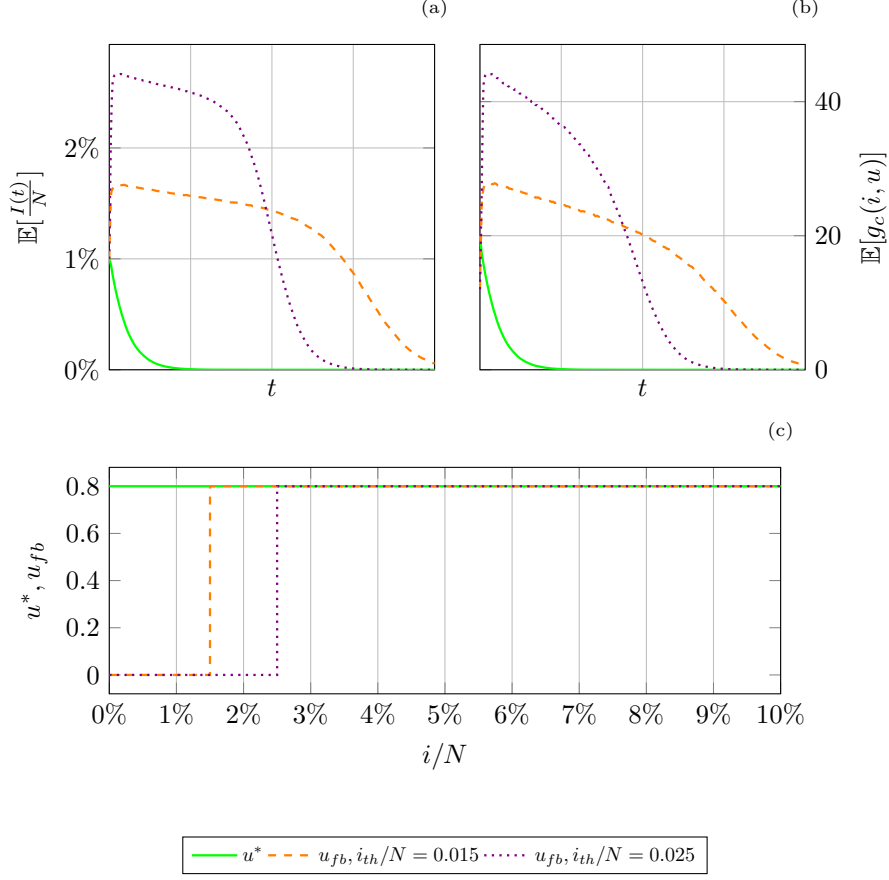

**Fig. S2:** The diagrams in Fig. S2(a), S2(b), display the expected prevalence  $\mathbb{E}[I(t)/N]$  and expected costs  $\mathbb{E}[g_c(i, u)]$  for the SIR epidemic under the optimal (—) and the ad-hoc chosen suboptimal feedback policies (see (22)) (---, ·····) displayed in Fig. S2(c). The infections levels and the costs for the optimal policies decrease rapidly for all the considered cases. The suboptimal policies are associated with high peaks of prevalence and high costs. The optimal policy is the solution of Problem 1 with costs as in (9) for  $\zeta = 12$  and the suboptimal policies shown in Fig. S2(c), make use of interventions at  $i_{th}/N = 0.015$  (---) and  $i_{th}/N = 0.025$  (·····). In Fig. S2(a) and S2(b) we select  $h(u) = (1 - q_{eff}u)$  and the effectiveness of the interventions  $q_{eff} = 0.65$  such that  $\mathcal{R}$  can be lower than 1, *i.e.* the interventions can mitigate the disease transmission and effectively reduce the levels of infection. This value of  $q_{eff}$  is selected close to the upper bound for the COVID-19 pandemic in the United States of America found in [41]. The parameters are  $\gamma = 0.32$ ,  $\mathcal{R}_0 = 3.5$ ,  $I(0)/N = 0.01N$ . The simulations have been performed using the stochastic simulation algorithm [42].

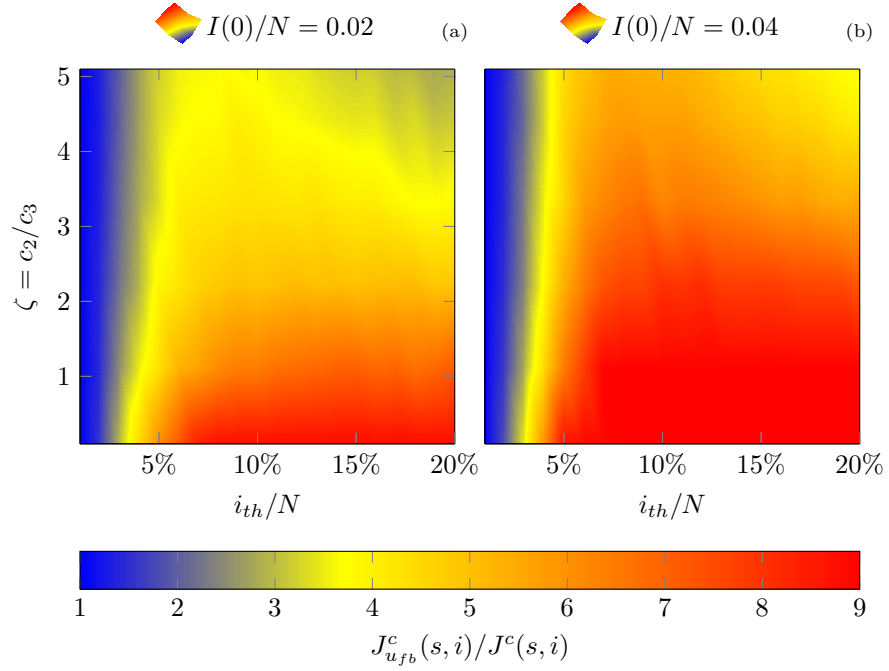

**Fig. S3:** The diagrams show the ratio between the total expected costs  $J_{u_{fb}}^c$  associated with the suboptimal prevalence sensitive feedback policy of the type in (22) over the expected costs  $J_{u_{fb}}^c$  associated with the optimal policies that are not sensitive to prevalence levels for which negative feedback is not effective. The total costs of adopting a negative feedback scheme on the infections is several times higher than for the optimal case. The initial conditions are set to  $I(0)/N = 0.02$  and  $I(0)/N = 0.04$ . The results are shown for  $\gamma = 0.32$ ,  $\mathcal{R}_0 = 3.5$ .

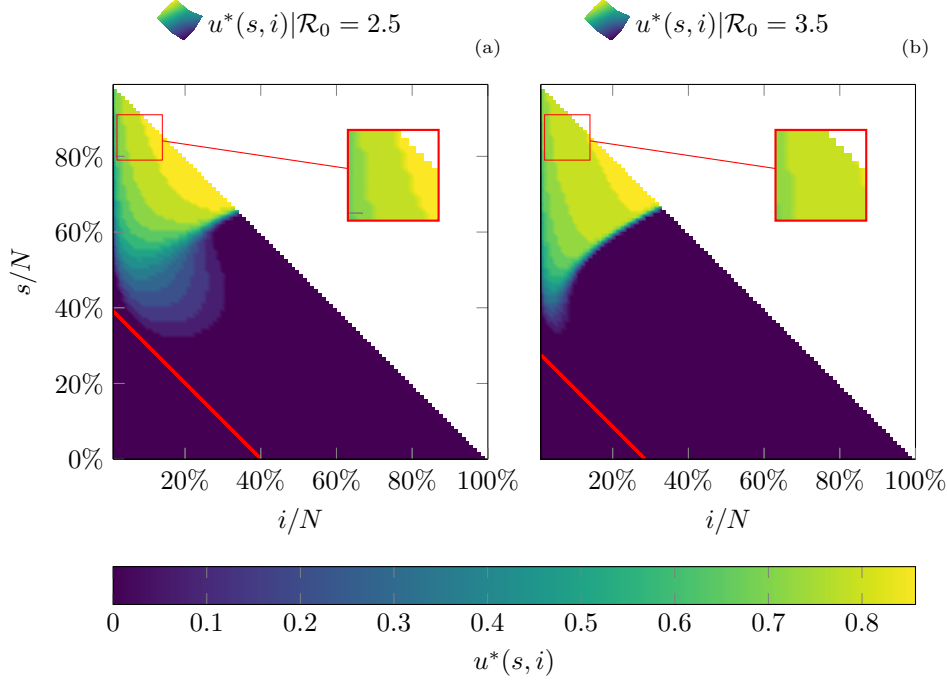

**Fig. S4:** The diagrams display the optimal policies of Problem 1 for the SIR epidemic with costs  $g_c(i, u) = c_3 i + c_4 N u$ ,  $c_2 \approx 0$ , and  $c_4 = 50c_3$ . Fig. S4(a) and S4(b) show that for high values of  $\mathcal{R}_0$  and for  $c_4/c_3 \gg 1$ , the optimal policies gradually implement interventions highlighting that a negative feedback scheme can be optimal for this setting. The optimal policies also change irrespectively of  $H_i$  (—) indicating that depending on the considered  $\mathcal{R}_0$  it may be beneficial to make use of interventions also after this threshold has been reached. We consider  $h(u) = (1 - q_{eff}u)^2$  where  $q_{eff} = 0.65$  [45]. This choice of  $h(u)$  yields rapid decreases of the transmission rate especially for low values of  $u$  and leads to policies that increase and decrease more gradually relative to to linear  $h(u)$ . The parameters have been selected as  $\gamma = 0.32$ , corresponding to an expected recovery of approximately 3.5 days which is inline with the values for COVID-19. The effectiveness of stay at home orders is selected close to the upper bound for the COVID-19 pandemic in the United States of America found in [41] *i.e.*  $q_{eff} = 0.65$  for which the optimal policies can yield  $\mathcal{R} < 1$ .

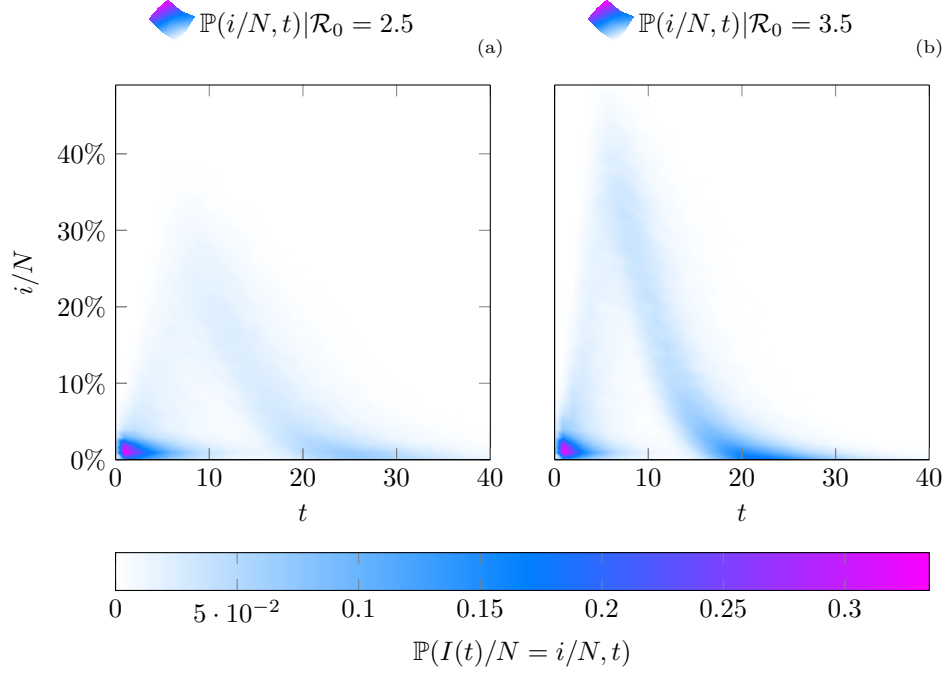

**Fig. S5:** The figures display the probability of prevalence  $\mathbb{P}(i/n, t)$  for the SIR epidemic under the negative feedback optimal policies computed for Fig. S4(a) and S4(b). For all the considered values of  $\mathcal{R}_0$  the optimal policies yield a peak in the infections. Fig. S5(a) displays the probability when using the optimal policy computed for  $\mathcal{R}_0 = 2.5$  in Fig. S4(b) and Fig. S5(b) shows the probability when using the optimal feedback law for  $\mathcal{R}_0 = 3.5$ . The parameters are  $h(u) = (1 - q_{eff}u)^2$ ,  $q_{eff} = 0.65$ , that yields values of  $\mathcal{R}$  lower than 1. We consider  $\gamma = 0.32$  and the initial condition is set to  $I(0)/N = 0.02N$ . The diagrams are obtained by solving the Kolmogorov equation (2) for the SIR epidemic.

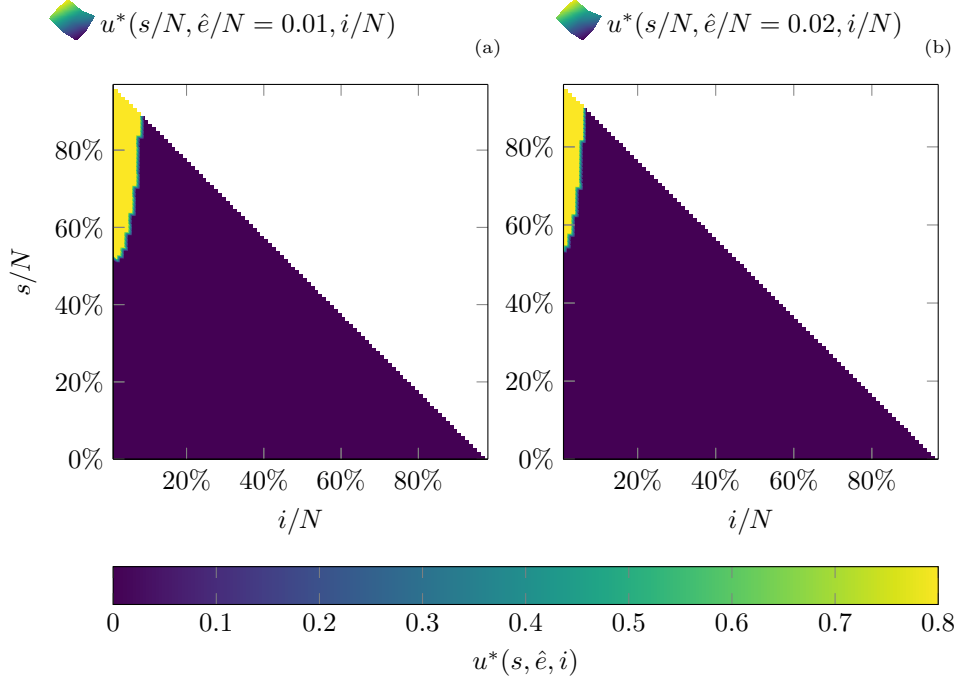

**Fig. S6:** The diagrams display the optimal policies  $u^*(s/N, \hat{e}/N, i/N)$  for the SEIR epidemic at different levels of exposed prevalence  $\hat{e}/N$  *i.e.* Problem 3 with costs functions of the type  $g_c(i, u) = \zeta i u + i$ ,  $\zeta = 15$ . For the considered levels of  $\hat{e}/N$  prevalence negative feedback schemes are not effective to control the epidemic since the optimal policies are non-increasing for increasing infection prevalence and are predominantly constant. It follows that also for this epidemic it is optimal to make use of interventions early and vary them. The optimal policies are shown as a function of the incidence  $s/N$  and infection prevalence  $i/N$ , for a constant levels of exposure  $\hat{e}/N$ , *i.e.* Fig. S6(a) shows the policies for  $\hat{e}/N = 0.02$  in and Fig. S6(b) shows the policies for  $\hat{e}/N = 0.03$ . The policies are computed for  $h(u) = 1 - u$ ,  $\zeta = 15$ ,  $\mathcal{R}_0 = 3.5$  and  $\epsilon = 0.5$ ,  $\gamma = 0.32$ , *i.e.* values that are in line with the parameters for COVID-19. The value of  $\epsilon$  corresponds to an average incubation time of approximately  $\frac{1}{\epsilon} = 2$  days, a value comparable with the incubation time of COVID-19 [46].

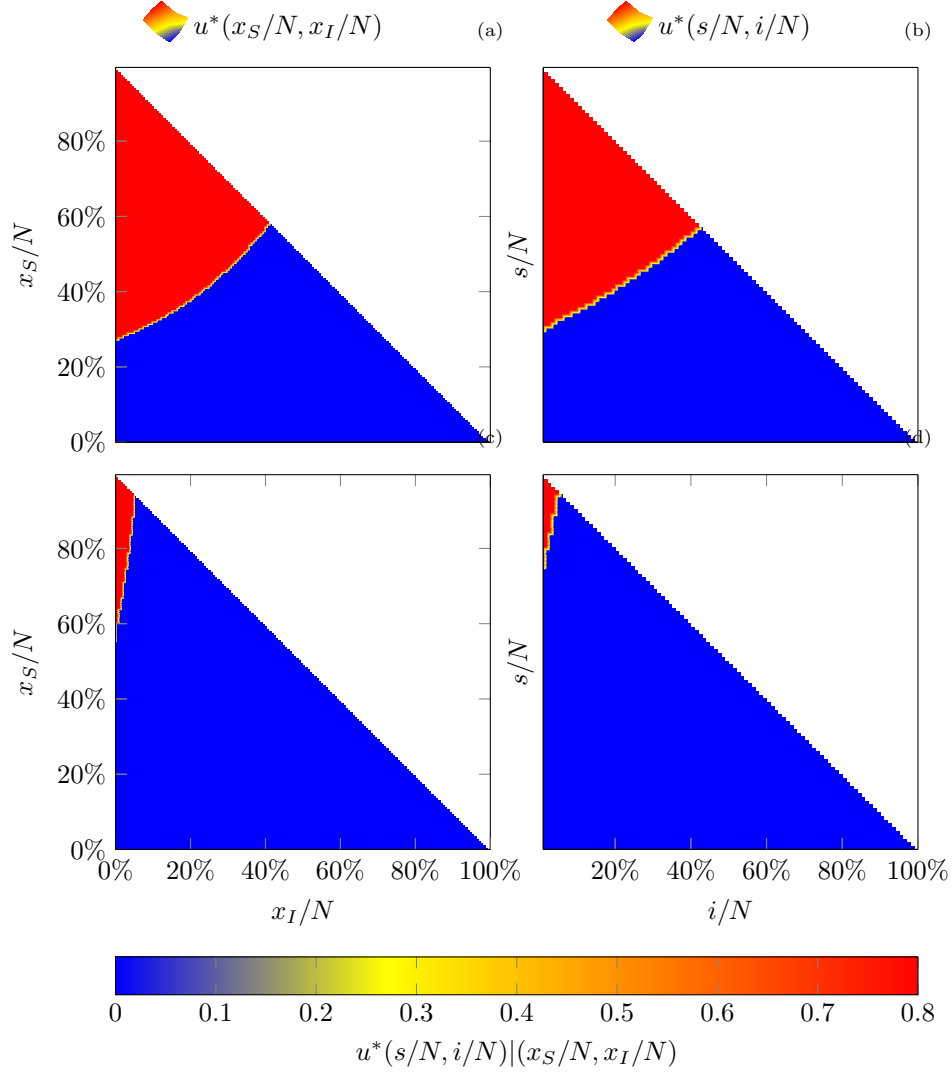

**Fig. S7:** The Figure shows in the left column the optimal policies  $u^*(x_S/N, x_I/N)$  for the deterministic SIR epidemic (Problem 4) and in the right column the policies  $u^*(s/N, i/N)$  for the stochastic Problem 1 with costs  $g_c(i, u) = c_2 i u + c_3 i$  and  $g_{x_I}(x_i, u) = c_2 x_I u + c_3 x_I$ . Without loss of generality we assume  $c_3 = 1$  and consider  $g_c(i, u) = \zeta i u + i$  and  $g_{x_I}(x_i, u) = \zeta x_I u + x_I$ . In all the diagrams the optimal policies are similar, *i.e.* the optimal policies are non-increasing with infection levels and predominantly constant. This highlights that negative feedback is ineffective also for the simplified deterministic setting in the regime considered in this example and validates the results holding for the more complex stochastic formulation. The diagram S7(b) and S7(a) show the optimal policies for the deterministic and stochastic problems the optimal policies with  $\zeta = 1$  *i.e.*  $c_2 = c_3 = 1$ . The diagram S7(d) and S7(c) show the optimal policies for the deterministic and stochastic problems the optimal policies with  $\zeta = 0.1$  *i.e.*  $c_2 = 0.1 c_3$ . The intervention to transmission rate function  $h(u)$  is selected as  $h(u) = 1 - u$  with  $\mathcal{U} = \{0, 0.8\}$ .



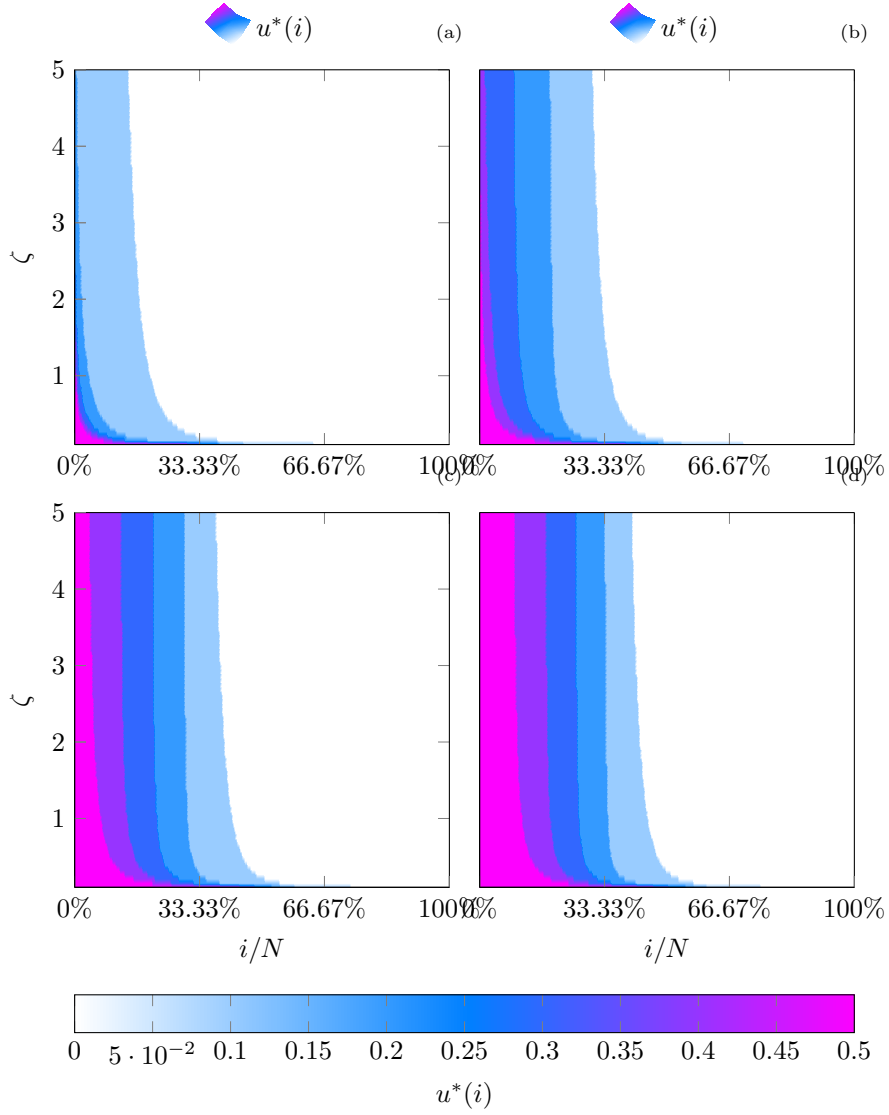

**Fig. S8:** The diagrams show the optimal policies associated with the SI epidemic when an infection event leads to a random number of infected individuals (Problem 10). For all the considered cases the optimal policies are non-increasing for increasing prevalence levels and thus negative feedback schemes are not effective to control the epidemic. The optimal policies are computed for  $\pi_Q \sim \mathcal{B}(p, n)$  for various values of  $p$  and  $n$  and for costs as in (9), *i.e.*  $g_c = c_2 i u + c_3 i$  that without any loss of generality we formulate with  $c_3 = 1$ .  $g_c(i, u) = \zeta i u + i$ . Higher expected values of  $\pi_Q$  lead to more conservative policies, *i.e.* higher values of  $i$  after which the policy will start to reduce interventions. Diagram S8(a) shows the policies for various values of  $\zeta$  when infections events lead to single infected individual *i.e.* Problem 1. Diagram S8(b) shows the policies for increasing values of  $\zeta$  when  $\pi_Q = \mathcal{B}(0.05, 3)$ . Diagram S8(c) shows the policies for increasing values of  $\zeta$  when  $\pi_Q = \mathcal{B}(0.5, 3)$ . Diagram S8(d) show the policies for several values of  $\zeta$  when  $\pi_Q = \mathcal{B}(0.95, 3)$ . In the figure we consider  $h(u) = (1 - u)^2$ ,  $\mathcal{U} = \{0, 0.05, \dots 0.5\}$ .

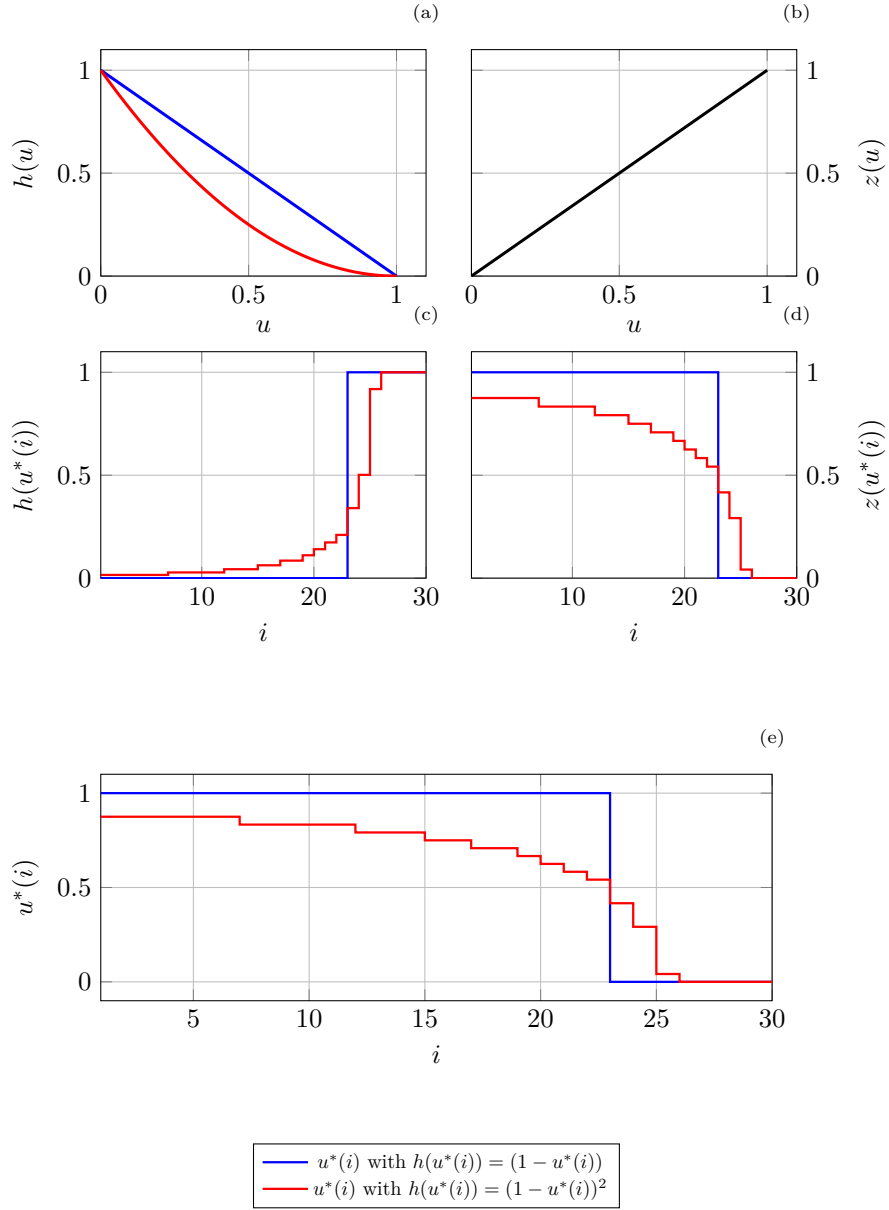

**Fig. B1:** Fig. B1(a) shows  $h(u) = (1 - q_{eff}u)$ ,  $q_{eff} = 1$  (—) and  $h(u) = (1 - q_{eff}u)^2$ ,  $q_{eff} = 1$  (—) as function of the set of interventions  $\mathcal{U} = \{0, 0.04, \dots, 1\}$ . Both functions show that for increasing values of  $u$  the functions  $h(u)$  correspond to reductions of the transmission rate. The diagram B1(b) shows linear interventions costs of the form  $z(u) = u$ . Fig. B1(e) shows the optimal policies  $u^*(i)$  computed explicitly for Problem 2 for costs as in (9) with  $z(u)$  (—) as in Fig. B1(b) and for  $h(u) = (1 - u)$  (—) and  $h(u) = (1 - u)^2$  (—). The optimal policies decrease more gradually for nonlinear mitigation to transmission rate functions. The diagram in Fig. and B1(d) display respectively  $h(u^*(i))$  and  $z(u^*(i))$  as a function of  $i$  under an optimal policy

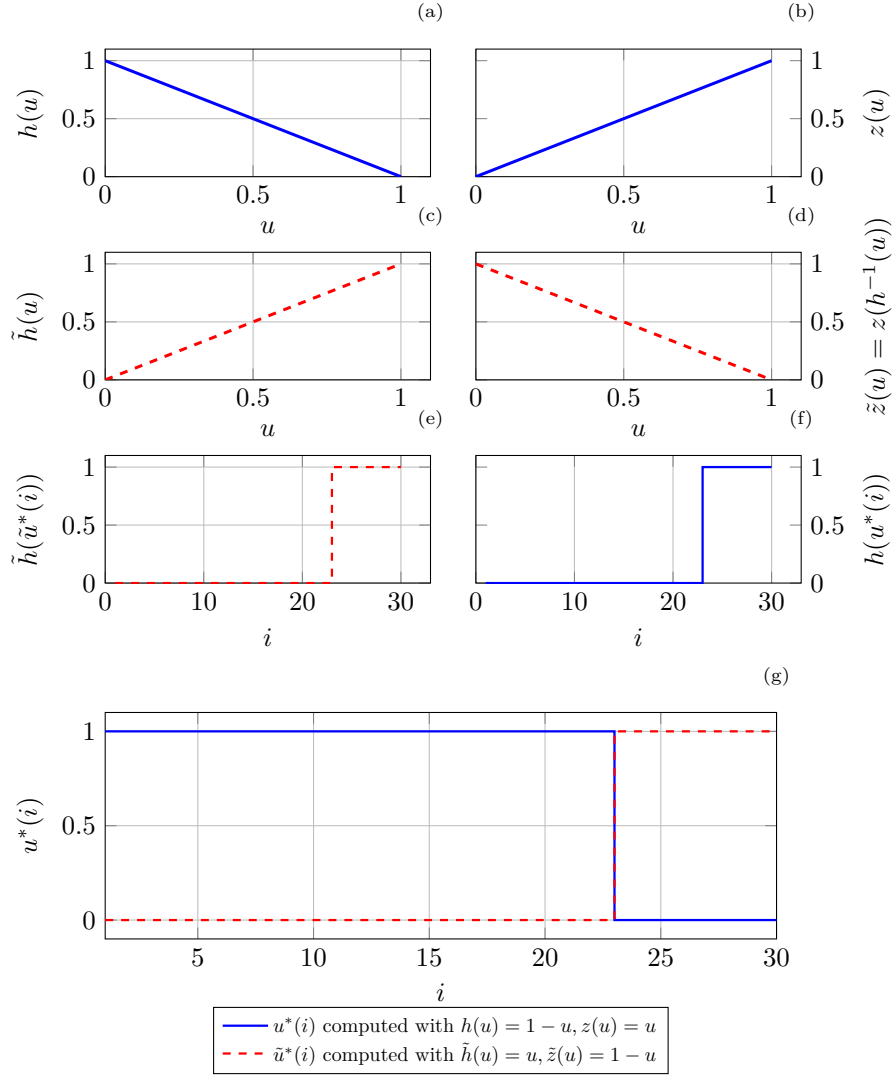

**Fig. B2:** Fig.B2(a) and Fig.B2(b) display  $h(u) = 1 - u$  and  $z(u) = u$  yielding a linear relation between transmission rate and costs. An equivalent formulation is shown in Fig. B2(c) and Fig. B2(d) where low values of  $\tilde{h}(u) = u$  and of the transmission rate yield high costs  $\tilde{z}(u) = 1 - u$ . Optimal policies associated with the two formulations are shown in Fig. B2(g). Fig.B2(e) and Fig.B2(f) show  $\tilde{h}(\tilde{u}^*(i))$  and  $h(u^*(i))$  as a function of the infection levels. Both formulations show equivalent effect upon the transmission is the same thus showing that Assumption 1 is not required for our results.

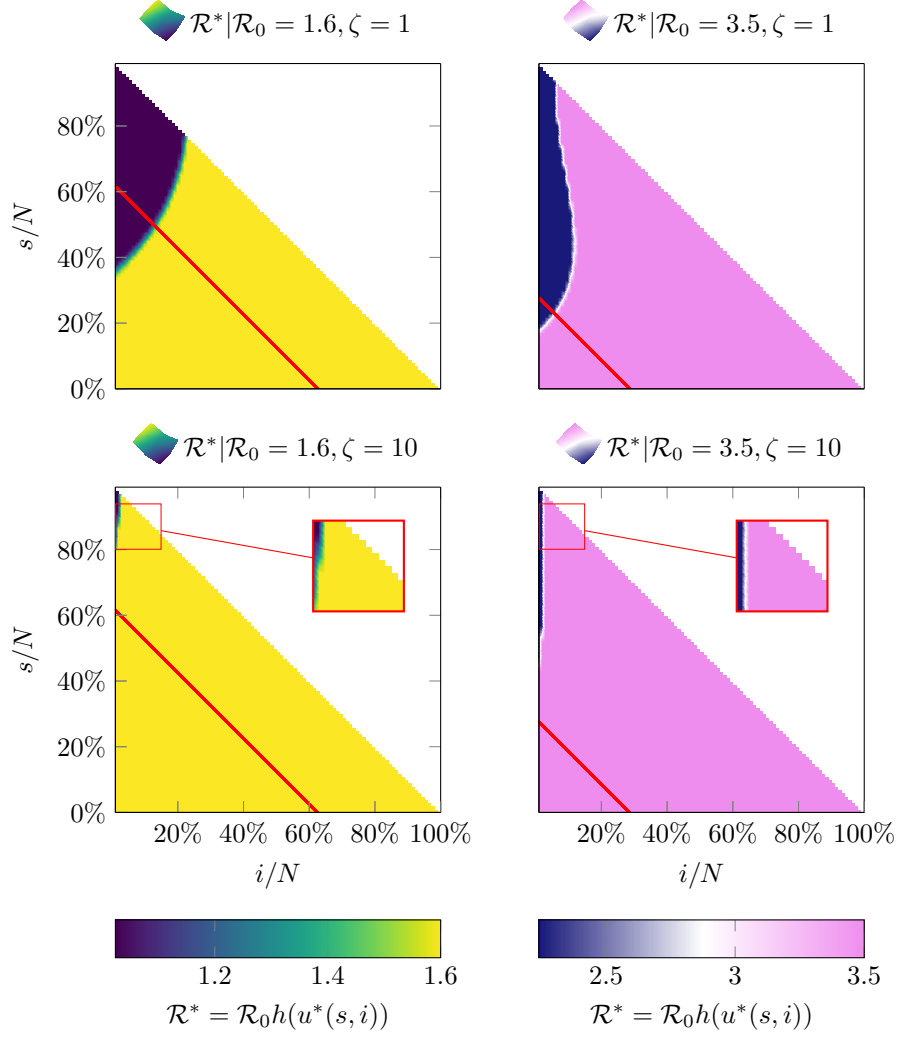

**Fig. B3:** The Figure shows the effective  $\mathcal{R}^*$  for the SIR epidemic in Problem 1 with  $g_c(i, u) = \zeta i u + i$ . The policies are computed for  $h(u) = (1 - 0.5u)^2$ . The optimal policies are non-increasing and are predominantly constant highlighting that negative feedback is not sensitive to infection prevalence. The herd immunity threshold  $H_i$  is plotted (—) for the considered  $\mathcal{R}_0$ . The reproduction number  $\mathcal{R}$  is computed for for  $\mathcal{R}_0 = \{1.6, 3.5\}$  and  $\zeta = \{1, 10\}$ . The parameters are set to  $z(u) = u, \gamma = 0.32, \mathcal{U} = \{0, 0.05, \dots, 0.4\}$ .

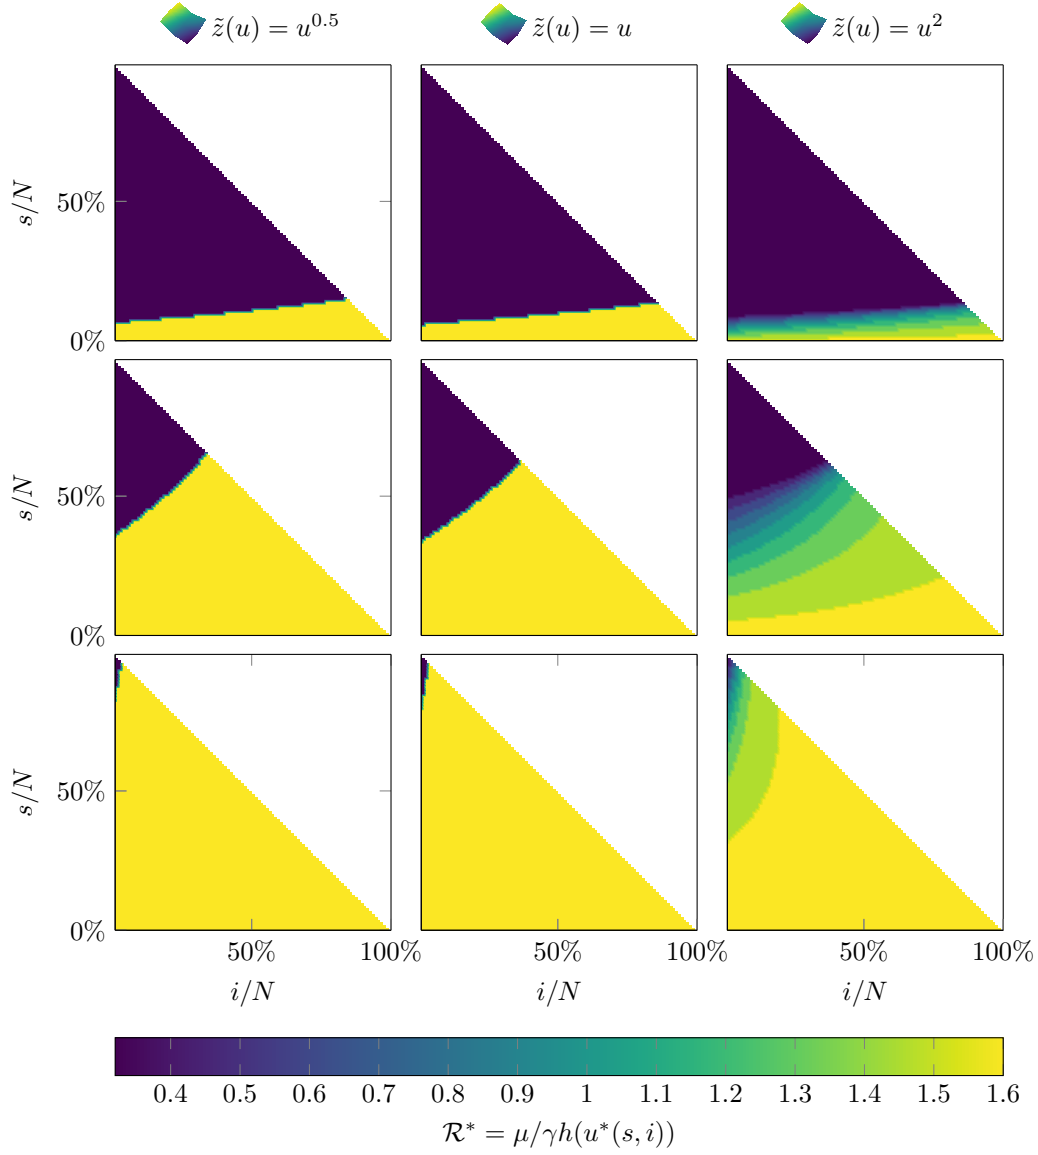

**Fig. B4:** The Figure shows the optimal  $\mathcal{R}^*$  with  $h(u) = 1 - u$  for the SIR epidemic in Problem 1 with  $g_c(i, u) = \zeta i u + i$ . The optimal  $\mathcal{R}$  is non-decreasing and constant for low prevalence. The optimal policies  $u^*$  are non-increasing and predominantly constant for low levels of infection in all the shown settings. In each row, starting from the top row, the diagrams show  $\mathcal{R}^*$  for  $\zeta = c_2/c_3 = 0.1, 1, 10$ . The diagrams illustrate in each column the effective reproduction number  $\mathcal{R}^*$  for  $z(u) = u^{0.5}, u, u^2$ , respectively. The parameters are set to  $\gamma = 0.32, \mathcal{R}_0 = \mu/\gamma = 1.6, h(u) = 1 - u, \mathcal{U} = \{0, 0.1, \dots, 0.8\}$ .

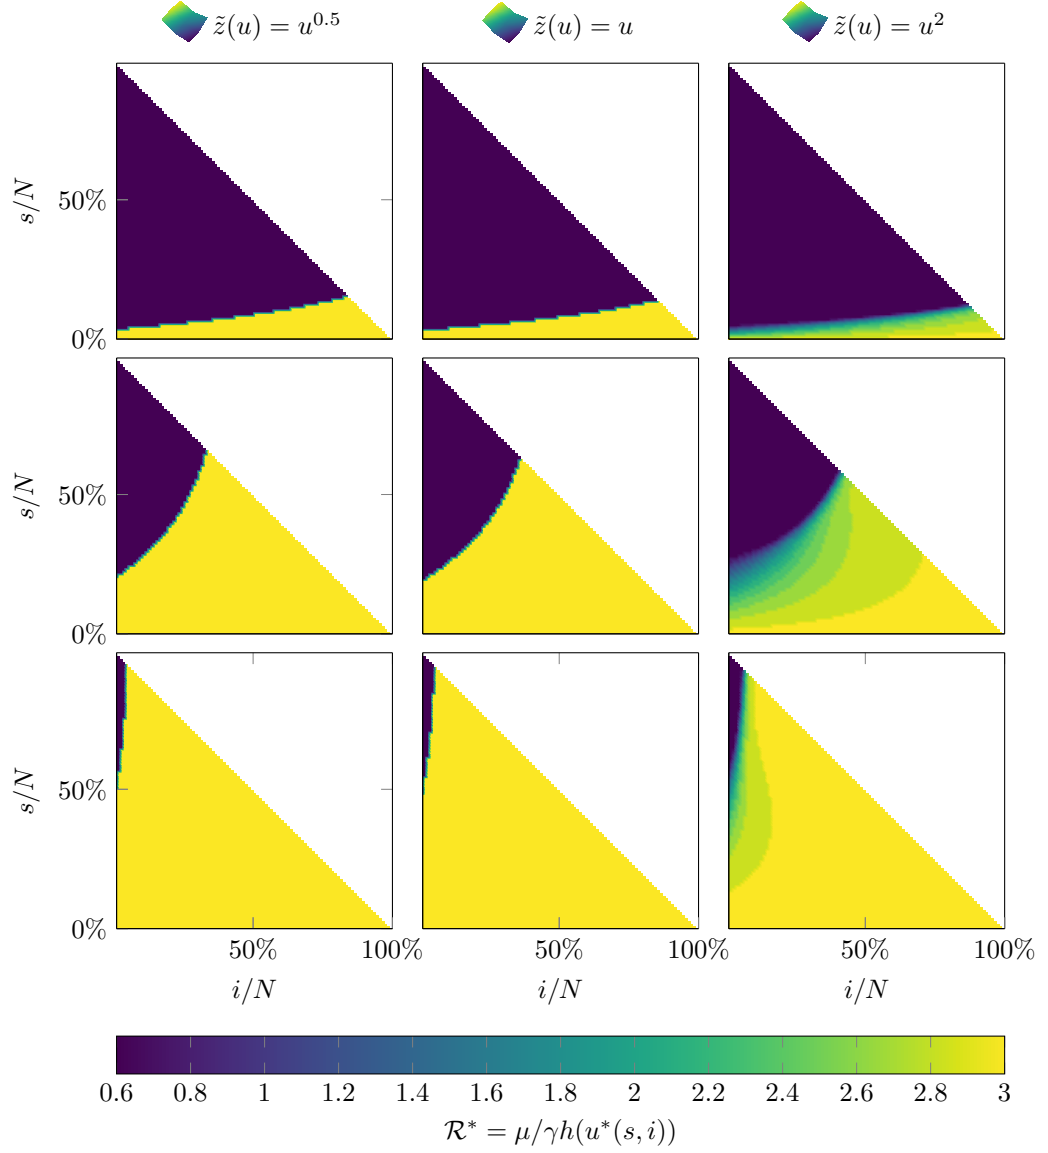

**Fig. B5:** The Figure shows the optimal  $\mathcal{R}^* = \mathcal{R}_0 h(u^*(s, i))$ ,  $h(u) = 1 - u$  for the SIR epidemic in Problem 1 with  $g_c(i, u) = \zeta i u + i$ . The diagrams are analogous to Fig. B4 but with  $\mathcal{R}_0 = 3.5$  a value inline for COVID-19. The optimal  $\mathcal{R}$  is non-decreasing and constant for low levels of infection. The optimal policies are thus non-increasing and predominantly constant for low levels of infection in all the shown settings. In each row, starting from the top row, the diagrams show  $\mathcal{R}^*$  for  $\zeta = c_2/c_3 = 0.1, 1, 10$ . The diagrams illustrate in each column the effective reproduction number  $\mathcal{R}^*$  for  $z(u) = u^{0.5}, u, u^2$ . The parameters are set to  $\gamma = 0.32$ ,  $\mathcal{R}_0 = \mu/\gamma = 3.5$ ,  $h(u) = 1 - u$ ,  $\mathcal{U} = \{0, 0.1, \dots, 0.8\}$ .

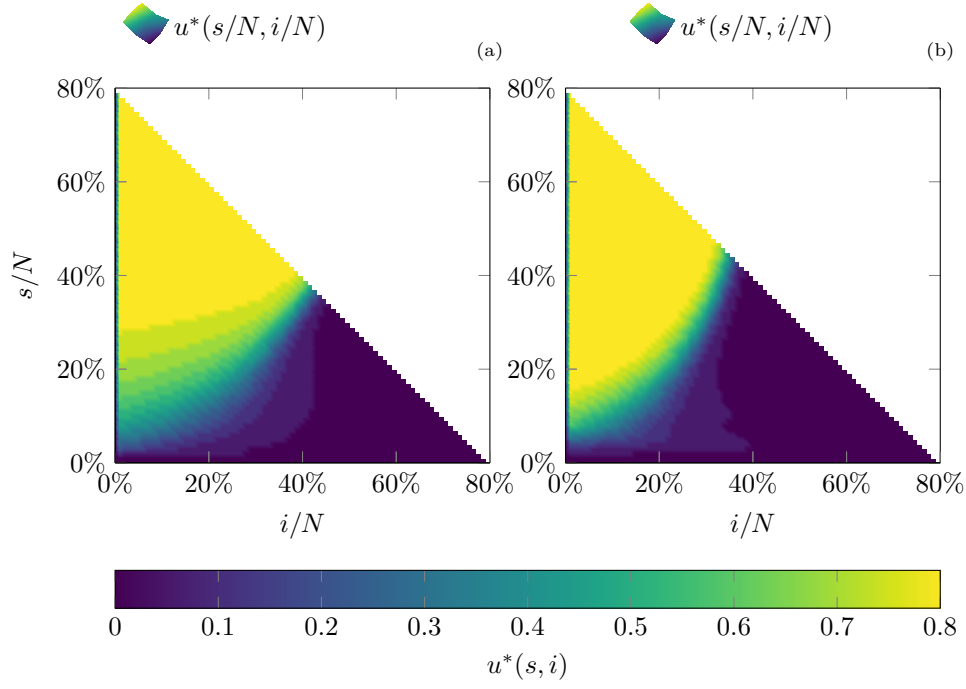

**Fig. B6:** Fig.S6(a) and fig.S6(b) display the optimal policies (Problem 5) with  $g_c(i, u) = \zeta i u + i$  for the SIR epidemic for  $\pi_Q \sim \mathcal{U}(1, 3)$  and  $\pi_Q \sim \mathcal{U}(1, 8)$  respectively. The figures show that also in this setting negative feedback schemes on the infections are not effective to mitigate the epidemic and higher values of  $\mathbb{E}_{\pi_Q}$  are associated with more conservative optimal policies *i.e.* policies with interventions held in place for larger ranges of infected individuals.

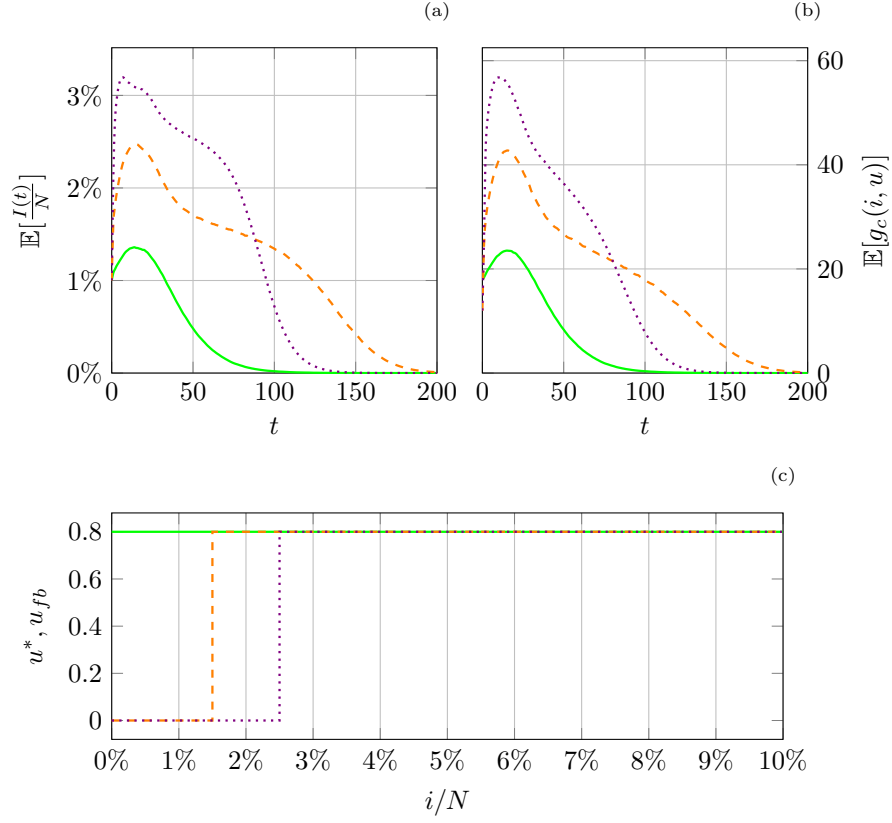

**Fig. B7:** The diagrams B7(a) and B7(b) show the expected infection levels and the associated costs for  $h(u) = (1 - 0.5u)$  when the interventions cannot reduce  $\mathcal{R}$  to values less than 1. In this regimes the infections peaks are much higher when compared to Fig. S2(a) and Fig. S2(b) where  $h(u) = (1 - 0.65u)$  and the interventions can reduce  $\mathcal{R} < 1$ . The parameters are  $\gamma = 0.32, \mathcal{R}_0 = 3.5, I(0)/N = 0.01N$ . The simulations have been performed using the stochastic simulation algorithm [42].



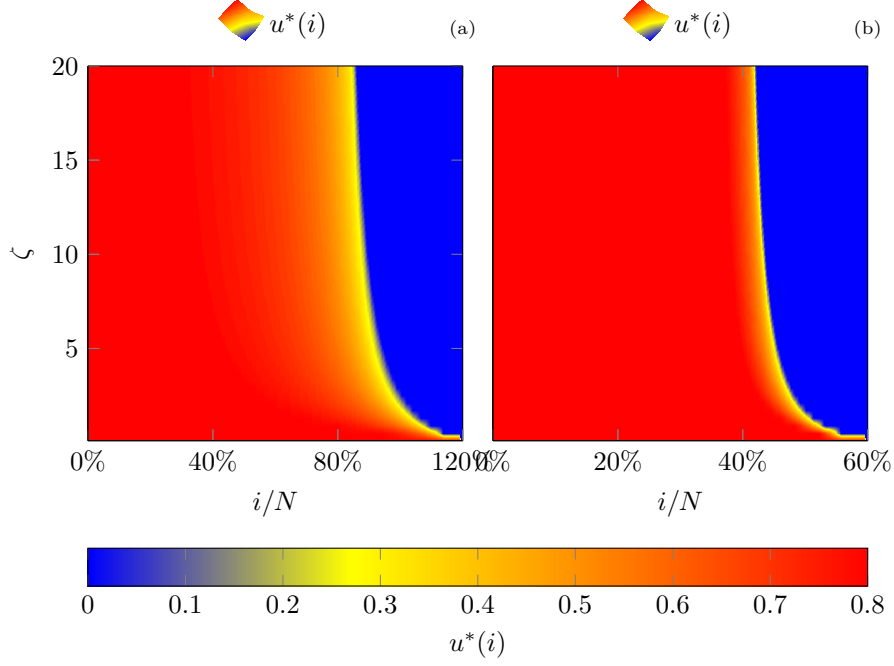

**Fig. B8:** Diagram B8(a) and diagram B8(b) display the optimal policies  $u^*(i)$  of Problem 2 with  $g_c(i, u) = \zeta i u + i$ . The optimal policies are non-increasing for increasing levels of prevalence irrespectively of  $\zeta$ . The policies are also predominantly constant for low levels of infection prevalence highlighting that a prevalence sensitive feedback policies are not effective. The diagram B8(a) shows the policies for  $h(u) = (1 - u)^2$  and the diagram B8(b) shows the policies for  $h(u) = (1 - 0.65u)^2$ . The diagram in Fig. B8(b), associated with a lower effectiveness of the interventions, displays more conservative policies, *i.e.* policies that decrease at lower values of prevalence with respect to Fig. B8(a). The parameters are  $\gamma = 0.32$ ,  $\mathcal{R}_0 = 3.5$ , and the set  $\mathcal{U}$  is selected as  $\mathcal{U} = \{0, 0.05, 0.10, \dots, 0.8\}$ .

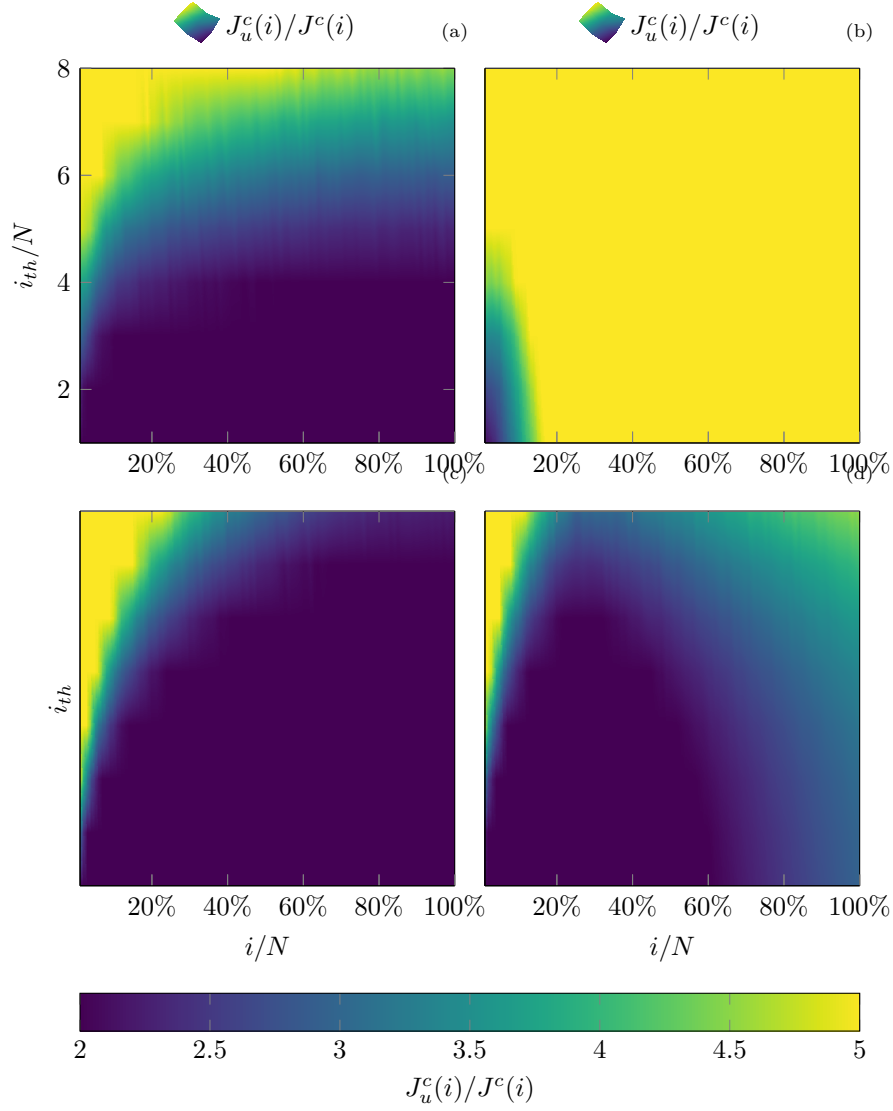

**Fig. B9:** The figure shows for cost functions of the form in (9) the ratio of the total expected costs of the suboptimal negative feedback strategy (22), *i.e.*  $J_{u_{fb}}^c$  defined in (13), over the optimal costs  $J^c(i)$  defined in (12). For all the considered cost parameter configurations negative feedback strategies are several times more expensive over using constant interventions at the onset of the epidemic. The diagrams B9(a) and B9(b) show the ratio of costs as in (9)  $g(i, u) = c_2 i u + c_3 i = \zeta i u + i$ , for  $\zeta = 4$  and for  $\zeta = 6$  respectively. Diagrams B9(a) and B9(a) display the ratio of costs for  $\zeta = 1$  and for  $\zeta = 50$ , respectively. The considered configuration is for  $h(u) = (1 - u)$ ,  $\mathcal{U} = \{0, 0.8\}$ ,  $\mathcal{R}_0 = 2$ ,  $\gamma = 0.32$ .

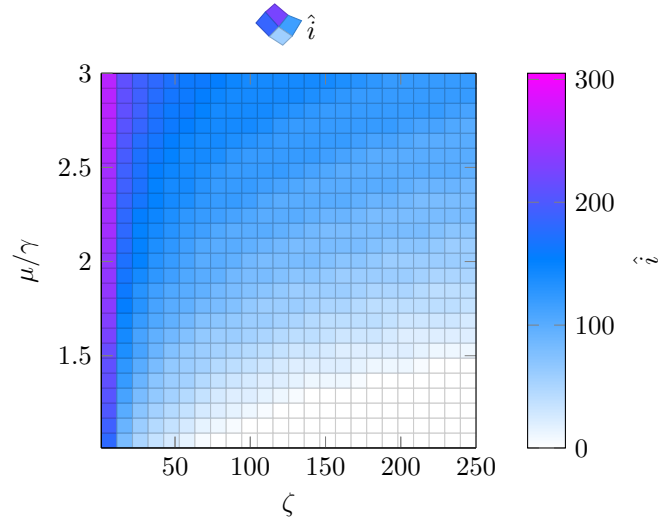

**Fig. B10:** The figure shows for several values of  $\zeta$  and  $\mathcal{R}_0 = \mu/\gamma$  the threshold  $\hat{i}$  at which we have observed the optimal policies decrease to 0 with costs as in (9), i.e.  $g_c(i, u) = \zeta i u + i$ . We consider  $h(u) = (1 - u)$  and the set  $\mathcal{U}$  is selected as  $\mathcal{U} = \{0, 0.05, 0.1, \dots, 0.5\}$ .

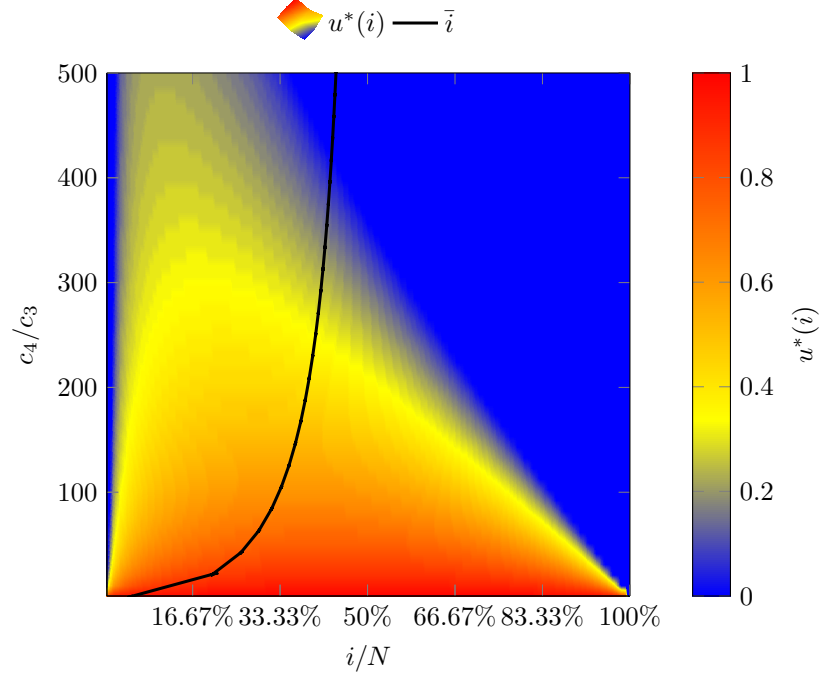

**Fig. B11:** The figure shows the optimal policies  $u^*(i)$  for a cost function of the form in (11), *i.e.*  $g_c(i, u) = c_2 i u + c_3 i + c_4 N u = c_2 i u + c_3 i + c_4 N u$  where  $c_1 = 0, c_2 = 0.01, c_3 = 1$  and for increasing values of  $c_4$ . (—) shows the value of  $\bar{i}$  from (18) for increasing  $c_4$ . The figure shows that for low values of  $c_4$  negative feedback scheme is not effective to tame the epidemic as the policies are non-increasing for increasing levels of infection. The results verify Proposition 2, as the policies are non-increasing  $\forall i \geq \bar{i}$ , *i.e.* on the right hand side of (—). A negative feedback scheme on the infection can be however beneficial for large values of  $c_4$  on the left hand of (—). The parameters are  $\mathcal{R}_0 = 2$   $h(u) = (1 - u)^2$  and the set  $\mathcal{U} = \{0, 0.05, 0.1, \dots, 1\}$ .
